# Supplementary material for: Reentrant phenomenon in the exactly solvable mixed spin-1/2 and spin-1 Ising-Heisenberg model on diamond-like decorated planar lattices
Source: arXiv:0909.4191 source file (2009-09-23)
Supplement: Supplementary file 2 [file caption.pdf]

# Typesetting captions with the caption package\*

Axel Sommerfeldt  
caption@sommerfee.de

2007/04/09

## Abstract

The caption package offers customization of captions in floating environments such `figure` and `table` and cooperates with many other packages.<sup>1</sup>

## Contents

|          |                                                 |           |
|----------|-------------------------------------------------|-----------|
| <b>1</b> | <b>Introduction</b>                             | <b>2</b>  |
| <b>2</b> | <b>Using the package</b>                        | <b>3</b>  |
| <b>3</b> | <b>Options</b>                                  | <b>3</b>  |
| 3.1      | Formatting . . . . .                            | 3         |
| 3.2      | Justification . . . . .                         | 6         |
| 3.3      | Fonts . . . . .                                 | 8         |
| 3.4      | Margins and further paragraph options . . . . . | 9         |
| 3.5      | Styles . . . . .                                | 10        |
| 3.6      | Skips . . . . .                                 | 11        |
| <b>4</b> | <b>Useful stuff</b>                             | <b>12</b> |
| <b>5</b> | <b>Do it yourself!</b>                          | <b>15</b> |
| 5.1      | Further Examples . . . . .                      | 17        |
| <b>6</b> | <b>Using non-standard document classes</b>      | <b>19</b> |

---

\*This package has version number v3.0q, last revised 2007/04/16.

<sup>1</sup>A complete re-work of the user interface done with Steven D. Cochran and Frank Mittelbach has lead to this new enhanced version 3.0.

|           |                                            |           |
|-----------|--------------------------------------------|-----------|
| <b>7</b>  | <b>Compatibility to other packages</b>     | <b>19</b> |
| 7.1       | The float package . . . . .                | 20        |
| 7.2       | The listings package . . . . .             | 21        |
| 7.3       | The longtable package . . . . .            | 21        |
| 7.4       | The rotating package . . . . .             | 21        |
| 7.5       | The sidecap package . . . . .              | 22        |
| 7.6       | The supertabular package . . . . .         | 22        |
| 7.7       | Known incompatibilities . . . . .          | 22        |
| <b>8</b>  | <b>Compatibility to older versions</b>     | <b>22</b> |
| 8.1       | The caption package version 1.x . . . . .  | 22        |
| 8.2       | The caption2 package version 2.x . . . . . | 24        |
| <b>9</b>  | <b>Further reading</b>                     | <b>26</b> |
| <b>10</b> | <b>Thanks</b>                              | <b>26</b> |
| <b>11</b> | <b>The Implementation</b>                  | <b>27</b> |
| 11.1      | Kernel . . . . .                           | 27        |
| 11.2      | Main package . . . . .                     | 46        |

# 1 Introduction

Within the standard L<sup>A</sup>T<sub>E</sub>X classes captions haven't received the attention they deserve. Simply typeset as an ordinary paragraph there is no remarkable visual difference from the rest of the text, like here:

Figure 1: White sand beaches. The pink smoothness of the conch shell. A sea abundant with possibilities. Duty-free shops filled with Europe's finest gifts and perfumes. Play your favorite game of golf amidst the tropical greens on one of the many championship courses.

There should be possibilities to change this; for example, it would be nice if you could make the text of the caption a little bit smaller as the normal text, add an extra margin, typeset the caption label with the same font family and shape as your headings etc. Just like this one:

**Figure 2** – White sand beaches. The pink smoothness of the conch shell. A sea abundant with possibilities. Duty-free shops filled with Europe's finest gifts and perfumes. Play your favorite game of golf amidst the tropical greens on one of the many championship courses.

You can do this easily with this package as there are many ready-to-use caption formatting options, but you are free to define your very own stuff, too.

## 2 Using the package

`\usepackage` Insert

```
\usepackage[<options>]{caption}[2007/04/16]
```

into the preamble of your document, i.e. the part of your document between `\documentclass` and `\begin{document}`. The options control how your captions will look like; e.g.,

```
\usepackage[margin=10pt,font=small,labelfont=bf]{caption}
```

would result in captions looking like the second one in the introduction.

`\captionsetup` For a later change of options the caption package provides the command

```
\captionsetup[<float type>]{<options>}
```

So

```
\usepackage[margin=10pt,font=small,labelfont=bf]{caption}
```

and

```
\usepackage{caption}  
\captionsetup{margin=10pt,font=small,labelfont=bf}
```

are equal in their results.

It's good to know that `\captionsetup` has an effect on the current environment only. So if you want to change some settings for the current figure or table only, just place the `\captionsetup` command inside the figure or table right before the `\caption` command. For example

```
\begin{figure}  
...  
\captionsetup{singlelinecheck=off}  
\caption{...}  
\end{figure}
```

switches the single-line-check off, but only for this figure so all the other captions remain untouched.

(For a description of the optional parameter *<float type>* see section 4: “Useful stuff”.)

## 3 Options

### 3.1 Formatting

`format=` A figure or table caption mainly consists of three parts: the caption label, which says if

this object is a ‘Figure’ or ‘Table’ and what number is associated with it, the caption text itself, which is normally a short description of contents, and the caption separator which separates the text from the label.

The *caption format* determines how this information will be presented; it is specified with the option

```
format=(format name) ,
```

having the name of the caption format as its argument.

There are two standard caption formats:

|                          |       |                                                                                                                                                                 |
|--------------------------|-------|-----------------------------------------------------------------------------------------------------------------------------------------------------------------|
| New description<br>v3.0h | plain | Typesets the captions as a normal paragraph. (This is the default behaviour, it is adapted from the standard L <sup>A</sup> T <sub>E</sub> X document classes.) |
|                          | hang  | Indents the caption text, so it will ‘hang’ under the first line of the text.                                                                                   |
|                          | ...   | Own formats can be defined using <code>\DeclareCaptionFormat</code> . (See section 5: “ <i>Do it yourself</i> ”)                                                |

An example: Specifying the option

```
format=hang
```

yields captions like this:

Figure 3: White sand beaches. The pink smoothness of the conch shell. A sea abundant with possibilities. Duty-free shops filled with Europe’s finest gifts and perfumes. Play your favorite game of golf amidst the tropical greens on one of the many championship courses.

`indentation=` For both formats (`plain` and `hang`) you can setup an extra indentation starting at the second line of the caption. You do this with the option

```
indentation=(amount).
```

Two examples:

```
format=plain,indentation=.5cm
```

Figure 4: White sand beaches. The pink smoothness of the conch shell. A sea abundant with possibilities. Duty-free shops filled with Europe’s finest gifts and perfumes. Play your favorite game of golf amidst the tropical greens on one of the many championship courses.

```
format=hang,indentation=-0.5cm
```

Figure 5: White sand beaches. The pink smoothness of the conch shell. A sea abundant with possibilities. Duty-free shops filled with Europe’s finest gifts and perfumes. Play your favorite game of golf amidst the tropical greens on one of the many championship courses.

`labelformat=` With the option

`labelformat=⟨label format name⟩`

New description v3.0e you specify how the caption label will be typeset. There are four standard caption label formats:

|                      |                                                                                                                                                                                |
|----------------------|--------------------------------------------------------------------------------------------------------------------------------------------------------------------------------|
| <code>default</code> | The caption label will be typeset as specified by the document class, usually this means the name and the number (like <code>simple</code> ). (This is the default behaviour.) |
| <code>empty</code>   | The caption label will be empty. (This option makes sense when used together with other options like <code>labelsep=none</code> .)                                             |
| <code>simple</code>  | The caption label will be typeset as a name and a number.                                                                                                                      |
| <code>parens</code>  | The number of the caption label will be typeset in parentheses.                                                                                                                |
| <code>...</code>     | Own label formats can be defined using <code>\DeclareCaptionLabelFormat</code> . (See section 5: “ <i>Do it yourself</i> ”)                                                    |

An example: Using the options

`labelformat=parens, labelsep=quad`

gives captions like this one:

Figure (6) White sand beaches. The pink smoothness of the conch shell. A sea abundant with possibilities. Duty-free shops filled with Europe’s finest gifts and perfumes. Play your favorite game of golf amidst the tropical greens on one of the many championship courses.

`labelsep=` With the option

`labelsep=⟨label separator name⟩`

you specify what caption separator will be used. You can choose one of the following:

|                      |                                                                                                                                      |
|----------------------|--------------------------------------------------------------------------------------------------------------------------------------|
| <code>none</code>    | There is no caption separator. (This option makes sense when used together with other options like <code>labelformat=empty</code> .) |
| <code>colon</code>   | The caption label and text will be separated by a colon and a space. (This is the default one.)                                      |
| <code>period</code>  | The caption label and text will be separated by a period and a space.                                                                |
| <code>space</code>   | The caption label and text will be separated by a single space.                                                                      |
| <code>quad</code>    | The caption label and text will be separated by a <code>\quad</code> .                                                               |
| <code>newline</code> | The caption label and text will be separated by a line break ( <code>\</code> ).                                                     |

New feature v3.0h    `endash`            The caption label and text will be separated by an en-dash, surrounded by spaces ( `--` ).

...                    Own separators can be defined using `\DeclareCaptionLabelSeparator`. (See section 5: “*Do it yourself*”)

Three examples:

```
labelsep=period
```

Figure 7. White sand beaches. The pink smoothness of the conch shell. A sea abundant with possibilities. Duty-free shops filled with Europe’s finest gifts and perfumes. Play your favorite game of golf amidst the tropical greens on one of the many championship courses.

```
labelsep=newline,singlelinecheck=false
```

Figure 8  
White sand beaches. The pink smoothness of the conch shell. A sea abundant with possibilities. Duty-free shops filled with Europe’s finest gifts and perfumes. Play your favorite game of golf amidst the tropical greens on one of the many championship courses.

```
labelsep=endash
```

Figure 9 – White sand beaches. The pink smoothness of the conch shell. A sea abundant with possibilities. Duty-free shops filled with Europe’s finest gifts and perfumes. Play your favorite game of golf amidst the tropical greens on one of the many championship courses.

### 3.2 Justification

`justification=` As addition to the caption format you could also specify a *caption justification*; it is specified with the option

```
justification=(justification name) .
```

You can choose one of the following:

- `justified`        Typesets the caption as a normal paragraph. (This is the default.)
- `centering`        Each line of the caption will be centered.
- `centerlast`        The last line of each paragraph of the caption text will be centered.
- `centerfirst`        Only the first line of the caption will be centered.
- `raggedright`        Each line of the caption will be moved to the left margin.

`RaggedRight` Each line of the caption will be moved to the left margin, too. But this time the command `\RaggedRight` of the `ragged2e` package will be used to achieve this. The main difference is that the word breaking algorithm of  $\TeX$  will work inside captions.

`raggedleft` Each line of the caption will be moved to the right margin.

... Own justifications can be defined using `\DeclareCaptionJustification`. (See section 5: “*Do it yourself*”)

Three examples:

```
justification=centerlast
```

Figure 10: White sand beaches. The pink smoothness of the conch shell. A sea abundant with possibilities. Duty-free shops filled with Europe’s finest gifts and perfumes. Play your favorite game of golf amidst the tropical greens on one of the many championship courses.

```
format=hang, justification=raggedright
```

Figure 11: White sand beaches. The pink smoothness of the conch shell. A sea abundant with possibilities. Duty-free shops filled with Europe’s finest gifts and perfumes. Play your favorite game of golf amidst the tropical greens on one of the many championship courses.

```
labelsep=newline, justification=centering
```

Figure 12

White sand beaches. The pink smoothness of the conch shell. A sea abundant with possibilities. Duty-free shops filled with Europe’s finest gifts and perfumes. Play your favorite game of golf amidst the tropical greens on one of the many championship courses.

`singlelinecheck=` The standard  $\LaTeX$  document classes (`article`, `report`, and `book`) automatically center a caption if it fits in one single line:

Figure 13: A short caption.

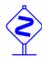

The caption package adapts this behaviour and therefore usually ignores the justification you have set with `justification=` in such case. But you can switch this special treatment of such short captions off with the option

```
singlelinecheck=(bool) .
```

Using `false`, `no`, `off` or `0` for `(bool)` switches the extra centering off:

```
singlelinecheck=false
```

Doing so the above short caption would look like

Figure 13: A short caption.

You switch the extra centering on again by using `true`, `yes`, `on` or `1` for *bool*. (The default is `on`.)

### 3.3 Fonts

`font=` There are three font options which affects different parts of the caption: One affecting the whole caption (`font`), one which only affects the caption label and separator (`labelfont`) and at least one which only affects the caption text (`textfont`). You set them up using the options

```
font={font options} ,
labelfont={font options} , and
textfont={font options} .
```

And these are the available font options:

|                           |                                     |
|---------------------------|-------------------------------------|
| <code>scriptsize</code>   | Very small size                     |
| <code>footnotesize</code> | The size usually used for footnotes |
| <code>small</code>        | Small size                          |
| <code>normalsize</code>   | Normal size                         |
| <code>large</code>        | Large size                          |
| <code>Large</code>        | Even larger size                    |
| <code>up</code>           | Upright shape                       |
| <code>it</code>           | <i>Italic shape</i>                 |
| <code>sl</code>           | <i>Slanted shape</i>                |
| <code>sc</code>           | SMALL CAPS SHAPE                    |
| <code>md</code>           | Medium series                       |
| <code>bf</code>           | <b>Bold series</b>                  |
| <code>rm</code>           | Roman family                        |
| <code>sf</code>           | Sans Serif family                   |
| <code>tt</code>           | Typewriter family                   |

... Own font options can be defined using `\DeclareCaptionFont`.  
(See section 5: “Do it yourself”)

If you use only one of these options you can omit the braces; e.g., the options `font={small}` and `font=small` will give the same result.

Two examples:

```
font={small,it},labelfont=bf
```

**Figure 14:** *White sand beaches. The pink smoothness of the conch shell. A sea abundant with possibilities. Duty-free shops filled with Europe’s finest gifts and perfumes. Play your favorite game of golf amidst the tropical greens on one of the many championship courses.*

```
font=small,labelfont=bf,textfont=it
```

**Figure 15:** *White sand beaches. The pink smoothness of the conch shell. A sea abundant with possibilities. Duty-free shops filled with Europe’s finest gifts and perfumes. Play your favorite game of golf amidst the tropical greens on one of the many championship courses.*

### 3.4 Margins and further paragraph options

`margin=` For all captions you can specify *either* an extra margin *or* a fixed width. You do this by  
`width=` using the options

```
margin=<amount> or  
width=<amount>
```

Nevertheless what option you use, the left and right margin will be the same.

Two examples will illustrating this:

```
margin=10pt
```

Figure 16: *White sand beaches. The pink smoothness of the conch shell. A sea abundant with possibilities. Duty-free shops filled with Europe’s finest gifts and perfumes. Play your favorite game of golf amidst the tropical greens on one of the many championship courses.*

```
width=.75\textwidth
```

Figure 17: *White sand beaches. The pink smoothness of the conch shell. A sea abundant with possibilities. Duty-free shops filled with Europe’s finest gifts and perfumes. Play your favorite game of golf amidst the tropical greens on one of the many championship courses.*

`parskip=` This option is useful for captions containing more than one paragraph. It specifies the extra vertical space inserted between them:

```
parskip=<amount>
```

One example:

```
margin=10pt,parskip=5pt
```

Figure 18: First paragraph of the caption. This one contains some test, just to show how these options affect the layout of the caption.

Second paragraph of the caption. This one contains some text, too, to show how these options affect the layout of the caption.

hangindent= The option

```
hangindent=<amount>
```

is for setting up a hanging indentation starting from the second line of each paragraph. If the caption contains just a single paragraph, using this option leads to the same result as the option `indentation=` you already know about. But if the caption contains multiple paragraphs you will notice the difference:

```
format=hang,indentation=-.5cm
```

Figure 19: First paragraph of the caption. This one contains some test, just to show how these options affect the layout of the caption.

Second paragraph of the caption. This one contains some text, too, to show how these options affect the layout of the caption.

```
format=hang,hangindent=-.5cm
```

Figure 20: First paragraph of the caption. This one contains some test, just to show how these options affect the layout of the caption.

Second paragraph of the caption. This one contains some text, too, to show how these options affect the layout of the caption.

### 3.5 Styles

`style=` A suitable combination of caption options is called *caption style*. You can compare them more or less to page styles which you set up with `\pagestyle`: The caption style provides all settings for a whole caption layout.

You switch to an already defined caption style with the option

```
style=<style name> .
```

The caption package usually defines only the style `default` which puts all options you already know about to the default ones. This means that specifying the option

```
style=default
```

has the same effect as specifying all these options:

```
format=default, labelformat=default, labelsep=default,
justification=default, font=default, labelfont=default,
textfont=default, margin=0pt, indentation=0pt, parindent=0pt
hangindent=0pt, singlelinecheck=true
```

Own caption styles can be defined using `\DeclareCaptionStyle`. (See section 5: “*Do it yourself*”)

### 3.6 Skips

`aboveskip=` The spaces above and below the caption are controlled by the skips `\abovecaptionskip`  
`belowskip=` and `\belowcaptionskip`. The standard L<sup>A</sup>T<sub>E</sub>X document classes `article`, `report`  
and `book` set `\abovecaptionskip` to 10pt and `\belowcaptionskip` to 0pt.  
Both skips can be changed with the command `\setlength`, but you can use these options, too:

```
aboveskip=(amount) and
belowskip=(amount) .
```

`position=` Using `\abovecaptionskip` and `\belowcaptionskip` has a major design flaw:  
If the caption is typeset *above* (and not *below*) the figure or table they are not set up very  
useful at default, because there will be some extra space above the caption but no space  
between the caption and the figure or table itself. (Remember: `\belowcaptionskip`  
is usually set to 0pt.)

Please compare the spacing in these small tables:

|                                                                                                                                                                                                                                                         |   |   |   |   |                                                                                                                                                                                                                                                         |   |   |   |   |
|---------------------------------------------------------------------------------------------------------------------------------------------------------------------------------------------------------------------------------------------------------|---|---|---|---|---------------------------------------------------------------------------------------------------------------------------------------------------------------------------------------------------------------------------------------------------------|---|---|---|---|
| <p>Table 1: A table</p> <table style="margin-left: auto; margin-right: auto;"> <tr><td style="padding: 0 10px;">A</td><td style="padding: 0 10px;">B</td></tr> <tr><td style="padding: 0 10px;">C</td><td style="padding: 0 10px;">D</td></tr> </table> | A | B | C | D | <table style="margin-left: auto; margin-right: auto;"> <tr><td style="padding: 0 10px;">A</td><td style="padding: 0 10px;">B</td></tr> <tr><td style="padding: 0 10px;">C</td><td style="padding: 0 10px;">D</td></tr> </table> <p>Table 2: A table</p> | A | B | C | D |
| A                                                                                                                                                                                                                                                       | B |   |   |   |                                                                                                                                                                                                                                                         |   |   |   |   |
| C                                                                                                                                                                                                                                                       | D |   |   |   |                                                                                                                                                                                                                                                         |   |   |   |   |
| A                                                                                                                                                                                                                                                       | B |   |   |   |                                                                                                                                                                                                                                                         |   |   |   |   |
| C                                                                                                                                                                                                                                                       | D |   |   |   |                                                                                                                                                                                                                                                         |   |   |   |   |

But you can fix this by using the option `position=`: It specifies how the spacing above  
and below the caption will be used:

```
position=top (or position=above)
```

tells the caption package to use the spacing useful for caption *above* the figure or table  
and

```
position=bottom (or position=below)
```

tells the caption package to use the spacing useful for captions *below* the figure or table.  
(The last one is the default setting except for `longtables`.)

So adding an extra `\captionsetup{position=top}` to the left example table  
gives you proper spacing around both captions:

Table 3: A table

|   |   |
|---|---|
| A | B |
| C | D |

|   |   |
|---|---|
| A | B |
| C | D |

Table 4: A table

(Technically speaking `\abovecaptionskip` and `\belowcaptionskip` will be swapped if you specify the option `position=top`, so in both cases `\abovecaptionskip` will be used between the caption and the figure or table itself.)

This option is especially useful when used together with the optional argument of the `\captionsetup` command. (See section 4: “*Useful stuff*” for details)

For example

```
\captionsetup[table]{position=top}
```

causes all captions within tables to be treated as captions *above* the table (regarding spacing around it). Because this is a very common setting the caption package offers an abbreviating option for the use with `\usepackage`:

`tableposition=`  
New feature  
v3.0a

```
\usepackage[... ,tableposition=top]{caption}2
```

is equivalent to

```
\usepackage[...]{caption}
\captionsetup[table]{position=top}
```

## 4 Useful stuff

`\caption` The command

```
\caption[⟨lst_entry⟩]{⟨heading⟩}
```

typesets the caption inside a floating environment like `figure` or `table`. Well, you already know this, but the caption package offers an extension: If you leave the argument `⟨lst_entry⟩` empty, no entry in the list of figures or tables will be made. For example:

```
\caption[] {A figure without entry in the list of figures.}
```

`\caption*` The `longtable` package defines the command `\caption*` which typesets the caption without label and without entry in the list of tables. An example:

```
\begin{longtable}{cc}
\caption*{A table}\\
A & B \\
C & D \\
\end{longtable}
```

looks like

---

<sup>2</sup>Please note that this is *not* sufficient when using a KOMA-Script document class, you need to use the *global* option `tablecaptionabove`, too.

A table

|   |   |
|---|---|
| A | B |
| C | D |

This package offers this feature, too, so you can use this command now within every floating environment like `figure` or `table`, like:

```
\begin{table}
  \caption*{A table}
  \begin{tabular}{cc}
    A & B \\
    C & D \\
  \end{tabular}
\end{table}
```

`\captionof` Sometimes you want to typeset a caption *outside* a floating environment, putting a figure within a `minipage` for instance. For this purpose the `caption` package offers the command `\captionof*`

```
\captionof{<float type>}[<lst-entry>]{<heading>}
```

Note that the first argument, the `<float type>`, is mandatory here, because the `\captionof` command needs to know which name to put into the caption label (e.g. “Figure” or “Table”) and in which list to put the contents entry. An example:

```
\captionof{figure}{A figure}
\captionof{table}{A table}
```

typesets captions like this:

Figure 21: A figure

Table 6: A table

The star variant `\captionof*` has the same behaviour as the `\caption*` command: it typesets the caption without label and without entry to the list of figures or tables.

Please use both `\captionof` and `\captionof*` only *inside* environments (like `minipage` or `\parbox`), otherwise a page break can appear between content and caption. Furthermore some strange effects could occur (e.g., wrong spacing around captions).

`\ContinuedFloat` Sometimes you want to split figures or tables without giving them their own reference number. This is what the command

```
\ContinuedFloat
```

is for; it should be used as first command inside the floating environment. It prevents the increment of the relevant counter (usually done by `\caption`) so a figure or table with a `\ContinuedFloat` in it gets the same reference number as the figure or table before.

An example:

```
\begin{table}
\caption{A table}
...
\end{table}
...
\begin{table}\ContinuedFloat
\caption{A table (cont.)}
...
\end{table}
```

gives the following result:

Table 7: A table

...

Table 7: A table (cont.)

`\captionsetup` We already know the `\captionsetup` command (see section 2: “Using the package”), but this time we get enlighten about its optional argument *float type*. Remember, the syntax of this command is

```
\captionsetup[float type]{options}
```

If a *float type* gets specified, all the *options* don’t change anything at this time. Instead they only get marked for a later use, when a caption inside of a floating environment of the particular type *float type* gets typeset. For example

```
\captionsetup[figure]{options}
```

forces captions within a `figure` environment to use the given *options*.

Here comes an example to illustrate this:

```
\captionsetup{font=small}
\captionsetup[figure]{labelfont=bf}
```

gives captions like this:

**Figure 22:** A figure

Table 8: A table

As you see the command `\captionsetup[figure]{labelfont=bf}` only changed the font of the figure caption labels, not touching all other ones.

`\clearcaptionsetup` If you want to get rid of these parameters marked for an automatic use within a particular environment you can use the command

```
\clearcaptionsetup{<float type>} .
```

For example `\clearcaptionsetup{figure}` would clear the extra handling in the example above:

Figure 23: A figure

Table 9: A table

As *<float type>* you can usually give one of these two only: `figure` or `table`. But as we will see later some  $\text{\LaTeX}$  packages (like the `float`, `longtable`, and `sidecap` package for example) offer additional floating environments and these two commands can also be used with them.

## 5 Do it yourself!

A family of commands is provided to allow users to define their own formats. This enables information on separators, justification, fonts, and styles to be associated with a name and kept in one place (these commands need to appear in the document preamble, this is the part between `\documentclass` and `\begin{document}`).

`\DeclareCaptionFormat` You can define your own caption formats using the command

```
\DeclareCaptionFormat{<name>}{<code using #1, #2 and #3>} .
```

At usage the system replaces `#1` with the caption label, `#2` with the separator and `#3` with the text. So the standard format `plain` is pre-defined by the caption package as

```
\DeclareCaptionFormat{plain}{#1#2#3\par}
```

`\DeclareCaptionLabelFormat` Likewise you can define your own caption label formats:

```
\DeclareCaptionLabelFormat{<name>}{<code using #1 and #2>}
```

At usage `#1` gets replaced with the name (e.g. “figure”) and `#2` gets replaced with the reference number (e.g. “12”).

`\bothIfFirst` If you define your own caption label formats and use the `subfig` package[10], you should  
`\bothIfSecond` take care of empty caption label names. For this purpose the commands

```
\bothIfFirst{<first arg>}{<second arg>} and  
\bothIfSecond{<first arg>}{<second arg>}
```

are offered. `\bothIfFirst` tests if the first argument exists (means: is not empty), `\bothIfSecond` tests if the second argument exists. If yes, both arguments get typeset, otherwise none of them.

For example the standard label format `simple` is *not* defined as

```
\DeclareCaptionLabelFormat{simple}{#1 #2} ,
```

because this could cause an extra space if #1 is empty. Instead `simple` is defined as

```
\DeclareCaptionLabelFormat{simple}{\bothIfFirst{#1}{ }#2}
,
```

causing the space to appear only if the label name is present.

`\DeclareCaptionLabelSeparator` You can define your own caption label separators with

```
\DeclareCaptionLabelSeparator{<name>}{<code>} .
```

Again an easy example taken from the `caption` package itself:

```
\DeclareCaptionLabelSeparator{colon}{: }
```

`\DeclareCaptionJustification` You can define your own caption justifications with

```
\DeclareCaptionJustification{<name>}{<code>} .
```

The `<code>` simply gets typeset just before the caption. E.g. using the justification `raggedright`, which is defined as

```
\DeclareCaptionJustification{raggedright}{\raggedright}
,
```

lets captions with all lines moved to the left margin.

`\DeclareCaptionFont` You can define your own caption fonts with

```
\DeclareCaptionFont{<name>}{<code>} .
```

For example this package defines the options `small` and `bf` as

```
\DeclareCaptionFont{small}{\small} and
\DeclareCaptionFont{bf}{\bfseries} .
```

New description  
v3.0h

The line spacing could be customized using the `setspace` package, for example:

```
\usepackage{setspace}
\captionsetup{font={onehalfspacing, small}, labelfont=bf}
```

**Figure 24:** White sand beaches. The pink smoothness of the conch shell. A sea abundant with possibilities. Duty-free shops filled with Europe’s finest gifts and perfumes. Play your favorite game of golf amidst the tropical greens on one of the many championship courses.

An example which brings color into life:

```
\usepackage{color}
\DeclareCaptionFont{red}{\color{red}}
\DeclareCaptionFont{green}{\color{green}}
\DeclareCaptionFont{blue}{\color{blue}}
\captionsetup{labelfont=blue,textfont=green}
```

**Figure 25:** White sand beaches. The pink smoothness of the conch shell. A sea abundant with possibilities. Duty-free shops filled with Europe’s finest gifts and perfumes. Play your favorite game of golf amidst the tropical greens on one of the many championship courses.

`\DeclareCaptionStyle` You can define your own caption styles with

```
\DeclareCaptionStyle{<name>}[<additional options>]{<options>}
```

Remember, caption styles are just a collection of suitable options, saved under a given name. You can wake up these options at any time with the option `style=<style name>`.

All caption styles are based on the default set of options. (See section 3.5: “*Styles*” for a complete list.) So you only need to specify options which are different to them.

If you specify `<additional options>` they get used in addition when the caption fits into a single line and this check was not disabled with the option `singlelinecheck=off`.

Again a very easy example taken from the core of this package: The caption style `default` is pre-defined as

```
\DeclareCaptionStyle{default}[justification=centering]{}
.
```

## 5.1 Further Examples

If you would like to have a colon *and* a line break as caption separator you could define it this way:

```
\DeclareCaptionLabelSeparator{period-newline}{. \\}
```

Selecting this separator with `\captionsetup{labelsep=period-newline}` you get captions like this:

**Figure 26.**

White sand beaches. The pink smoothness of the conch shell. A sea abundant with possibilities. Duty-free shops filled with Europe’s finest gifts and perfumes. Play your favorite game of golf amidst the tropical greens on one of the many championship courses.

For short captions—which fit into one single line—this separator may not be satisfying, even when the automatically centering process is switched off (with `singlelinecheck=off`):

**Figure 27.**

A figure.

An own caption style which selects another caption separator automatically puts this right:

```
\DeclareCaptionStyle{period-newline}%  
  [labelsep=period]{labelsep=period-newline}
```

**Figure 27.** A figure.

If you would like to keep the centering of these captions instead, an appropriate definition would be something like

```
\DeclareCaptionStyle{period-newline}%  
  [labelsep=period, justification=centering]%  
  {labelsep=period-newline} .
```

Using this definition short captions look like

**Figure 27.** A figure.

while long ones still have a line break after the caption label.

Slightly changed, you also get centered captions if they are longer than one line:

```
\DeclareCaptionStyle{period-newline}%  
  [labelsep=period]%  
  {labelsep=period-newline, justification=centering}
```

**Figure 28.**

White sand beaches. The pink smoothness of the conch shell. A sea abundant with possibilities. Duty-free shops filled with Europe’s finest gifts and perfumes. Play your favorite game of golf amidst the tropical greens on one of the many championship courses.

Another example: You want captions to look like this:

White sand beaches. The pink smoothness of the conch shell. A sea abundant with possibilities. Duty-free shops filled with Europe’s finest gifts and perfumes. Play your favorite game of golf amidst the tropical greens on one of the many championship courses.

*(Figure 29)*

You could do it this way:

```
\DeclareCaptionFormat{reverse}{#3#2#1}  
\DeclareCaptionLabelFormat{fullparens}{(\bothIfFirst{#1}{ }#2)}  
\DeclareCaptionLabelSeparator{fill}{\hfill}  
\captionsetup{format=reverse, labelformat=fullparens,  
  labelsep=fill, font=small, labelfont=it}
```

Another example: The caption text should go into the left margin; a possible solution would be:

```
\DeclareCaptionFormat{llap}{\llap{#1#2}#3\par}
\captionsetup{format=llap,labelsep=quad,singlelinecheck=no}
```

As a result you would get captions like this:

Figure 30 White sand beaches. The pink smoothness of the conch shell. A sea abundant with possibilities. Duty-free shops filled with Europe's finest gifts and perfumes. Play your favorite game of golf amidst the tropical greens on one of the many championship courses.

## 6 Using non-standard document classes

New description v3.0p The caption package was developed using the standard document classes `article`, `report` and `book`, it also works with the Dutch document classes `artikel`, `rapport` and `boek`. It is *incompatible* with all other document classes, except the ones based on one of the above.

If you are unsure if your document class is supported or not, it's better *not* to use this package. You could try if your document will compile fine with the caption package anyway, but you should watch carefully if side-effects occur, i.e. the look and feel of your captions should *not* change if you just include the caption package without options. (If it does, you can carry on, but you should be warned that the output could change with upcoming versions of the caption package.) If this is fine, you can start setting options with `\usepackage[...]{caption}` or `\captionsetup` and keep your fingers crossed.

The upcoming version v3.1 of the caption package will be adapted to several document classes, e.g. the beamer class and the KOMA-Script ones. It's planned for release during Summer 2007.

## 7 Compatibility to other packages

The caption package contains special adaptations to other packages, so the captions should always look like you have specified them to look like.

These are the packages the caption package is adapted to:

|                           |                                                               |
|---------------------------|---------------------------------------------------------------|
| <code>float</code>        | Gives you the possibility to define new floating environments |
| <code>listings</code>     | Typesets source code listings                                 |
| <code>longtable</code>    | Typesets tables spanned over multiple pages                   |
| <code>rotating</code>     | Supports rotated figures and tables                           |
| <code>sidecap</code>      | Offers captions <i>beside</i> figures or tables               |
| <code>supertabular</code> | Typesets tables spanned over multiple pages                   |

New feature v3.0b If you use one of the above packages together with the caption package you get the additional possibility to set up captions with

```
\captionsetup[environment]{options} ,
```

where *environment* stands for any environment the above packages offer. (Please note that this do not work with the `sideways` environments offered by the rotating package.)  
For example

```
\captionsetup[lstlisting]{labelfont=bf}
```

forces captions inside the `lstlisting` environment to have bold labels.

If a certain support is not desired you can switch it off using the caption package option

```
\usepackage[... ,package=no]{caption} .
```

For example specifying the option `float=no` means you don't like the caption package to support the float package. (Note: You can specify these options only within the `\usepackage` command, especially *not* at a later time with `\captionsetup`.)

For further information about the packages mentioned above please take a look at the documentation belonging to them or buy yourself *The L<sup>A</sup>T<sub>E</sub>X Companion*[1].

## 7.1 The float package

A very useful feature is provided by the float package[2]: It offers the float placement specifier `H` which is much more restrictive than the specifier `h` offered by L<sup>A</sup>T<sub>E</sub>X. While the latter one is only a recommendation to L<sup>A</sup>T<sub>E</sub>X to set the float “here”, the `H` forces the float to appear exactly at the spot where it occurs in your input file and nowhere else.

Furthermore it offers different styles for floating environments, these styles are `plain`, `plaintop`, `ruled`, and `boxed`. You can link one of these styles to either new floating environments or to one of the existing environments `figure` and `table`.

If you are using the caption package together with the float package a caption style called `ruled` gets defined automatically:

```
\DeclareCaptionStyle{ruled}{labelfont=bf,labelsep=space}
```

This style represents the caption layout in `ruled` styled floats. For you as an end user this means that captions within `ruled` floats will always look like this, nevertheless what generic caption options do you specify:

---

**Program 7.1** The first program. This hasn't got anything to do with the package but is included as an example. Note the `ruled` float style.

---

```
#include <stdio.h>

int main(int argc, char **argv)
{
    for (int i = 0; i < argc; ++i)
        printf("argv[%d] = %s\n", i, argv[i]);
    return 0;
}
```

---

If you want a different layout for `ruled` captions you have to define your own one using the command

```
\DeclareCaptionStyle{ruled}{options} .
```

This mechanism also works with all other float styles. If you want a special caption layout—for `plain` or `boxed` floats for example—you can simply define a suitable caption style with the same name as the float style.

**Note:** For successful cooperation you need the float package version 1.3 or newer.

## 7.2 The listings package

New description  
v3.0b

The `listings` package[6] is a source code printer for  $\LaTeX$ . You can typeset stand alone files as well as listings with an environment similar to `verbatim` as well as you can print code snippets using a command similar to `\verb`. Many parameters control the output and if your preferred programming language isn't already supported, you can make your own definition.

**Note:** For successful cooperation you need the `listings` package version 1.2 or higher. You'll get an error message when using an older version!

## 7.3 The longtable package

The `longtable` package[7] offers the environment `longtable` which behaves similar to the `tabular` environment, but the table itself can span multiple pages.

**Note:** For successful cooperation you need the `longtable` package version 3.15 or newer.

## 7.4 The rotating package

The `rotating` package[8] offers the floating environments `sidewaysfigure` and `sideways-table` which are just like normal figures and tables but rotated by 90 degree. Furthermore they always use a full page on their own.

## 7.5 The sidecap package

New description v3.0b The sidecap package[9] offers the floating environments `SCfigure` and `SCTable` which are like normal figures and tables but the caption will be put *beside* the contents.

The sidecap package offers it's own options for justification. If set, they will override the one specified with the caption option `justification=` for captions beside their contents.

`listof=` Using the sidecap package you will probably notice that suppressing the entry in the list of figures or tables with `\caption[]{\dots}` won't work inside these environments. This is caused by the implementation design of the sidecap package, but you can use `\captionsetup{listof=false}` inside the figure or table as an alternative here.

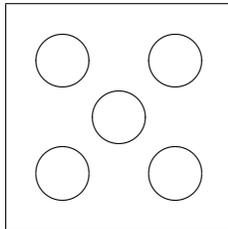

**Figure 31:** A small example with the caption beside the figure.

## 7.6 The supertabular package

The supertabular package[11] offers the environment `supertabular` which is quite similar to the `longtable` environment provided by the `longtable` package. Both offers the typesetting of tables which can span multiple pages. For a detailed discussion about the differences between these powerful packages please take a look at The L<sup>A</sup>T<sub>E</sub>X Companion[1].

## 7.7 Known incompatibilities

New description v3.0b Using the caption package together with one of the following packages is not recommended; usually this would cause unwanted side effects or even errors:

`ccaption`, `ftcap`, `hvfloat`, and `nonfloat`

# 8 Compatibility to older versions

## 8.1 The caption package version 1.x

This version of the caption package still supports the old options and commands provided by the version 1.x of this package. So there shouldn't occur any problems compiling old documents, but please don't mix old options and commands with the new ones. This isn't supported and can cause ugly side effects.

Here comes a short oversight of the obsolete options and commands and how they have been replaced within this version of the caption package:

| caption v1.x | caption v3.x             |
|--------------|--------------------------|
| normal       | format=plain             |
| hang         | format=hang              |
| isu          | format=hang              |
| center       | justification=centering  |
| centerlast   | justification=centerlast |
| nooneline    | singlelinecheck=off      |
| scriptsize   | font=scriptsize          |
| footnotesize | font=footnotesize        |
| small        | font=small               |
| normalsize   | font=normalsize          |
| large        | font=large               |
| Large        | font=Large               |
| up           | labelfont=up             |
| it           | labelfont=it             |
| sl           | labelfont=sl             |
| sc           | labelfont=sc             |
| md           | labelfont=md             |
| bf           | labelfont=bf             |
| rm           | labelfont=rm             |
| sf           | labelfont=sf             |
| tt           | labelfont=tt             |

Beside the options for setting up the desired font there were also the commands `\captionsize` resp. `\captionfont` and `\captionlabelfont` who could be redefined with `\renewcommand` and allowed an alternate and more flexible way to change the font used for captions. This mechanism was replaced by the commands

```
\DeclareCaptionFont{...}{...} and
\captionsetup{font=...,labelfont=...} .
```

(See section 5: “*Do it yourself*”)

Setting the margin for captions was done in v1.x with

```
\setlength{\captionmargin}{...} .
```

This was replaced by

```
\captionsetup{margin=...} .
```

(See section 3.4: “*Margins and further paragraph options*”)

For example the old-style code

```
\usepackage[hang,bf]{caption}
\renewcommand\captionfont{\small\sffamily}
\setlength\captionmargin{10pt}
```

will still work fine, but should be written today as

```
\usepackage[format=hang,labelfont=bf,font={small,sf},
margin=10pt]{caption}
```

or

```
\usepackage{caption}
\captionsetup{format=hang,labelfont=bf,font={small,sf},
margin=10pt} .
```

The quite exotic option `ruled` which allowed a partial usage of the caption settings for ruled floats defined with the `float` package will be emulated by this version of the caption package, too. But using this option is not recommended anymore since this version of the caption package offers a more flexible way for changing the captions of these floating environments:

```
\DeclareCaptionStyle{ruled}{...}
```

resp.

```
\captionsetup[ruled]{...} .
```

(See section 5: “*Do it yourself*”, 4: “*Useful stuff*”, and 7.1: “*The float package*”)

## 8.2 The caption2 package version 2.x

Although they do very similar stuff, the packages `caption` and its experimental and now obsolete variant `caption2` have a very different implementation design. Therefore a full compatibility could not be offered. For that reason you will still find a file called `caption2.sty` in this package distribution, so old documents using the `caption2` package will still compile fine.

Newly created documents should use the actual version of the `caption` package instead. In most cases it's sufficient to replace the command

```
\usepackage[...]{caption2}
```

by

```
\usepackage[...]{caption} .
```

But some options and commands will not be emulated, so you can get error messages afterwards. This section will hopefully help you removing these errors. If you have problems migrating from `caption2` to `caption` please don't hesitate to send me an e-mail asking for help.

In addition to the obsolete options shown in the last section these ones will be emulated, too:

| caption2 v2.x | caption v3.x              |
|---------------|---------------------------|
| flushleft     | justification=raggedright |
| flushright    | justification=raggedleft  |
| oneline       | singlelinecheck=on        |

Setting the margin for captions was done in v2.x with

```
\setcaptionmargin{...} resp. \setcaptionwidth{...} .
```

This was replaced by

```
\captionsetup{margin=...} resp. \captionsetup{width=...} .
```

(See section 3.4: “*Margins and further paragraph options*”)

Setting an indentation was done in v2.x with

```
\captionstyle{indent}
\setlength\captionindent{...} .
```

This is now done with

```
\captionsetup{format=plain,indentation=...} .
```

The so-called single-line-check was controlled by the commands `\onelinecaptionsfalse` (for switching the check off) and `\onelinecaptionstrue` (for switching the check on). This was replaced by `\captionsetup{singlelinecheck=off}` resp. `\captionsetup{singlelinecheck=on}`. (See section 3.2: “*Justification*”)

The commands

```
\captionlabeldelim, \captionlabelsep, \captionstyle,
\defcaptionstyle, \newcaptionstyle, and \renewcaptionstyle
```

do not have a simple replacement and therefore will not be emulated by this version of the caption package. (So using them will cause error messages.) Rewriting such code is not always easy and straight-ahead, but by conscientious reading of this manual you should find appropriate options and commands instead.

The v2.x option `ignoreLTcapwidth` do not have a replacement, too. But in most cases you can simply drop using that option because in this version of the caption package the value of `\LTcapwidth` will be ignored anyway (unless you set it to a different value than the default one). (See section 7.3: “*The longtable package*”)

## 9 Further reading

I recommend the following documents for further reading:

- The T<sub>E</sub>X FAQ - Frequently asked questions about T<sub>E</sub>X and L<sup>A</sup>T<sub>E</sub>X:

<http://faq.tug.org/>

- A French FAQ can be found at

<http://www.grappa.univ-lille3.fr/FAQ-LaTeX/>

- epslatex from Keith Reckdahl contains many tips around including graphics in L<sup>A</sup>T<sub>E</sub>X 2<sub>ε</sub> documents. You will find this document in the directory

<ftp://ftp.ctan.org/pub/tex/info/epslatex/>

## 10 Thanks

I would like to thank Katja Melzner, Steven D. Cochran, Frank Mittelbach, David Carlisle, Carsten Heinz, Olga Lapko, and Keith Reckdahl. Thanks a lot for all your help, ideas, patience, spirit, and support!

Also I would like to thank Harald Harders, Peter Löffler, Peng Yu, Alexander Zimmermann, Matthias Pospiech, Jürgen Wieferink, Christoph Bartoschek, Uwe Stöhr, Ralf Stubner, Geoff Vallis, Florian Keiler, Jürgen Göbel, Uwe Siart, Sang-Heon Shim, Henrik Lundell, David Byers, William Asquith, and Prof. Dr. Dirk Hoffmann, who all helped to make this package a better one.

## 11 The Implementation

The caption package consists of two parts – the kernel (`caption3.sty`) and the main package (`caption.sty`).

The kernel provides all the user commands and internal macros which are necessary for typesetting captions and setting parameters regarding these. While the standard  $\LaTeX$  document classes provides an internal command called `\@makecaption` and no options to control its behavior (except the vertical skips above and below the caption itself), we provide similar commands called `\caption@make` and `\caption@@make`, but with a lot of options which can be selected with `\captionsetup`. Loading the kernel part do not change the output of a  $\LaTeX$  document – it just provides functionality which can be used by  $\LaTeX 2\epsilon$  packages which typesets captions, like the `caption` package or the `subfig` package.

The `caption` package itself redefines the  $\LaTeX$  commands `\caption`, `\@caption`, and `\@makecaption` and maps the latter one to `\caption@@make`, giving the user the possibility to control the captions of the floating environments `figure` and `table`. Furthermore it does similar to the caption stuff coming from other packages (like the `longtable` or `supertabular` package): Mapping the appropriate internal commands (like `\LT@makecaption` or `\ST@caption`) to the ones offered by the `caption` kernel. So you can think of the `caption` package as a layer package, it simply provides adaptation layers between the caption stuff coming from  $\LaTeX 2\epsilon$  itself or a  $\LaTeX 2\epsilon$  package and the caption stuff offered by the `caption` kernel.

### 11.1 Kernel

#### Identification

```
1 \NeedsTeXFormat{LaTeX2e}[1994/12/01]
2 \ProvidesPackage{caption3}[2007/04/11 v3.0q caption3 kernel (AR)]
```

#### Generic helpers

`\@nameundef` This is the opposite to `\@namedef` which is offered by the  $\LaTeX$  kernel. We use it to remove the definition of some commands and keyval options after `\begin{document}` (to save  $\TeX$  memory) and to remove caption options defined with `\captionsetup[⟨type⟩]`.

```
3 \providecommand*\@nameundef[1]{%
4   \expandafter\let\csname #1\endcsname\@undefined}
```

`\l@addto@macro` The  $\LaTeX 2\epsilon$  kernel offers the internal helper macro `\g@addto@macro` which globally adds commands to any existing macro, like in `\AtBeginDocument`. This is the same but it works local, not global (using `\edef` instead of `\xdef`).

```
5 \providecommand{\l@addto@macro}[2]{%
6   \begingroup
7     \toks@\expandafter{#1#2}%
8     \edef\@tempa{\endgroup\def\noexpand#1{\the\toks@}}%
9   \@tempa}
```

`\bothIfFirst` `\bothIfFirst` tests if the first argument is not empty, `\bothIfSecond` tests if the second argument is not empty. If yes both arguments get typeset, otherwise none of them.

```

10 \def\bothIfFirst#1#2{%
11   \protected@edef\caption@tempa{#1}%
12   \ifx\caption@tempa\@empty\else
13     #1#2%
14   \fi}

15 \def\bothIfSecond#1#2{%
16   \protected@edef\caption@tempa{#2}%
17   \ifx\caption@tempa\@empty\else
18     #1#2%
19   \fi}

```

`\caption@ifinlist` This helper macro checks if the first argument is in the comma separated list which is offered as second argument. So for example

```
\caption@ifinlist{frank}{axel, frank, steven}{yes}{no}
```

would expand to `yes`.

```

20 \def\caption@ifinlist#1#2{%
21   \let\next\@secondoftwo
22   \edef\caption@tempa{#1}%
23   \@for\caption@tempb:={#2}\do{%
24     \ifx\caption@tempa\caption@tempb
25       \let\next\@firstoftwo
26     \fi}%
27   \next}

```

`\caption@setbool` For setting and testing boolean options we offer these three helper macros:

```

\caption@ifbool
\caption@undefbool
\caption@setbool{<name>}{<value>}
    (with value = false/true/no/yes/off/on/0/1)
\caption@ifbool{<name>}{<if-clause>}{<else-clause>}
\caption@undefbool{<name>}

```

```

28 \def\caption@setbool#1#2{%
29   \caption@ifinlist{#2}{1,true,yes,on}{%
30     \expandafter\let\csname caption@if#1\endcsname\@firstoftwo
31   }{\caption@ifinlist{#2}{0,false,no,off}{%
32     \expandafter\let\csname caption@if#1\endcsname\@secondoftwo
33   }{%
34     \caption@Error{Undefined boolean value `#2'}%
35   }}}

36 \def\caption@ifbool#1{\@nameuse{caption@if#1}}
37 \def\caption@undefbool#1{\@nameundef{caption@if#1}}

```

`\caption@newcounter` To save counter space we use commands instead of counters.  
`\caption@setcounter` `\caption@newcounter#1{\gdef#1{0}}`  
`\caption@addtocounter` `\caption@setcounter#1#2{\xdef#1{#2}}`  
`\caption@stepcounter`

```

40 \def\caption@addtocounter#1#2{%
41   \begingroup
42     \@tempcnta#1%
43     \advance\@tempcnta#2%
44     \xdef#1{\the\@tempcnta}%
45   \endgroup}
46 \def\caption@stepcounter#1{\caption@addtocounter#1\@ne}

```

## Errors

`\caption@Error` This is mainly identical to `\PackageError{caption}{#1}{\caption@eh}`.

```

47 \newcommand\caption@Package{caption}
48 \newcommand*\caption@Error[1]{%
49   \PackageError\caption@Package{#1}\caption@eh}

```

`\caption@eh` At the moment we only offer this simple error message as generic helper for the user.

```

50 \newcommand\caption@eh{%
51   If you do not understand this error, please take a closer look\MessageBreak
52   at the documentation of the '\caption@Package' package.\MessageBreak
53   \@ehc}

```

## Using the keyval package

We need the `keyval` package for option handling, so we load it here.

```

54 \RequirePackage{keyval}[1997/11/10]

```

`\undefine@key` This helper macro is the opposite of `\define@key`, it removes a `keyval` definition.

```

55 \providecommand*\undefine@key[2]{%
56   \@nameundef{KV@#1@#2}\@nameundef{KV@#1@#2@default}}

```

`\DeclareCaptionOption` `\DeclareCaptionOption{<option>}{<code>}`  
`\DeclareCaptionOption*{<option>}{<code>}`

We declare our options using these commands (instead of using `\DeclareOption` offered by `LATEX 2ε`), so the `keyval` package is used. The starred form makes the option available during the lifetime of the current package only, so they can be used with `\usepackage`, but *not* with `\captionsetup` later on.

```

57 \newcommand\DeclareCaptionOption{%
58   \@ifstar{\caption@declareoption\AtEndOfPackage}%
59   {\caption@declareoption\@gobble}}
60 \newcommand*\caption@declareoption[2]{%
61   #1{\undefine@key{caption}{#2}}\define@key{caption}{#2}}
62 \@onlypreamble\DeclareCaptionOption
63 \@onlypreamble\caption@declareoption

```

`\captionsetup` `\captionsetup[<type>]{<keyval-list of options>}`

If the optional argument ‘type’ is specified, we simply save or append the option list, otherwise we ‘execute’ it with `\setkeys`.

```

64 \newcommand\captionsetup{\@ifnextchar[\caption@setuptype\caption@setup}

```

```

65 \newcommand\caption@typ@{caption@typ@} % This saves 74 words of TeX memory
66 \def\caption@setuptype[#1]#2{%
67   \@ifundefined{caption@typ@#1}%
68     {\@namedef{caption@typ@#1}{#2}}%
69     {\expandafter\l@addto@macro\csname\caption@typ@#1\endcsname{,#2}}
70 \newcommand\caption@setup{\caption@setkeys{caption}}

```

`\caption@setkeys` This one simply calls `\setkeys{<package>}{<args>}` but lets the error messages refer to the *<package>* package instead of the `keyval` package.

```

71 \newcommand*\caption@setkeys{%
72   \@dblarg\caption@@setkeys}
73 \long\def\caption@@setkeys[#1]#2#3{%
74   \ifnum\caption@keydepth=0\relax
75     \let\caption@KV@errx\KV@errx
76     \let\caption@KV@err\KV@err
77     \let\KV@errx\caption@Error
78     \let\KV@err\caption@Error
79   \fi
80   \caption@stepcounter\caption@keydepth
81 %
82   \def\caption@Package{#1}%
83   \caption@Debug{\protect\setkeys{#2}{#3}}%
84   \setkeys{#2}{#3}%
85   \def\caption@Package{caption}%
86 %
87   \caption@addtocounter\caption@keydepth\m@ne
88   \ifnum\caption@keydepth=0\relax
89     \let\KV@errx\caption@KV@errx
90     \let\KV@err\caption@KV@err
91   \fi}
92 \caption@newcounter\caption@keydepth

```

`\caption@settype` `\caption@settype{<type>}`

Caption options which have been saved with `\captionsetup[<type>]` can be executed using this command. (It simply executes the saved option list, if there is any.)

```

93 \newcommand*\caption@settype[1]{%
94   \@ifundefined{caption@typ@#1}{}{%
95     \caption@esetup{\csname\caption@typ@#1\endcsname}}

```

`\caption@esetup` `\caption@esetup{<keyval-list of options>}`

To execute a keyval-list of options saved within a macro we need this special version of `\caption@setup` which expands the argument first.

```

96 \newcommand*\caption@esetup[1]{%
97   \edef\caption@tempa{\noexpand\caption@setup{#1}}%
98   \caption@tempa}

```

`\clearcaptionsetup` `\clearcaptionsetup{<type>}`

This removes the saved option list associated with *<type>*.

```

99 \newcommand*\clearcaptionsetup[1]{\@nameundef{caption@typ@#1}}

```

`\showcaptionsetup` `\showcaptionsetup[<package>]{<type>}`  
**This comes for debugging issues: It shows the saved option list which is associated with *<type>*.**

```

100 \newcommand*\showcaptionsetup[2][\@firstofone]{%
101   \GenericWarning{ }{%
102     #1 Caption Info: KV list on `#2'\MessageBreak
103     #1 Caption Data: (%
104     \@ifundefined{\caption@typ@#2}{%
105       % empty -- print nothing
106     }{%
107       \@nameuse{\caption@typ@#2}%
108     }%
109   )}}
```

`\caption@ProcessOptions` **We process our options using the keyval package, so we use this one instead of `\ProcessOptions` offered by L<sup>A</sup>T<sub>E</sub>X 2<sub>ε</sub>. (This code was taken from the hyperref package and improved.)**

```

110 \newcommand*\caption@ProcessOptions[1]{%
111   \let\@tempc\relax
112   \let\caption@tempa\@empty
113   \@for\CurrentOption:=\@classoptionslist\do{%
114     \@ifundefined{KV@#1@\CurrentOption}{%
115       }{%
116         \@ifundefined{KV@#1@\CurrentOption @default}{%
117           \PackageInfo{#1}{Global option '\CurrentOption' ignored}%
118         }{%
119           \PackageInfo{#1}{Global option '\CurrentOption' processed}%
120           \edef\caption@tempa{\caption@tempa,\CurrentOption,}%
121           \@expandtwoargs\@removeelement\CurrentOption
122           \@unusedoptionlist\@unusedoptionlist
123         }%
124       }%
125     }%
126     \edef\caption@tempa{%
127       \noexpand\caption@setkeys{#1}{%
128         \caption@tempa\@optionlist{\@currname.\@current}%
129       }%
130     }%
131     \caption@tempa
132   \let\CurrentOption\@empty
133   \AtEndOfPackage{\let\@unprocessedoptions\relax}}
134 \@onlypreamble\caption@ProcessOptions
```

### Margin resp. width

`\captionmargin` and `\captionwidth` contain the extra margin resp. the total width used for captions. Please never set these values in a direct way, they are just accessible in user documents to provide compatibility to `caption.sty v1.x`.

Note that we can only set one value at a time, ‘margin’ or ‘width’. If `\captionwidth` is not zero we will take this value afterwards, otherwise `\captionmargin` and `\captionmargin@`.

```
135 \newdimen\captionmargin
136 \newdimen\captionmargin@
137 \newdimen\captionwidth

138 \DeclareCaptionOption{margin}{\setcaptionmargin{#1}}
139 \DeclareCaptionOption{width}{\setcaptionwidth{#1}}
140 \DeclareCaptionOption{twoside}[1]{\caption@setbool{twoside}{#1}}
```

`\setcaptionmargin` `\setcaptionmargin{<amount>}` `\setcaptionmargin{<amount>}`  
**Please never use this in user documents, it’s just there to provide compatibility to `caption2.sty v2.x`.**

```
141 \newcommand*\setcaptionmargin[1]{%
142   \captionwidth\z@
143   \caption@@setmargin#1,#1,\@nil\@@}
144 \def\caption@@setmargin#1,#2,#3\@@{%
145   \setlength\captionmargin{#1}%
146   \setlength\captionmargin@{#2}%
147   \advance\captionmargin@ by -\captionmargin}
```

`\setcaptionwidth` `\setcaptionwidth{<amount>}` `\setcaptionwidth{<amount>}`  
**Please never use this in user documents, it’s just there to provide compatibility to `caption2.sty v2.x`.**

```
148 \newcommand\setcaptionwidth{%
149   \setlength\captionwidth}
```

`\caption@count` **This counter numbers the captions. It will be used inside `\caption@ifoddpages` only.**

```
150 \caption@newcounter\caption@count
```

`\caption@newlabel` **This command is a modified version of `\newlabel` from `LATEX2e`. It will be written to the `.aux` file to pass label information from one run to another. It will be used inside `\caption@ifoddpages` and `\caption@ragged`.**

```
151 \newcommand*\caption@newlabel{\@newlabel{caption}}
```

`\caption@thepage` **This command is a modified version of `\thepage` from `LATEX2e`. It will be used inside `\caption@ifoddpages` only.**

```
152 \newcommand*\caption@thepage{\the\c@page}
```

`\caption@ifoddpages` **Note: This macro re-defines itself so the `.aux` file will only be used once per group.**

```
153 \def\caption@ifoddpages{%
154   \caption@iftwoside{%
   \refstepcounter{caption@count}
155   \caption@stepcounter\caption@count
   \label{\the\caption@count}
156   \protected@write\@auxout{\let\caption@thepage\relax}%
157     {\string\caption@newlabel{\caption@count}{\caption@thepage}}%
```

```

\edef\caption@thepage{\pageref{\the\caption@count}}
158 \expandafter\ifx\csname caption@\caption@count\endcsname\relax
159 \G@refundefinedtrue % => 'There are undefined references.'
160 \PackageWarning{caption3}{Reference on page \thepage \space undefined}%
161 \else
162 \expandafter\let\expandafter\caption@thepage
163 \csname caption@\caption@count\endcsname
164 \fi
\ifodd\caption@thepage...
165 \ifodd\caption@thepage
166 \let\caption@ifoddpage\@firstoftwo
167 \else
168 \let\caption@ifoddpage\@secondoftwo
169 \fi
170 }{\let\caption@ifoddpage\@firstoftwo}%
171 \caption@ifoddpage}

```

### Indentions

```

\captionindent These are the indentions we support.
\captionparindent 172 \newdimen\captionindent
\captionhangindent 173 \newdimen\captionparindent
174 \newdimen\captionhangindent

```

```

175 \DeclareCaptionOption{indent}[\leftmargini]{\setlength\captionindent{#1}}% obsolete
176 \DeclareCaptionOption{indentation}[\leftmargini]{\setlength\captionindent{#1}}
177 \DeclareCaptionOption{hangindent}{\setlength\captionhangindent{#1}}
178 \DeclareCaptionOption{parindent}{\setlength\captionparindent{#1}}
179 \DeclareCaptionOption{parskip}{\l@addto@macro\caption@@par{\setlength\parskip{#1}}}
180 \ifundefined{scr@caption}{}{}%

```

There is an option clash between the KOMA-Script document classes and the caption kernel, both define the options `parindent` and `parskip` but with different meaning. Furthermore the ones defined by the caption kernel take a value as parameter but the KOMA-Script ones do not. So we need special versions of the options `parindent` and `parskip` here, ones who determine if a value is given (and therefore should be treated as our option) or not (and therefore should be ignored by us).

```

181 \let\caption@KV@parindent\KV@caption@parindent
182 \DeclareCaptionOption{parindent}[]{}%
183 \def\caption@tempa{#1}%
184 \ifx\caption@tempa\@empty
185 \PackageInfo{caption3}{Option 'parindent' ignored}%
186 \else
187 \caption@KV@parindent{#1}%
188 \fi}%
189 \let\caption@KV@parskip\KV@caption@parskip
190 \DeclareCaptionOption{parskip}[]{}%

```

```

191 \def\caption@tempa{#1}%
192 \ifx\caption@tempa\@empty
193 \PackageInfo{caption3}{Option 'parskip' ignored}%
194 \else
195 \caption@KV@parskip{#1}%
196 \fi}%
197 }

```

## Styles

```

\DeclareCaptionStyle \DeclareCaptionStyle{<name>}[<single-line-list-of-KV>]{<list-of-KV>}
198 \newcommand*\DeclareCaptionStyle[1]{%
199 \@ifnextchar[{\caption@declarestyle{#1}}{\caption@declarestyle{#1}[]}}
200 \def\caption@declarestyle#1[#2]#3{%
201 \global\@namedef{caption@sls@#1}{#2}%
202 \global\@namedef{caption@sty@#1}{#3}}
203 \@onlypreamble\DeclareCaptionStyle
204 \@onlypreamble\caption@declarestyle

205 \DeclareCaptionOption{style}{\caption@setstyle{#1}}

\caption@setstyle \caption@setstyle{<name>}
\caption@setstyle*{<name>}

```

Selecting a caption style means saving the additional *<single-line-list-of-KV>* (this will be done by `\caption@sls`), resetting the caption options to the default ones (this will be done using `\caption@setdefault`) and executing the *<list-of-KV>* options (this will be done using `\caption@esetup`).

The starred version will give no error message if the given style is not defined.

```

206 \newcommand\caption@setstyle{%
207 \@ifstar{\caption@@setstyle\@gobble}{\caption@@setstyle\@firstofone}}
208 \newcommand*\caption@@setstyle[2]{%
209 \@ifundefined{caption@sty@#2}%
210 {#1{\caption@Error{Undefined caption style `#2'}}}%
211 {\expandafter\let\expandafter\caption@sls\csname caption@sls@#2\endcsname
212 \caption@setdefault\caption@esetup{\csname caption@sty@#2\endcsname}}}

```

```

\caption@setdefault This resets (nearly) all caption options to the default ones. Note that this does not touch
the skips and the positioning!
213 \newcommand\caption@setdefault{\captionsetup{%
214 format=default,labelformat=default,labelsep=default,textformat=default,%
215 justification=default,font=default,labelfont=default,textfont=default,%
216 margin=0pt,indent=0pt,parindent=0pt,hangindent=0pt,%
217 singlelinecheck=1,strut=1}}

```

Currently there is only one pre-defined style, called 'default'. It's a perfect match to the behaviour of `\@makecaption` offered by the standard L<sup>A</sup>T<sub>E</sub>X document classes: If the caption fits in one single line, it is typeset centered.

```

218 \DeclareCaptionStyle{default}[indent=0pt,justification=centering]{}

```

## Formats

```
\DeclareCaptionFormat \DeclareCaptionFormat{<name>}{<code with #1, #2, and #3>}
\DeclareCaptionFormat*{<name>}{<code with #1, #2, and #3>}
```

The starred form causes the code being typeset in vertical (instead of horizontal) mode, but does not support the `indentation=` option.

```
219 \newcommand\DeclareCaptionFormat{%
220   \@ifstar{\caption@declareformat@gobble}%
221           {\caption@declareformat@firstofone}}
222 \newcommand\caption@declareformat[3]{%
223   \global\expandafter\let\csname caption@ifh@#2\endcsname#1%
224   \global\long\@namedef{caption@fmt@#2}##1##2##3{#3}}
225 \@onlypreamble\DeclareCaptionFormat
226 \@onlypreamble\caption@declareformat

227 \DeclareCaptionOption{format}{\caption@setformat{#1}}
```

```
\caption@setformat \caption@setformat{<name>}
```

Selecting a caption format simply means saving the code (in `\caption@fmt`) and if the code should be used in horizontal or vertical mode (`\caption@ifh`).

```
228 \newcommand*\caption@setformat[1]{%
229   \@ifundefined{caption@fmt@#1}%
230   {\caption@Error{Undefined caption format '#1'}}%
231   {\expandafter\let\expandafter\caption@ifh\csname caption@ifh@#1\endcsname
232   \expandafter\let\expandafter\caption@fmt\csname caption@fmt@#1\endcsname}}
```

There are two pre-defined formats, called ‘plain’ and ‘hang’.

```
233 \DeclareCaptionFormat{plain}{#1#2#3\par}
234 \DeclareCaptionFormat{hang}{%
235   \@hangfrom{#1#2}%
236   \advance\captionparindent\hangindent
237   \advance\captionhangindent\hangindent
238   \caption@@par
239   #3\par}
```

‘default’ usually maps to ‘plain’.

```
240 \def\caption@fmt@default{\caption@fmt@plain}
241 \def\caption@ifh@default{\caption@ifh@plain}
```

## Label formats

```
\DeclareCaptionLabelFormat \DeclareCaptionLabelFormat{<name>}{<code with #1 and #2>}
```

```
242 \newcommand*\DeclareCaptionLabelFormat[2]{%
243   \global\@namedef{caption@lfmt@#1}##1##2{#2}}
244 \@onlypreamble\DeclareCaptionLabelFormat
```

```
245 \DeclareCaptionOption{labelformat}{\caption@setlabelformat{#1}}
```

```

\caption@setlabelformat \caption@setlabelformat{<name>}
Selecting a caption label format simply means saving the code (in \caption@lfmt).
246 \newcommand*\caption@setlabelformat[1]{%
247 \@ifundefined{caption@lfmt@#1}%
248 {\caption@Error{Undefined caption label format `#1'}}%
249 {\expandafter\let\expandafter\caption@lfmt\csname caption@lfmt@#1\endcsname}}

```

There are three pre-defined label formats, called ‘empty’, ‘simple’, and ‘parens’.

```

250 \DeclareCaptionLabelFormat{empty}{}
251 \DeclareCaptionLabelFormat{simple}{\bothIfFirst{#1}{\nobreakspace}#2}
252 \DeclareCaptionLabelFormat{parens}{\bothIfFirst{#1}{\nobreakspace} (#2)}

```

‘default’ usually maps to ‘simple’.

```

253 \def\caption@lfmt@default{\caption@lfmt@simple}

```

### Label separators

```

\DeclareCaptionLabelSeparator \DeclareCaptionLabelSeparator{<name>}{<code>}
\DeclareCaptionLabelSeparator*{<name>}{<code>}
The starred form causes the label separator to be typeset without using \captionlabelfont.

```

```

254 \newcommand\DeclareCaptionLabelSeparator{%
255 \@ifstar{\caption@declarelabelseparator\@gobble}%
256 {\caption@declarelabelseparator\@firstofone}}
257 \newcommand\caption@declarelabelseparator[3]{%
258 \global\expandafter\let\csname caption@iflf@#2\endcsname#1%
259 \global\long\@namedef{caption@lsep@#2}{#3}}
260 \@onlypreamble\DeclareCaptionLabelSeparator
261 \@onlypreamble\caption@declarelabelseparator

262 \DeclareCaptionOption{labelsep}{\caption@setlabelseparator{#1}}
263 \DeclareCaptionOption{labelseparator}{\caption@setlabelseparator{#1}}

```

```

\caption@setlabelseparator \caption@setlabelseparator{<name>}
Selecting a caption label separator simply means saving the code (in \caption@lsep).
264 \newcommand*\caption@setlabelseparator[1]{%
265 \@ifundefined{caption@lsep@#1}%
266 {\caption@Error{Undefined caption label separator `#1'}}%
267 {\expandafter\let\expandafter\caption@iflf\csname caption@iflf@#1\endcsname
268 \expandafter\let\expandafter\caption@lsep\csname caption@lsep@#1\endcsname}}

```

There are seven pre-defined label separators, called ‘none’, ‘colon’, ‘period’, ‘space’, ‘quad’, ‘newline’, and ‘endash’.

```

269 \DeclareCaptionLabelSeparator{none}{}
270 \DeclareCaptionLabelSeparator{colon}{: }
271 \DeclareCaptionLabelSeparator{period}{. }
272 \DeclareCaptionLabelSeparator{space}{ }
273 \DeclareCaptionLabelSeparator*{quad}{quad}
274 \DeclareCaptionLabelSeparator*{newline}{\\}
275 \DeclareCaptionLabelSeparator*{endash}{\space\textendash\space}

```

‘default’ usually maps to ‘colon’.

```
276 \def\caption@lsep@default{\caption@lsep@colon}
277 \def\caption@iflf@default{\caption@iflf@colon}
```

### Text formats

```
\DeclareCaptionTextFormat \DeclareCaptionTextFormat{<name>}{<code with #1>}
```

```
278 \newcommand*\DeclareCaptionTextFormat[2]{%
279   \global\long\@namedef{caption@tfmt@#1}##1{#2}}
280 \@onlypreamble\DeclareCaptionTextFormat
```

```
281 \DeclareCaptionOption{textformat}{\caption@settextformat{#1}}
```

```
\caption@settextformat \caption@settextformat{<name>}
```

Selecting a caption text format simply means saving the code (in \caption@tfmt).

```
282 \newcommand*\caption@settextformat[1]{%
283   \@ifundefined{caption@tfmt@#1}%
284     {\caption@Error{Undefined caption text format `#1'}}%
285     {\expandafter\let\expandafter\caption@tfmt\csname caption@tfmt@#1\endcsname}}
```

There are two pre-defined text formats, called ‘simple’ and ‘period’.

```
286 \DeclareCaptionTextFormat{simple}{#1}
287 \DeclareCaptionTextFormat{period}{#1.}
```

‘default’ usually maps to ‘simple’.

```
288 \def\caption@tfmt@default{\caption@tfmt@simple}
```

### Justifications

```
DeclareCaptionJustification \DeclareCaptionJustification{<name>}{<code>}
```

```
289 \newcommand*\DeclareCaptionJustification[2]{%
290   \global\@namedef{caption@hj@#1}{#2}}
291 %\newcommand\DeclareCaptionJustification{\DeclareCaptionFont}
292 \@onlypreamble\DeclareCaptionJustification
```

```
293 \DeclareCaptionOption{justification}{\caption@setjustification{#1}}
```

```
\caption@setjustification \caption@setjustification{<name>}
```

Selecting a caption justification simply means saving the code (in \caption@hj).

```
294 \newcommand*\caption@setjustification[1]{%
295   \@ifundefined{caption@hj@#1}%
296     {\caption@Error{Undefined caption justification `#1'}}%
297     {\expandafter\let\expandafter\caption@hj\csname caption@hj@#1\endcsname}}
298 %\newcommand\caption@setjustification{\caption@setfont{@hj}}
```

These are the pre-defined justification code snippets.

```
299 \DeclareCaptionJustification{justified}{}
300 \DeclareCaptionJustification{centering}{\centering}
301 \DeclareCaptionJustification{centerfirst}{\centerfirst}
302 \DeclareCaptionJustification{centerlast}{\centerlast}
303 \DeclareCaptionJustification{raggedleft}{\raggedleft}
304 \DeclareCaptionJustification{raggedright}{\raggedright}
```

‘default’ usually maps to ‘justified’.

```
305 \def\caption@hj@default{\caption@hj@justified}
```

`\centerfirst` Please blame Frank Mittelbach for `\caption@centerfirst :-)`

```
306 \providecommand\centerfirst{%
307   \let\\\@centercr
308   \edef\caption@normaladjust{%
309     \leftskip\the\leftskip
310     \rightskip\the\rightskip
311     \parfillskip\the\parfillskip\relax}%
312   \leftskip\z@\@plus -1fil%
313   \rightskip\z@\@plus 1fil%
314   \parfillskip\z@skip
315   \noindent\hskip\z@\@plus 2fil%
316   \@setpar{\@@par\@restorepar\caption@normaladjust}}
```

`\centerlast` This is based on code from Anne Brüggemann-Klein[12]

```
317 \providecommand\centerlast{%
318   \let\\\@centercr
319   \leftskip\z@\@plus 1fil%
320   \rightskip\z@\@plus -1fil%
321   \parfillskip\z@\@plus 2fil\relax}
```

We also support the upper-case commands offered by the `ragged2e` package. Note that these just map to their lower-case variants if the `ragged2e` package is not available.

```
322 \DeclareCaptionJustification{Centering}{%
323   \caption@ragged\Centering\centering}
324 \DeclareCaptionJustification{RaggedLeft}{%
325   \caption@ragged\RaggedLeft\raggedleft}
326 \DeclareCaptionJustification{RaggedRight}{%
327   \caption@ragged\RaggedRight\raggedright}
```

`\caption@ragged` `\caption@ragged` will be basically defined as

```
\AtBeginDocument{\IfFileExists{ragged2e.sty}%
  {\RequirePackage{ragged2e}\let\caption@ragged\@firstoftwo}%
  {\let\caption@ragged\@secondoftwo}}
```

but with an additional warning if the `ragged2e` package is not loaded (yet). (This warning will be typeout only one time per option, that’s why we need the `\caption\string#1` stuff.) Furthermore we load the `ragged2e` package, if needed and available.

```
328 \newcommand*\caption@ragged{%
```

```

329 \caption@Debug{We need ragged2e}%
330 \protected@write\@auxout{}\string\caption@newlabel{ragged2e}{}%
331 \global\let\caption@ragged\caption@@ragged
332 \caption@@ragged}

333 \newcommand*\caption@@ragged[2]{%
334 \@ifundefined{caption\string#1}{%
335 \PackageWarning{caption3}{%
336 `ragged2e' package not loaded, therefore\MessageBreak
337 substituting \string#2 for \string#1\MessageBreak}%
338 \global\@namedef{caption\string#1}{}%
339 #2}

340 \AtBeginDocument{%
341 \@ifundefined{caption@ragged2e}{%
342 \let\caption@@ragged\@secondoftwo % suppress warning above
343 }{%
344 \caption@Debug{We load ragged2e}%
345 \IfFileExists{ragged2e.sty}{%
346 \RequirePackage{ragged2e}\let\caption@@ragged\@firstoftwo}{}%
347 }}

```

## Fonts

```

\DeclareCaptionFont \DeclareCaptionFont {<name>} {<code>}
348 \newcommand\DeclareCaptionFont [2]{%
349 \define@key{caption@fnt}{#1}[]{\g@addto@macro\caption@tempa{#2}}
350 \@onlypreamble\DeclareCaptionFont

351 \DeclareCaptionOption{font}{\caption@setfont{font}{#1}}
352 \DeclareCaptionOption{labelfont}{\caption@setfont{labelfont}{#1}}
353 \DeclareCaptionOption{textfont}{\caption@setfont{textfont}{#1}}

\caption@setfont \caption@setfont {<name>} {<keyval-list of names>}
Selecting a caption font means saving all the code snippets (in \caption#1). Because we use \setkeys recursive here we need to do this inside an extra group and collect all the code snippets in \caption@tempa first.
354 \newcommand*\caption@setfont [2]{%
355 \let\caption@tempa\@empty
356 \begingroup
357 % \define@key{caption@fnt}{default}[]{%
358 % \global\expandafter\let\expandafter\caption@tempa
359 % \csname caption#1@default\endcsname}%
360 \caption@setkeys[caption]{caption@fnt}{#2}%
361 \endgroup
362 \expandafter\let\csname caption#1\endcsname\caption@tempa}

363 \DeclareCaptionFont{default}{}

These are the pre-defined font code snippets.
364 \DeclareCaptionFont{scriptsize}{\scriptsize}

```

```

365 \DeclareCaptionFont{footnotesize}{\footnotesize}
366 \DeclareCaptionFont{small}{\small}
367 \DeclareCaptionFont{normalsize}{\normalsize}
368 \DeclareCaptionFont{large}{\large}
369 \DeclareCaptionFont{Large}{\Large}

370 \DeclareCaptionFont{up}{\upshape}
371 \DeclareCaptionFont{it}{\itshape}
372 \DeclareCaptionFont{sl}{\slshape}
373 \DeclareCaptionFont{sc}{\scshape}
374 \DeclareCaptionFont{md}{\mdseries}
375 \DeclareCaptionFont{bf}{\bfseries}
376 \DeclareCaptionFont{rm}{\rmfamily}
377 \DeclareCaptionFont{sf}{\sffamily}
378 \DeclareCaptionFont{tt}{\ttfamily}

```

### setspace package support

```

379 \DeclareCaptionFont{singlespacing}{\setstretch{\setspace@singlespace}}% normally 1
380 \DeclareCaptionFont{onehalfspacing}{\onehalfspacing}
381 \DeclareCaptionFont{doublespacing}{\doublespacing}

```

`\captionsize` The old versions `v1.x` of the caption package offered this command to setup the font size used for captions. We still do so old documents will work fine.

```

382 \providecommand\captionsize{}

383 \DeclareCaptionOption{size}{\caption@setfont{size}{#1}}

```

### Vertical spaces before and after captions

`\abovecaptionskip` Usually these skips are defined within the document class, but some document classes  
`\belowcaptionskip` don't do so.

```

384 \@ifundefined{abovecaptionskip}{%
385   \newlength\abovecaptionskip\setlength\abovecaptionskip{10\p@}}{}
386 \@ifundefined{belowcaptionskip}{%
387   \newlength\belowcaptionskip\setlength\belowcaptionskip{0\p@}}{}

388 \DeclareCaptionOption{aboveskip}{\setlength\abovecaptionskip{#1}}
389 \DeclareCaptionOption{belowskip}{\setlength\belowcaptionskip{#1}}
390 \DeclareCaptionOption{skip}{\setlength\abovecaptionskip{#1}}

```

### Positioning

These macros handle the right position of the caption. Note that the position is actually *not* controlled by the caption kernel options, but by the user (or a specific package like the float package) instead. The user can put the `\caption` command wherever he likes! So this stuff is only to give us a *hint* where to put the right skips, the user usually has to take care for himself that this hint actually matches the right position. The user can also try out the experimental setting `position=auto` which means that the caption package should try to guess the actual position of the caption for himself. (But in many cases, for

example in longtables, this is doomed to fail, so it's not documented in the user part of the documentation.)

```
391 \DeclareCaptionOption{position}{\caption@setposition{#1}}
```

```
\caption@setposition \caption@setposition{<position>}
```

Selecting the caption position means that we put `\caption@position` to the right value. *Please do not use the internal macro `\caption@position` in your own package or document, but use the wrapper macro `\caption@iftop` instead.*

```
392 \newcommand*\caption@setposition[1]{%
393   \caption@ifinlist{#1}{d,default}{%
394     \def\caption@position{\caption@defaultpos}%
395   }{\caption@ifinlist{#1}{t,top,above}{%
396     \let\caption@position\@firstoftwo
397   }{\caption@ifinlist{#1}{b,bottom,below}{%
398     \let\caption@position\@secondoftwo
399   }{\caption@ifinlist{#1}{a,auto}{%
400     \let\caption@position\@undefined
401   }{%
402     \caption@Error{Undefined caption position `#1'}%
403   }}}}
```

```
\caption@defaultpos
```

The default 'position' is usually 'bottom', this means that the (larger) skip will be typeset above the caption. This corresponds to the `\@makecaption` implementation in the standard L<sup>A</sup>T<sub>E</sub>X document classes.

```
404 %\caption@setdefaultpos{b}% default = bottom
405 \let\caption@defaultpos\@secondoftwo
```

```
\caption@iftop \caption@iftop{<true-code>}{<false-code>}
(If the position= is set to auto we assume a bottom position.)
```

```
406 \newcommand\caption@iftop{%
407   \ifx\caption@position\@undefined
408     \expandafter\@secondoftwo
409   \else
410     \expandafter\caption@position
411   \fi}
```

```
\caption@fixposition \caption@fixposition
```

This macro checks if the 'position' is set to 'auto'. If yes, `\caption@autoposition` will be called to set `\caption@position` to a proper value we can actually use.

```
412 \newcommand\caption@fixposition{%
413   \ifx\caption@position\@undefined
414     \caption@autoposition
415   \fi}
```

```
\caption@autoposition \caption@autoposition
```

We guess the actual position of the caption by checking `\prevdepth`.

```
416 \newcommand\caption@autoposition{%
417   \ifvmode
```

```

418 \edef\caption@tempa{\the\prevdepth}%
419 \caption@Debug{\protect\prevdepth=\caption@tempa}%
420 % \caption@setposition{\ifdim\prevdepth>-\p@ b\else t\fi}%
421 \ifdim\prevdepth>-\p@
422 \let\caption@position\@secondoftwo
423 \else
424 \let\caption@position\@firstoftwo
425 \fi
426 \else
427 \caption@Debug{no \protect\prevdepth}%
428 % \caption@setposition{b}%
429 \let\caption@position\@secondoftwo
430 \fi}

```

### Hooks

```

\AtBeginCaption \AtBeginCaption {code}
\AtEndCaption \AtEndCaption {code}

```

These hooks can be used analogous to `\AtBeginDocument` and `\AtEndDocument`.

```

431 \newcommand\caption@beginhook{}
432 \newcommand\caption@endhook{}
433 \newcommand\AtBeginCaption{\l@addto@macro\caption@beginhook}
434 \newcommand\AtEndCaption{\l@addto@macro\caption@endhook}

```

### Miscellaneous options

```

435 \DeclareCaptionOption{listof}{\caption@setbool{lof}{#1}}
436 \DeclareCaptionOption{singlelinecheck}{\caption@setbool{slc}{#1}}
437 \DeclareCaptionOption{strut}{\caption@setbool{strut}{#1}}

```

### Debug option

```

438 \DeclareCaptionOption{debug}[1]{%
439 \caption@setbool{debug}{#1}%
440 \caption@ifdebug{%
441 \def\caption@Debug{\PackageInfo{caption3}}%
442 }{%
443 \let\caption@Debug\@gobble
444 }}
445 \setkeys{caption}{debug=0}

```

### Initialization of parameters

```

446 \captionsetup{style=default,position=default,listof=1,%
447 twoside=\if@twoside 1\else 0\fi}

```

`\ifcaption@star` If the starred form of `\caption` is used, this will be set to `true`. (It will be reset to `false` at the end of `\caption@@make`.)

```

448 \newif\ifcaption@star

```

### Typesetting the caption

```
\caption@make \caption@make{<float name>}{<ref. number>}{<text>}
449 \newcommand\caption@make[2]{%
450 \caption@@make{\caption@lfmt{#1}{#2}}}
```

```
\caption@@make \caption@@make{<caption label>}{<caption text>}
451 \newcommand\caption@@make[2]{%
452 \beginingroup
453 \caption@beginhook
454 \caption@calcmargin
```

#### Special single-line treatment (option singlelinecheck=)

```
455 \caption@ifslc{\ifx\caption@sls\@empty\else
456 \caption@slc{#1}{#2}\captionwidth\relax
457 \fi}{}%
```

#### Typeset the left margin (option margin=)

```
458 \@tempdima\captionmargin
459 \ifdim\captionmargin@=\z@\else
460 \caption@ifoddpagel{\advance\@tempdima\captionmargin@}%
461 \fi
462 \caption@ifh{\advance\@tempdima\captionindent}%
463 \hskip\@tempdima
```

We actually use a `\vbox` of width `\captionwidth - \captionindent` to typeset the caption (Note: `\captionindent` is *not* supported if the caption format was defined with `\DeclareCaptionFormat*`.)

```
464 \@tempdima\captionwidth
465 \caption@ifh{\advance\@tempdima by -\captionindent}%
466 \captionbox\@tempdima{%
```

#### Typeset the indentation (option indention=)

Bugfix 04-05-05: `\hskip-\captionindent` replaced by `\ifdim\captionindent=\z@...`

```
467 \caption@ifh{%
468 \ifdim\captionindent=\z@
469 \leavevmode
470 \else
471 \hskip-\captionindent
472 \fi}%
```

#### Typeset the caption itself and close the `\captionbox`

```
473 \caption@@@make{#1}{#2}}%
```

#### Typeset the right margin (option margin=)

```
474 \@tempdima\captionmargin
475 \ifdim\captionmargin@=\z@\else
476 \caption@ifoddpagel{\advance\@tempdima\captionmargin@}{}%
477 \fi
478 \hskip\@tempdima
```

```

479 \caption@endhook
480 \endgroup
481 \global\caption@starfalse}

\caption@calcmargin Calculate \captionmargin & \captionwidth, so both contain valid values.
482 \newcommand\caption@calcmargin{%
Note: Inside a list environment \linewidth do not contain the proper value, be-
cause \@caption calls \@parboxrestore which resets \linewidth to \hsize.
Therefore we have to calculate the proper line width on our own in this case.
483 \@tempdima\hsize
484 \ifnum\@listdepth>0\relax
485 \advance\@tempdima by -\leftmargin
486 \advance\@tempdima by -\rightmargin
487 \fi
488 \ifdim\captionwidth=\z@
489 \captionwidth\@tempdima
490 \advance\captionwidth by -2\captionmargin
491 \advance\captionwidth by -\captionmargin@
492 \else
493 \captionmargin\@tempdima
494 \advance\captionmargin by -\captionwidth
495 \divide\captionmargin by 2
496 \captionmargin@\z@
497 \fi
498 \caption@Debug{%
499 \protect\hsize=\the\hsize,
500 \protect\margin=\the\captionmargin,
501 \protect\marginx=\the\captionmargin@,
502 \protect\width=\the\captionwidth}%
503 }

\caption@slc This one does the single-line-check.
504 \newcommand\caption@slc[4]{%
505 \caption@startslc
506 \sbox\@tempboxa{\caption@@@make{#1}{#2}}%
507 \ifdim\wd\@tempboxa >#3%
508 \caption@endslc
509 \else
510 \caption@endslc
511 \caption@esetup\caption@sls
512 #4%
513 \fi}

\caption@startslc Re-define anything which would disturb the single-line-check.
514 \newcommand\caption@startslc{%
515 \begingroup
516 \let\label\@gobble

```

```

517 \let\@footnotetext\@gobble\let\@endnotetext\@gobble
518 \def\stepcounter##1{\advance\c@##1\endcsname\@ne\relax}%
519 \let\caption@hj\relax}

\caption@endslc This ends the single-line-check.
520 \newcommand\caption@endslc{%
521 \endgroup}

\captionbox This macro defines the box which surrounds the caption paragraph.
522 \newcommand\captionbox{\parbox[b]}

\caption@@@make \caption@@@make{<caption label>}{<caption text>}
This one finally typesets the caption paragraph, without margin and indentation.
523 \newcommand\caption@@@make[2]{%
If the label is empty, we use no caption label separator.
524 \sbox\@tempboxa{#1}%
525 \ifdim\wd\@tempboxa=\z@
526 \let\caption@lsep\relax
527 \fi

If the text is empty, we use no caption label separator, too.
528 \caption@ifempty{#2}{%
529 \let\caption@lsep\relax
530 % \let\caption@ifstrut\@secondoftwo
531 }%

Take care that \captionparindent and \captionhangindent will be used to
typeset the paragraph.
532 \@setpar{\@@par\caption@@par}\caption@@par

Finally the caption will be typeset.
533 \caption@hj\captionsize\captionfont\caption@fmt
534 {\ifcaption@star\else{\captionlabelfont#1}\fi}%
535 {\ifcaption@star\else{\caption@iflf\captionlabelfont\caption@lsep}\fi}%
536 {\captiontextfont
537 \caption@ifstrut{\vrule\@height\ht\strutbox\@width\z@}{}}%
538 \nobreak\hskip\z@skip
539 \caption@tfmt{#2}%
540 % \caption@ifstrut{\vrule\@height\z@\@depth\dp\strutbox\@width\z@}{}}%
541 \caption@ifstrut{\@finalstrut\strutbox}{}}%
542 \par}}

\caption@ifempty \caption@ifempty{<text>}{<if-clause>}
This one tests if the <text> is actually empty.
Note: This will be done without expanding the text, therefore this is far away from being
bullet-proof.
543 \newcommand\caption@ifempty[1]{%
544 \def\caption@tempa{#1}%

```

```

545 \def\caption@tempb{\ignorespaces}%
546 \ifx\caption@tempa\caption@tempb
547   \let\caption@tempa\@empty
548 \fi
549 \ifx\caption@tempa\@empty
550   \expandafter\@firstofone
551 \else
552   \expandafter\@gobble
553 \fi}

```

`\caption@@par` `\caption@@par`

This command will be executed with every `\par` inside the caption.

```

554 \newcommand*\caption@@par{%
555   \parindent\captionparindent\hangindent\captionhangindent}%

```

### subfig package support

This is a very small bugfix for v1.2 and v1.3 or the subfig package, making `\subfig` robust. I do this here because it's caption related stuff and I get all the bug reports ;-)

```

556 \AtBeginDocument{%
557   \def\@tempa{\@ifstar\sf@@subref\sf@subref}%
558   \ifx\subref\@tempa
559     \PackageInfo{caption3}{subref 1.2 or 1.3 detected}%
560     \DeclareRobustCommand*\subref{\@ifstar\sf@@subref\sf@subref}%
561   \fi
562 }

```

## 11.2 Main package

### Identification

```

563 \NeedsTeXFormat{LaTeX2e}[1994/12/01]
564 \ProvidesPackage{caption}[2007/04/16 v3.0q Customising captions (AR)]

```

### Loading the kernel

```

565 \RequirePackage{caption3}[2007/01/31] % needs v3.01 or newer

```

### Check against the obsolete caption2 package

```

566 \@ifpackageloaded{caption2}{%
567   \caption@Error{You can't use both the caption *and* caption2 package}%
568   \endinput
569 }{}

```

### Option for configuration files

```

570 \DeclareCaptionOption{config}[caption]{%
571   \InputIfFileExists{#1.cfg}{\typeout{*** Local configuration file
572     #1.cfg used ***}}%
573   {\PackageWarning{caption}{Configuration

```

574

file #1.cfg not found}}

### Options for figure and table

```
575 \DeclareCaptionOption*{figureposition}{\captionsetup[figure]{position=#1}}
576 \DeclareCaptionOption*{tableposition}{\captionsetup[table]{position=#1}}
577 \DeclareCaptionOption*{figurename}{\captionsetup[figure]{name=#1}}
578 \DeclareCaptionOption*{tablename}{\captionsetup[table]{name=#1}}
```

### caption v1.x compatibility options

```
579 \DeclareCaptionOption*{normal}[]{\caption@setformat{normal}}
580 \DeclareCaptionOption*{isu}[]{\caption@setformat{hang}}
581 \DeclareCaptionOption*{hang}[]{\caption@setformat{hang}}
582 \DeclareCaptionOption*{center}[]{\caption@setjustification{centering}}
583 \DeclareCaptionOption*{anne}[]{\caption@setjustification{centerlast}}
584 \DeclareCaptionOption*{centerlast}[]{\caption@setjustification{centerlast}}

585 \DeclareCaptionOption*{scriptsize}[]{\def\captionfont{\scriptsize}}
586 \DeclareCaptionOption*{footnotesize}[]{\def\captionfont{\footnotesize}}
587 \DeclareCaptionOption*{small}[]{\def\captionfont{\small}}
588 \DeclareCaptionOption*{normalsize}[]{\def\captionfont{\normalsize}}
589 \DeclareCaptionOption*{large}[]{\def\captionfont{\large}}
590 \DeclareCaptionOption*{Large}[]{\def\captionfont{\Large}}

591 \DeclareCaptionOption*{up}[]{\l@addto@macro\captionlabelfont\upshape}
592 \DeclareCaptionOption*{it}[]{\l@addto@macro\captionlabelfont\itshape}
593 \DeclareCaptionOption*{sl}[]{\l@addto@macro\captionlabelfont\slshape}
594 \DeclareCaptionOption*{sc}[]{\l@addto@macro\captionlabelfont\scshape}
595 \DeclareCaptionOption*{md}[]{\l@addto@macro\captionlabelfont\mdseries}
596 \DeclareCaptionOption*{bf}[]{\l@addto@macro\captionlabelfont\bfseries}
597 \DeclareCaptionOption*{rm}[]{\l@addto@macro\captionlabelfont\rmfamily}
598 \DeclareCaptionOption*{sf}[]{\l@addto@macro\captionlabelfont\sffamily}
599 \DeclareCaptionOption*{tt}[]{\l@addto@macro\captionlabelfont\ttfamily}

600 \DeclareCaptionOption*{nooneline}[]{\caption@setbool{slc}{0}}
601 \caption@setbool{ruled}{0}
602 \DeclareCaptionOption*{ruled}[]{\caption@setbool{ruled}{1}}
```

### Some caption2 v2.x compatibility options

```
603 \DeclareCaptionOption*{flushleft}[]{\caption@setjustification{raggedright}}
604 \DeclareCaptionOption*{flushright}[]{\caption@setjustification{raggedleft}}
605 \DeclareCaptionOption*{oneline}[]{\caption@setbool{slc}{1}}
606 \DeclareCaptionOption*{ignoreLTcapwidth}[]{}
```

### Some KOMA-Script compatibility options

```
607 \DeclareCaptionOption*{onelinecaption}[]{\caption@setbool{slc}{1}}
608 \DeclareCaptionOption*{noonelinecaption}[]{\caption@setbool{slc}{0}}
609 \DeclareCaptionOption*{tablecaptionabove}[]{\captionsetup[table]{position=t}}
610 \DeclareCaptionOption*{tablecaptionbelow}[]{\captionsetup[table]{position=b}}
```

### Generic package support

```
\caption@declarepackage \caption@declarepackage{<package name>}
```

Each single package support can be switched on or off by using the appropriate option. By default all of them are enabled.

```
611 \newcommand*\caption@declarepackage[1]{%
612   \caption@setbool{pkt@#1}{1}%
613   \DeclareCaptionOption*{#1}{\caption@setbool{pkt@#1}{##1}}
614 \AtEndOfPackage{\let\caption@declarepackage\@undefined}
```

```
\caption@ifpackage \caption@ifpackage{<package name>}{<package macro>}{<code>}
```

If a certain package support is requested the appropriate code will be used. ‘Requested’ means that the option belonging to it is set to true and the macro called *<package macro>* is defined. (If *<package macro>* is not yet defined we use `\AtBeginDocument` here, so the package could be loaded after this package, too.)

```
615 \newcommand\caption@ifpackage[3]{%
616   \edef\caption@tempa{%
617     \caption@ifbool{pkt@#1}%
618     {\@ifundefined{#2}{AtBeginDocument}{firstofone}}%
619     {gobble}}%
620   \caption@Info{#1=\caption@ifbool{pkt@#1}{1}{0} %
621     {\@ifundefined{#2}{not }{}}loaded->\caption@tempa}%
622   \caption@ifbool{pkt@#1}{%
623     \@ifundefined{#2}%
624     {\let\caption@tempa\AtBeginDocument}%
625     {\let\caption@tempa\@firstofone}%
626   }{%
627     \let\caption@tempa\@gobble
628   }%
629   \caption@tempa{\@ifundefined{#2}{}{#3}}%
630   \caption@undefbool{pkt@#1}}
631 \AtEndOfPackage{\let\caption@ifpackage\@undefined}
```

You can also switch the caption support off using the package option `caption=false`. This may look strange, but there are certain circumstances where this could be useful. Such a situation might be the usage of the `subfig` package without disturbing the main caption code of the document class.

*Note: This mechanism is obsolete now, it has been superseded by the `subfig` package option `caption=false` which causes that only the caption kernel `caption3` is loaded.*

```
632 \caption@declarepackage{caption}
```

These are the packages we support:

```
633 \caption@declarepackage{float}
634 \caption@declarepackage{floatrow}
635 \caption@declarepackage{hyperref}
636 \caption@declarepackage{hypcap}
637 \caption@declarepackage{listings}
638 \caption@declarepackage{longtable}
639 \caption@declarepackage{picins}
640 \caption@declarepackage{rotating}
```

```
641 \caption@declarepackage{sidecap}
642 \caption@declarepackage{supertabular}
```

### Processing of options

```
643 \DeclareCaptionOption{verbose}[1]{%
644   \caption@setbool{verbose}{#1}%
645   \caption@ifverbose{%
646     \def\caption@Info{\PackageInfo{caption}}%
647   }{%
648     \let\caption@Info@gobble
649   }}
650 \setkeys{caption}{verbose=0}
651 \caption@ProcessOptions{caption}
```

If the option `caption=false` was given we stop processing this file immediately.

```
652 \caption@ifbool{pkt@caption}{}{\endinput}
653 \caption@undefbool{pkt@caption}
```

### Useful stuff

```
\captionof \captionof(*){<type>}[<lst_entry>]{<heading>}
654 \def\captionof{\@ifstar{\caption@of{\caption*}}{\caption@of\caption}}
655 \newcommand*\caption@of[2]{\def\@capytype{#2}#1}
```

Note: Like `\captionof` the option `type=` should only be used inside a group or environment and does not check if the argument is a valid floating environment or not.

```
656 \DeclareCaptionOption{name}{\caption@setfloatname\@capytype{#1}}
657 \DeclareCaptionOption{type}{\def\@capytype{#1}}
```

```
\ContinuedFloat \ContinuedFloat[<type>]
```

This mainly decreases the appropriate counter by  $-1$ .

```
658 \providecommand\ContinuedFloat{%
659   \@ifnextchar[%]
660     \@ContinuedFloat
661     {\ifx\@capytype\undefined
662       \latex@error{\noexpand\ContinuedFloat outside float}\@ehd
663     \else
664       \@ContinuedFloat[\@capytype]%
665     \fi}}
666 \def\@ContinuedFloat[#1]{%
667   \addtocounter{#1}\m@ne
668   \caption@ContinuedFloat{#1}%
669   \caption@@ContinuedFloat{#1}}
```

```
\caption@ContinuedFloat \caption@ContinuedFloat{<type>}
\caption@resetContinuedFloat \caption@resetContinuedFloat{<type>}
```

The first one will be called inside `\ContinuedFloat`, the second one inside `\caption`. Usually they do nothing but this changes if the `hyperref` package is loaded. (See `hyperref` package support for details.)

```
670 \let\caption@ContinuedFloat\@gobble
671 \let\caption@resetContinuedFloat\@gobble
```

`\caption@@ContinuedFloat` This hook is for foreign packages which link themselves into `\ContinuedFloat`, for example the `subfig` package[10].

```
672 \providecommand*\caption@@ContinuedFloat[1]{} }
```

### Internal helpers

`\caption@begin` Our handling of `\caption` will always be surrounded by `\caption@begin` (or `\caption@beginex`) and `\caption@end`.  
`\caption@begin{<type>}` performs these tasks:

- Call `\caption@resetContinuedFloat` (see above) and start a new group
- Execute the options set with `\captionsetup[<type>]`
- Define `\fnum{<type>}` if the caption label format is set to non-default
- Override the `position=` setting, if necessary (for example if set to `auto` or used inside a `supertabular`)

```
673 \newcommand*\caption@begin[1]{%
674   \caption@resetContinuedFloat{#1}%
675   \begingroup
676   \caption@setfloattype{#1}%
677   \ifx\caption@lfmt\caption@lfmt@default\else
678     \@namedef{fnum@#1}{%
679       \caption@lfmt{\caption@floatname{#1}}{\@nameuse{the#1}}}%
680   \fi
681   \caption@fixposition
682   \global\let\caption@fixedposition\caption@position}
```

`\caption@beginex` `\caption@beginex{<type>}{<list entry>}{<heading>}`  
performs the same tasks as `\caption@begin` and additionally: Redefine `\addcontentsline` if no list-of entry is requested, that means either the argument `<list entry>` is empty or `listof=` was set to `false`.

```
683 \newcommand\caption@beginex[3]{%
684   \caption@begin{#1}%
685   \caption@iflof%
686     {\def\caption@tempa{#2}}%
687     {\let\caption@tempa\@empty}%
688   \ifx\caption@tempa\@empty
689     \long\def\addcontentsline##1##2##3{% There is no \@gobblethree...
690   \fi
691   \caption@ifempty{#3}{\let\caption@ifempty\@secondoftwo}%
692 }
```

```

\caption@end \caption@end closes the group.
693 \newcommand*\caption@end{%
694   \endgroup
695   \let\caption@position\caption@fixedposition}

```

```

\caption@setfloattype \caption@setfloattype{<type>}
sets up the right float type within \@caption, \LT@makecaption etc. Usually this
is equivalent to \caption@settype but I made it an own macro so I can extend it
later on, for example if the float or sidecap package is loaded.
696 \let\caption@setfloattype\caption@settype

```

```

\caption@letfloattype \caption@letfloattype{<type>}{<extra code>}
redefines \caption@setfloattype so it does not only \caption@settype{<type>}
but two additional tasks: Executing extra code given as second argument and execute op-
tions with \caption@settype{#1} afterwards.
You can find an example of its usage in the longtable support, where this macro is
called so \captionsetup[longtable]{...} can be used to setup options for
longtables which have a higher priority than the options which have been setup with
\captionsetup[table]{...} or \setlength\LTcapwidth{...}.
697 \newcommand*\caption@letfloattype[2]{%
698   \def\caption@setfloattype##1{%
699     \caption@settype{##1}#2\caption@settype{##1}}

```

```

\caption@floatname \caption@floatname{<type>}
Usually all float names (which partly build the caption label) follow the same naming
convention. But some packages (for example the float package) do not, so we use this
wrapper macro which can be changed later on.
700 \newcommand*\caption@floatname[1]{\@nameuse{#1name}}
701 \newcommand*\caption@setfloatname[1]{\@namedef{#1name}}

```

### Caption support

Some packages (like the hyperref package for example) redefines `\caption` and `\@caption`, too, but without chaining to their previous definitions. So we have to use `\AtBeginDocument` here, so we can make sure our definition don't get lost.

```
702 \AtBeginDocument{%
```

We only patch `\caption` and `\@caption` if the `captcont` package (which brings it's own definition of `\caption*`) is not used. It does not make much sense using the actual version of the `caption` package with the `captcont` package, but this was different in the old (`v1.x`) days so we take care to be backward compatible.

```
703   \@ifundefined{cc@caption}{%
704     \@ifundefined{caption@old}{%

```

```

\caption Here comes our definition of \caption and \caption*. (We set \caption@starttrue
globally so it works with the sidecap package, too.)

```

```

705 \let\caption@old\caption
706 \def\caption{\caption@caption\caption@old}%
707 \def\caption@caption#1{%
708   \ifstar{\ContinuedFloat\global\caption@startrue#1[]}{#1}}%

```

\caption Our definition of \caption simply calls the old definition, nested by \caption@beginex and \caption@end.

```

709 \let\caption@@old\caption
710 \long\def\caption#1[#2]#3{%
711   \caption@beginex{#1}{#2}{#3}%
712   \caption@@old{#1}[{#2}]{#3}%
713   \caption@end}%

```

```
714 }{}{}%
```

**Minimum captcont package support:**

We define \caption@caption here so it's there but does not make any harm.

```

715 \caption@Info{captcont package v2.0 detected}%
716 \def\caption@caption#1{#1}%
717 }%
718 }

```

\makecaption \@makecaption{<label>}{<text>}

The original code (from latex/base/classes.dtx):

```

\long\def\makecaption#1#2{%
  \vskip\abovecaptionskip
  \sbox\@tempboxa{#1: #2}%
  \ifdim \wd\@tempboxa >\hsize
    #1: #2\par
  \else
    \global \@minipagefalse
    \hb@xt@\hsize{\hfil\box\@tempboxa\hfil}%
  \fi
  \vskip\belowcaptionskip}

```

We do basically the same, but take care of the position= setting and use \caption@@make from the caption kernel to actually typeset the caption.

```

719 \renewcommand\makecaption[2]{%
720   \caption@iftop{\vskip\belowcaptionskip}{\vskip\abovecaptionskip}%
721   \caption@@make{#1}{#2}%
722   \caption@iftop{\vskip\abovecaptionskip}{\vskip\belowcaptionskip}}

```

**KOMA-Script classes support**

```

723 \@ifundefined{scr@caption}{}{%
724   \caption@Info{KOMA-Script class detected}
725   \AtBeginDocument{\let\scr@caption\caption}

```

```

\onelinecaptionsfalse
\onelinecaptionstrue 726 \def\onelinecaptionstrue{\caption@setbool{slc}{1}}
727 \def\onelinecaptionsfalse{\caption@setbool{slc}{0}}

\captionabove Original code:
\captionbelow \newcommand{\captionabove}{\@captionabovetrue\scr@caption}
\newcommand{\captionbelow}{\@captionabovefalse\scr@caption}

728 \def\captionabove{%
729 \caption@setposition{t}\let\caption@setposition\@gobble
730 \scr@caption}
731 \def\captionbelow{%
732 \caption@setposition{b}\let\caption@setposition\@gobble
733 \scr@caption}

734 }

french(1e) package support

735 \AtBeginDocument{\@ifundefined{f@ffrench}}{%
736 \caption@Info{french(1e) package detected}%

If \GOfrench is defined as \relax all the re-definitions regarding captions have already been done, so we can do our patches immediately. Otherwise we must add our stuff to \GOfrench.

737 \@ifundefined{GOfrench}%
738 {\let\caption@tempa\@firstofone}%
739 {\def\caption@tempa{\g@addto@macro\GOfrench}}%
740 \caption@tempa%

\@cnORI We update the definition of \@cnORI so it actually reflects our definition of \caption.
741 \let\@cnORI\caption

\@tablescaption The french(1e) package sets \caption to \@tablescaption at \begin{table} for special treatment of footnotes. Therefore we have to patch \@tablescaption so \caption* will work inside the table environment.

742 \let\caption@tablescaption\@tablescaption
743 \def\@tablescaption{\caption@caption\caption@tablescaption}%

\ffrench \ffrench and \ftfrench reflect \fnum@figure and \fnum@table when
\ftfrench used in french mode. These contain additional code which typesets the caption separator \captionseparator instead of the usual colon. Because this breaks with our \@makecaption code we have to remove this additional code here.

744 \let\@eatDP\@undefined
745 \let\caption@tempa\@empty
746 \ifx\ffrench\fnum@figure
747 \l@addto@macro\caption@tempa{\let\fnum@figure\ffrench}%
748 \fi

```

```

749 \ifx\floatfrench\fnun@table
750 \l@addto@macro\caption@tempa{\let\fnun@table\floatfrench}%
751 \fi
752 \def\floatfrench{\ifx\listoffigures\relax\else\figurename~\thefigure\fi}%
753 \def\floatfrench{\ifx\listoftables\relax\else\tablename~\thetable\fi}%
754 \caption@tempa
755 }}}

```

### float package support

The float package usually do not use the L<sup>A</sup>T<sub>E</sub>X kernel command `\caption` to typeset the caption but `\float@caption` instead. (`\caption` will only be used if the float is re-styled with `\restylefloat*`.)

The main two things `\float@caption` is doing different are:

- The caption will be typeset inside a savebox called `\float@capt` so it can be placed above or below the float contents afterwards.
- `\makecaption` will not be used to finally typeset the caption. Instead `\float@capt` will be used which definition is part of the float style. (Note that `\float@capt` will not typeset any vertical space above or below the caption; instead this space will be typeset by the float style code itself.)

So our main goal is to re-define `\float@caption` so our macro `\caption@make` will be used instead of `\float@capt`.

To allow different caption styles for different float styles we will also determine the current float style (e.g. ‘ruled’) at run time and select a caption style (and additional settings) with the same name, if defined.

`\caption@setfloatposition` First of all we provide a macro which converts `\float@iftopcapt` (which is part of a float style and controls where the caption will be typeset, above or below the float contents) to our `position=` setting. Since the spacing above and below the caption will be done by the float style and *not* by us this sounds quite useless. But in fact it isn’t, since some packages based on the caption package (like the subfig package) could have an interest for this information and therefore use the `\caption@iftop` macro we provide in our kernel. Furthermore we need this information for ourself in `\captionof` which uses `\makecaption` to finally typeset the caption with skips.

```

756 \def\caption@setfloatposition{%
757 \caption@setposition{\float@iftopcapt t\else b\fi}}
758 \caption@ifpackage{float}{\float@setevery}{%
759 \caption@Info{float package v1.3 (or newer) detected}%

```

Since `\float@caption` puts the float contents into a savebox we need a special version of `\captionof` which ‘unfolds’ this box afterwards, so the caption actually gets typeset. Furthermore we have to typeset the spacing above and below the caption for ourself, since this space is not part of the box.

Please note that this version of `\captionof` only works *outside* floating environments defined with the float package, so for example a `\captionof{Program}` used within a ‘standard’ figure or a `minipage` will work fine, but not within a re-styled figure or an Example environment defined with `\newfloat`. (We don’t check for this so you’ll get wired errors if you try to do so!)

`\captionof@float` Usually no special action is necessary, so we define `\captionof@float` to `\@gobble`. We will redefine it later on to `\@firstofone` to activate the code which ‘unfolds’ the savebox.

```
760 \let\captionof@float\@gobble
```

`\captionof` If the float is defined by the float package (which means `\fst@{type}` is defined) we activate the special treatment for such captions typeset with `\captionof`. Furthermore we ‘execute’ this float style, so `\@fs@iftopcapt` is set to its proper value.

```
761 \renewcommand*\captionof[2]{%
762   \@ifundefined{fst@#2}{}{%
763     \let\captionof@float\@firstofone
764     \@nameuse{fst@#2}\@float@setevery{#2}}%
765   \def\@capytype{#2}#1}%
```

`\float@caption` Our version of `\float@caption` nearly looks like our version of `\@caption`. The main differences are that `\@fs@capt` will be replaced by our `\caption@@make` and that the savebox called `\@floatcapt` will be unfolded if requested by `\captionof`. (see above)

```
766 \let\caption@@float\float@caption
767 \long\def\float@caption#1[#2]#3{%
768   \caption@beginex{#1}{#2}{#3}%
769   \let\@fs@capt\caption@@make
770   \caption@@float{#1}[{#2}]{#3}%
771   \captionof@float{%
```

If the `hyperref` package is loaded, we need to set the appropriate anchor for ourself. To do so without adding extra vertical space we need to save (and restore) `\prevdepth` and switch off the interline skip.

```
772   \@ifundefined{hyper@@anchor}{}{%
773     \begingroup
774     \@tempdima\prevdepth
775     \nointerlineskip
776     \let\leavevmode\relax
777     \hyper@@anchor\@currentHref\relax
778     \prevdepth\@tempdima
779     \endgroup}%
780   \def\caption@@make##1#2{\unvbox\@floatcapt}%
781   \@makecaption{}{}%
782 \caption@end}%
```

`\@float@setevery` `\@float@setevery{<float type>}` is provided by the float package; it's called every time a floating environment defined with `\newfloat` or `\restylefloat` begins. We use this hook to do some adaptations and to setup the proper caption style (if defined) and additional settings declared with `\captionsetup[<float style>]`.

```
783 \let\caption@float@setevery\@float@setevery
784 \def\@float@setevery#1{%
```

L<sup>A</sup>T<sub>E</sub>X and most packages use `\<type>name` to provide a macro for the float name – for example the command `\figurename` will usually contain the name of the floating environment figure:

```
\newcommand\figurename{Figure}
```

But the float package don't follow this naming convention, it uses `\fname@<type>` instead. So we have to adapt `\caption@floatname` here, so our captions will be still ok.

```
785 \def\caption@floatname#1{\@nameuse{fname@#1}}%
786 \def\caption@setfloatname#1{\@namedef{fname@#1}}%
```

Both `\newfloat` and `\restylefloat` save the *actual* definition of `\caption` or `\float@caption` in `\@float@c@<capttype>` with `\let` (instead of using `\def`), so redefinitions of `\caption` (and of course our redefinition of `\float@caption`) will never be used if the `\newfloat` or `\restylefloat` command takes place in front of the redefinitions provided by the caption or other packages like the hyperref package. So here we determine if the user has used `\restylefloat` or `\restylefloat*` and bring `\@float@c@<capttype>` up-to-date. This is quite easy: If `\@float@c@<capttype>` is the same as the original or our own definition of `\float@caption`, the user has used `\restylefloat` (and `\float@caption` should be used), otherwise we assume he has used `\restylefloat*` (and `\caption` should be used). (This test will fail if some other package re-defines `\float@caption`, too, so we have to assume that we are the only one.)

```
787 \expandafter\let\expandafter\caption@tempa\csname @float@c@#1\endcsname
788 \ifx\caption@tempa\float@caption
789 \else\ifx\caption@tempa\caption
790 \else\ifx\caption@tempa\caption@float
791 \caption@Info{\protect\@float@c@#1\space := \protect\float@caption}%
792 \expandafter\let\csname @float@c@#1\endcsname\float@caption
793 \else
794 \caption@Info{\protect\@float@c@#1\space := \protect\caption}%
795 \expandafter\let\csname @float@c@#1\endcsname\caption
796 \fi\fi\fi
```

If the floating environment is defined with `\newfloat` or `\restylefloat` (and *not* with `\restylefloat*`), `\@float@c@<type>` will now be identical to `\float@caption`.

```
797 \expandafter\ifx\csname @float@c@#1\endcsname\float@caption
```

First of all we set the caption position to it's proper value. (See above definition of `\caption@setfloatposition`)

```
798 \caption@setfloatposition
```

Now we'll have to determine the current float style. This is not so easy because the only hint provided by the float package is the macro `\fst@⟨float type⟩` which points to the macro which represents the float style. So for example after

```
\floatstyle{ruled}
\newfloat{Program}{tbp}{lop}
```

`\fst@Program` will be defined as

```
\def\fst@Program{\fs@ruled} .
```

So here is what we do: We copy `\fst@⟨float type⟩` to `\caption@fst` and make it a string so we can gobble the first four tokens (= `\fs@`), so only the the name of the float style is left.

```
799 \expandafter\let\expandafter\caption@fst\csname fst@#1\endcsname
800 \edef\caption@fst{\noexpand\string\expandafter\noexpand\caption@fst}%
801 \edef\caption@fst{\noexpand@gobblefour\caption@fst}%
802 % \edef\caption@fst{\caption@fst}%
```

`\caption@fst` now contains the float style (e.g. 'ruled') so we can use it to set the corresponding style (if defined) and additional options.

```
803 \caption@setstyle*\caption@fst
804 \caption@settype\caption@fst
805 \fi
806 \caption@float@setevery{#1}}%
```

`\fs@plaintop` The float styles `plaintop` and `boxed` don't use our `skip` which can be set with `skip=`  
`\fs@boxed` : `plaintop` uses `\belowcaptionskip` instead of `\abovecaptionskip`, and `boxed` uses a fixed space of 2pt. So we patch the according float style macros here to change this.

```
807 \g@addto@macro\fs@plaintop{\def\@fs@mid{\vspace\abovecaptionskip\relax}}%
808 \g@addto@macro\fs@boxed{\def\@fs@mid{\kern\abovecaptionskip\relax}}%
809 }
```

The skip between 'boxed' floats and their caption defaults to 2pt.

```
810 \captionsetup[boxed]{skip=2pt}
```

To emulate the 'ruled' definition of `\@fs@capt` we provide a caption style 'ruled' with appropriate options. But if the package option `ruled` was specified, we setup some caption parameters to emulate the behaviour of the caption package v1.x option `ruled` instead: The current caption settings will be used, but without margin and without 'single-line-check'.

```
811 \caption@ifbool{ruled}{%
812 \captionsetup[ruled]{margin=0pt,singlelinecheck=0}%
813 }%
814 \DeclareCaptionStyle{ruled}{labelfont=bf,labelsep=space,strut=0}%
815 }
816 \caption@undefbool{ruled}
```

### floatrow package support

The floatrow package is already adapted for usage with the caption package. So the main work has already been done by Mrs.Lapko, there are only two little things we have to take care about:

```
817 \caption@ifpackage{floatrow}{flrow@setlist}{%
818   \caption@Info{floatrow package v0.1f (or newer) detected}%
```

`\caption@of` Captions typeset with `\captionof` should have the correct layout, so we have to ‘activate’ this layout here with `\flrow@setlist`.  
(Please note that this version of `\captionof` has the same restrictions than the `\captionof` offered for floating environments defined with the float package, see above.)

```
819   \renewcommand*\caption@of[2]{%
820     \def\@capytype{#2}\flrow@setlist{{#2}}#1}%
```

`\caption@floatname` The floatrow package follows the same naming convention as the float package; so we have to adapt `\caption@floatname` here, too.

```
821   \renewcommand*\caption@floatname[1]{%
822     \@nameuse{\@ifundefined{fname@#1}{#1name}{fname@#1}}}%
823   \renewcommand*\caption@setfloatname[1]{%
824     \@namedef{\@ifundefined{fname@#1}{#1name}{fname@#1}}}%
825 }
```

### hyperref package support

When the hyperref package is used we have the problem that the usage of `\ContinuedFloat` will create duplicate hyperlinks – both `\@currentHlabel` and `\@currentHref` will be the same for the main float and the continued ones. So we have to make sure unique labels and references will be created each time. We do this by extending `\theHfigure` and `\theHtable`, so for continued floats the scheme

$$\langle type \rangle . \langle type \# \rangle . \langle continue \# \rangle$$

will be used instead of

$$\langle type \rangle . \langle type \# \rangle .$$

(This implementation follows an idea from Steven Douglas Cochran.)

Note: This does not help if `\Hy@naturalnamestrue` is set.

```
826 \caption@ifpackage{hyperref}{theHfigure}{%
827   \caption@Info{hyperref package v6.74m (or newer) detected}%
```

`\caption@ContinuedFloat` If `\theH⟨type⟩` is defined, we extend it with `.⟨continue #⟩`. Furthermore we set `\caption@resetContinuedFloat` to `\@gobble` so the continuation counter will not be reset to zero inside `\caption`.

```
828   \def\caption@ContinuedFloat#1{%
829     \@ifundefined{theH#1}{}{%
830       \@ifundefined{CF@#1}{%
```

```

831     \expandafter\caption@newcounter\csname CF@#1\endcsname
832     \caption@resetContinuedFloat{#1}}{}%
833     \expandafter\caption@stepcounter\csname CF@#1\endcsname
834     \expandafter\l@addto@macro\csname theH#1\endcsname{%
835     .\csname CF@#1\endcsname}%
836     \let\caption@resetContinuedFloat\@gobble
837     }}%

```

`\caption@resetContinuedFloat` If a continuation counter is defined, we reset it.

```

838 \def\caption@resetContinuedFloat#1{%
839   \@ifundefined{CF@#1}{}{%
840     \expandafter\caption@setcounter\csname CF@#1\endcsname0}}%
841 }

```

### hycap package support

When the hycap package is used the following problems occur:

1. The hycap package uses `\capstart`, `\hc@caption`, and `\hc@@caption` instead of `\caption` and `\@caption`.<sup>3</sup> So we have to patch these macros, too.
2. `\caption` will be saved to `\hc@org@caption` when the hycap package is loaded. We have to change this so our definition of `\caption` will always be used.
3. Both, `\capstart` and `\hc@@caption`, call `\hyper@makecurrent`. But since we offer `\ContinuedFloat` the float counters could have changed between these both calls! So we fix this by saving the `hyperref` reference (= `\@currentHref`) in `\capstart` and restoring it later on in `\hc@@caption`. (This also fixes the problem that hycap does not work if `\Hy@hypertextnamesfalse` is set.<sup>4</sup> This come in handy; we set it locally to avoid duplicated `hyperref` labels which could occur if `\ContinuedFloat` will be used.)
4. `\capstart` will call `\H@refstepcounter` to increase the float number. This collides with a following `\ContinuedFloat`, too, so we have to move this call from here to `\caption`. (Since we set `\Hy@hypertextnamesfalse` we can do this without problems.)

```

842 \caption@ifpackage{hycap}{hc@caption}{%
843   \caption@Info{hycap package v1.0 (or newer) detected}%

```

`\capstart` Here comes our version of `\capstart`:

```

844 \let\caption@capstart\capstart
845 \def\capstart{%

```

---

<sup>3</sup>This issue was fixed in hycap v1.7

<sup>4</sup>This issue was fixed in hycap v1.6

First of all we update `\hc@org@caption` to correct the problem that the `hypcap` package has saved an older definition of `\caption`.

```
846 \let\hc@org@caption\caption
```

Since we don't know the float counter yet (it could be changed with `\ContinuedFloat` afterwards!) we make sure `\H@refstepcounter` will not be used and `\Hy@hypertexnamesfalse` is set, so unique `hyperref` labels will be generated by the original definition of `\capstart`.

Afterwards we save the reference which was generated by `\hyper@makecurrent`.

```
847 \begingroup
848 \let\H@refstepcounter\@gobble
849 \Hy@hypertexnamesfalse
850 \caption@capstart
851 \@ifundefined{hc@hyperref}{}{% hypcap v1.7
852 \global\advance\c@name c@\@captype\endcsname\@ne}%
853 \global\let\hc@currentHref\@currentHref
854 \endgroup
```

The `hypcap` package restores the previous definition of `\caption` inside `\hc@@caption`. But since we will call this inside a group later on (making this restauration non-working), we have to make this for ourself inside `\caption`. (This would not be necessary if `hypcap` would do this inside `\hc@caption` instead of `\hc@@caption`.)

Additionally we increase the float counter here (since we have suppressed this in `\capstart`) and use `\caption@caption` here, so `\caption*` will work as expected. (This is surrounded by `\hc@hyperref` so it does not make any harm when used with `hypcap v1.7`.)

```
855 \@ifundefined{hc@hyperref}%
856 {\let\next\@firstofone}\let\next\hc@hyperref}% hypcap v1.7
857 \next{\def\caption{%
858 \let\caption\hc@org@caption
859 \H@refstepcounter\@captype
860 \@ifundefined{hc@hyperref}{}{% hypcap v1.7
861 \global\advance\c@name c@\@captype\endcsname\@m@ne}%
862 \caption@caption\hc@caption}}%
863 }%
```

`\hc@@caption` Here comes our version of `\hc@@caption`:

```
864 \let\caption@hc@@caption\hc@@caption
865 \long\def\hc@@caption#1[#2]#3{%
866 \caption@beginex{#1}{#2}{#3}%
```

Beside the usual `\caption@begin` and `\caption@end` stuff (to support local options etc.) we make sure our saved `hyperref` reference will be used.

```
867 \let\caption@hyper@makecurrent\hyper@makecurrent
868 \def\hyper@makecurrent\@captype{%
869 \let\hyper@makecurrent\caption@hyper@makecurrent
870 \global\let\@currentHref\hc@currentHref}%
871 \caption@hc@@caption{#1}[{#2}]{#3}%
872 \caption@end}%
```

```
873 }
```

### listings package support

```
874 \caption@ifpackage{listings}{\lst@MakeCaption}{%
875 \caption@Info{listings package v1.2 (or newer) detected}%
```

`\lst@MakeCaption` To support the listings package we need to redefine `\lst@MakeCaption` so the original stuff is nested with `\caption@begin` and `\caption@end`.

```
876 \let\caption@lst@MakeCaption\lst@MakeCaption
877 \def\lst@MakeCaption#1{%
```

If the `position=` is set to `auto`, we take over the `captionpos=` setting from the listings package. Note that we won't do this otherwise, so listings settings like `abovecaptionskip=0pt`, `belowcaptionskip=10pt`, `captionpos=t` will *not* cause different outputs with or without the caption package loaded.

```
878 \def\caption@autoposition{\caption@setposition{#1}}%
879 \caption@begin{lstlisting}%
880 \caption@lst@MakeCaption{#1}%
881 \caption@end}%
882 }
```

### longtable package support

```
883 \caption@ifpackage{longtable}{\LT@makecaption}{%
884 \caption@Info{longtable package v3.15 (or newer) detected}%
```

`\LT@makecaption` `\LT@makecaption{<cmd>}{<label>}{<text>}`

Original code:

```
\def\LT@makecaption#1#2#3{%
\LT@mcol\LT@cols c{\hbox to\z@{\hss\parbox[t]\LTcapwidth{%
% Based on article class "\@makecaption", "#1" is "\@gobble" in star
% form, and "\@firstofone" otherwise.
\sbox\@tempboxa{#1{#2: }#3}%
\ifdim\wd\@tempboxa>\hsize
#1{#2: }#3%
\else
\hbox to\hsize{\hfil\box\@tempboxa\hfil}%
\fi
\endgraf\vskip\baselineskip}%
\hss}}}
```

```
885 \def\LT@makecaption#1#2#3{%
886 \caption@LT@make{%
```

We set `\ifcaption@star` according the 1st argument.

```
887 \caption@startrue#1\caption@starfalse
```

If `\LTcapwidth` is not set to its default value `4in` we assume that it shall overwrite our own setting. (But `\captionsetup[longtable]{width=...}` will overwrite `\LTcapwidth`.)

```

888     \caption@letfloattype{longtable}{%
889       \ifdim\LTcapwidth=4in \else
890         \setcaptionwidth\LTcapwidth
891       \fi}%

```

The default `position=` setting for `longtables` is `top`. (This emulates the standard behaviour of the `longtable` package which has no skip above the caption but a skip below it.)

```

892 %     \caption@setdefaultpos{t}%
893     \let\caption@defaultpos\@firstoftwo

```

`position=auto` is a bad idea for `longtables`, but we do our very best. This works quite well for captions inside the `longtable` contents, but not for captions inside the `longtable` (end)foot.

```

894     \def\caption@autoposition{%
895       \caption@setposition{\ifcase\LT@rows t\else b\fi}}%
896     \caption@begin{table}%

```

The following skip has the purpose to correct the height of the `\parbox[t]`. Usually it's the height of the very first line, but because of our extra skips (`\abovecaptionskip` and `\belowcaptionskip`) it's always 0pt. (A different idea would be typesetting the first skip outside the `longtable` column with `\noalign{\vskip...}`, but this means we have to move `\caption@begin` to some other place because it does not work in tabular mode...)

```

897     \vskip-\ht\strutbox

```

This should look familiar. We do our skips and use `\caption@@make` to typeset the caption itself.

```

898     \caption@iftop{\vskip\belowcaptionskip}{\vskip\abovecaptionskip}%
899     \caption@@make{#2}{#3}\endgraf
900     \caption@iftop{\vskip\abovecaptionskip}{\vskip\belowcaptionskip}%
901     \caption@end}}%

```

`\caption@LT@make` Typesets the caption as centered `\multicolumn...`

```

902 \newcommand\caption@LT@make[1]{%
903   \LT@mcol\LT@cols c{\hbox to\z@{\hss\parbox[t]\hsize{#1}\hss}}}%
904 }

```

### picins package support

```

905 \caption@ifpackage{picins}{piccaption}{%
906 \caption@Info{picins package v3.0 (or newer) detected}%

```

`\piccaption` Original code:

```

\def\piccaption{\@ifnextchar [{\@piccaption}{\@piccaption[]}]

907 \def\piccaption{\@dblarg\@piccaption}
908 % \def\piccaption{\caption@caption{\@dblarg\@piccaption}}

```

*TODO: Make \piccaption[...]{...} and \piccaption{} work*

909 }

### rotating package support

```
910 \caption@ifpackage{rotating}{@rotcaption}{%
911 \caption@Info{rotating package v2.0 (or newer) detected}%
```

```
\rotcaption Make \rotcaption* work.
```

```
912 \def\rotcaption{\let\@makecaption\@makerotcaption\caption}%
913 % \let\@rotcaption\@undefined
```

```
\rotcaptionof Make \rotcaptionof(*) work.
```

```
914 \def\rotcaptionof{%
915 \@ifstar{\caption@of{\rotcaption*}}{\caption@of\rotcaption}}%
```

```
\@makerotcaption Original (bugfixed) code:
```

```
\long\def\@makerotcaption#1#2{%
\setbox\@tempboxa\hbox{#1: #2}%
\ifdim \wd\@tempboxa > .8\vsizel
\rotatebox{90}{%
\begin{minipage}{.8\textheight}#1: #2\end{minipage}%
}%\par % <== \par removed (AR)
\else%
\rotatebox{90}{\box\@tempboxa}%
\fi
\nobreak\hspace{12pt}% <== \nobreak added (AR)
}
```

Our version emulates this behaviour, but if `width=` is set, the rotated caption is always typeset as `minipage`. (Note that `margin=` is not supported here.)

```
916 \long\def\@makerotcaption#1#2{%
917 \ifdim\captionwidth=\z@
918 \setcaptionwidth{.8\textheight}%
919 \caption@slc{#1}{#2}{.8\vsizel}{%
920 \let\caption@makerot\caption@@make
921 \setcaptionmargin\z@
922 % \setlength\captionindent\z@
923 % \long\def\captionbox##1##2{\hbox{\hsize=.8\textheight\relax##2}}%
924 % (not needed because \rotatebox uses an \hbox anyway)
925 \let\captionbox\@secondoftwo}%
926 \caption@setbool{slc}{0}% been there, done that
927 \fi
928 \rotatebox{90}{\caption@makerot{#1}{#2}}%
929 \nobreak\hspace{12pt}}%
930 \newcommand\caption@makerot[2]{%
931 \begin{minipage}\captionwidth\caption@@make{#1}{#2}\end{minipage}}%
932 }
```

### sidecap package support

```
933 \caption@ifpackage{sidecap}{endSC@FLOAT}{%
934 \caption@Info{sidecap package v1.4d (or newer) detected}%
\SC@caption First of all, we let sidecap use an actual definition of \caption.
(This is only required for version 1.5d of the sidecap package.)
935 \@ifundefined{caption@caption}{%
936 {\let\caption@tempa\AtBeginDocument}%
937 {\let\caption@tempa\@firstofone}%
938 \caption@tempa{\let\SC@caption=\caption}%

\SC@zfloat This macro will be called at the start of the environment, here is a good opportunity to do
some adaptations to \caption and \captionsetup.
939 \let\caption@SC@zfloat\SC@zfloat
940 \def\SC@zfloat#1#2#3[#4]{%

Note: #2 is either figure or table and will be stored to \SC@capttype by the
original version of \SC@zfloat.
941 \caption@SC@zfloat{#1}{#2}{#3}[#4]%

Since the sidecap package uses our \caption code outside the floating environment the
regular \captionsetup will not work. So we need a special version here which saves
the given argument list which will be executed later on.
942 \global\let\SC@CAPsetup\@empty
943 \def\captionsetup##1{\g@addto@macro\SC@CAPsetup{,##1}}%

Make \caption* work.
944 \let\caption@SC\caption
945 % \def\caption{\renewcommand\captionsetup[1]{}\caption@caption\caption@SC}%
946 \def\caption{\caption@caption\caption@SC}%
947 }%

\endSC@FLOAT This macro will be called at the end of the environment, here we need to setup our stuff
before the sidecap package actually typesets its caption.
948 \let\caption@endSC@FLOAT\endSC@FLOAT
949 \def\endSC@FLOAT{%

Note that \@capttype isn't defined so far, this will be done inside the original
definition of \endSC@FLOAT. But we define \@capttype already here to make
\captionsetup work with \@capttype-based options (like type=).
950 \let\@capttype\SC@capttype

Here we execute the options set with \captionsetup inside this environment.
951 \caption@esetup\SC@CAPsetup

Before we can typeset the caption we need to set the margin to zero because any extra
margin would only be disturbing here.
(We don't need to take care about the caption position because the sidecap package set
both \abovecaptionskip and \belowcaptionskip to a skip of zero anyway.)
Furthermore \SC@justify will override the caption justification, if set. The usage of
\SC@justify differs from version to version of the sidecap package:
```

Version 1.4: \SC@justify is not defined  
 Version 1.5: \SC@justify is \relax when not set  
 Version 1.6: \SC@justify is \@empty when not set

```

952 \caption@letfloattype{SC@capttype}{%
953 \listdepth\z@
954 \setcaptionmargin\z@
955 \@ifundefined{SC@justify}{}{%
956 \ifx\SC@justify\@empty\else
957 \let\caption@hj\SC@justify
958 \let\SC@justify\@empty
959 \fi}}%

```

We adapt \caption@ifempty so \caption{} will work within these environments, too.

```

960 \long\def\caption@ifempty##1{%
961 \ifx\SC@CAPtext\@empty
962 \expandafter\@firstofone
963 \else
964 \expandafter\@gobble
965 \fi}%

```

Finally we call the original definition of \endSC@FLOAT which will call our version of \caption to typeset the caption.

```

966 \caption@endSC@FLOAT}%
967 }

```

#### supertabular package support

\caption@setSTposition The position= setting will be overwritten by the supertabular package: If \topcaption is used, the position will be top automatically, bottom otherwise.

```

968 \def\caption@setSTposition{%
969 \caption@setposition{\if@topcaption t\else b\fi}}

970 \caption@ifpackage{supertabular}{ST@caption}{%
971 \caption@Info{supertabular package detected}%

```

\tablecaption Make \topcaption\* and \bottomcaption\* work.

```

972 \let\caption@tablecaption\tablecaption
973 \def\tablecaption{\caption@caption\caption@tablecaption}%

```

\ST@caption Original code:

```

\long\def\ST@caption#1[#2]#3{\par%
\addcontentsline{\csname ext@#1\endcsname}{#1}%
{\protect\numberline{%
\csname the#1\endcsname}{\ignorespaces #2}}

\begingroup
\@parboxrestore
\normalsize

```

```

\if@topcaption \vskip -10\p@ \fi
\@makecaption{\csname fnum@#1\endcsname}{\ignorespaces #3}\par
\if@topcaption \vskip 10\p@ \fi
\endgroup}

974 \long\def\ST@caption#1[#2]#3{\par%
975 \caption@letfloattype{supertabular}{}%
976 \let\caption@fixposition\caption@setSTposition
977 \caption@beginex{#1}{#2}{#3}%
978 \addcontentsline{\csname ext@#1\endcsname}{#1}%
979 {\protect\numberline{%
980 \csname the#1\endcsname}{\ignorespaces #2}}%
981 \@parboxrestore
982 \normalsize
983 \@makecaption{\csname fnum@#1\endcsname}{\ignorespaces #3}\par
984 \caption@end}%

985 }

```

## References

- [1] Frank Mittelbach and Michel Goossens: *The L<sup>A</sup>T<sub>E</sub>X Companion (2nd. Ed.)*, Addison-Wesley, 2004.
- [2] Anselm Lingnau: *An Improved Environment for Floats*, 2001/11/08
- [3] Olga Lapko: *The floatrow package documentation*, 2005/05/22
- [4] Sebastian Rahtz & Heiko Oberdiek: *Hypertext marks in L<sup>A</sup>T<sub>E</sub>X*, 2007/01/25
- [5] Heiko Oberdiek: *The hypcap package – Adjusting anchors of captions* 2007/02/19
- [6] Carsten Heinz: *The Listings Package*, 2004/02/13
- [7] David Carlisle: *The longtable package*, 2000/10/22
- [8] Sebastian Rahtz and Leonor Barroca: *A style option for rotated objects in L<sup>A</sup>T<sub>E</sub>X*, 1997/09/26
- [9] Rolf Niepraschk und Hubert Gäßlein: *The sidecap package*, 2003/06/06
- [10] Steven D. Cochran: *The subfig package*, 2005/07/05
- [11] Johannes Braams und Theo Jurriens: *The supertabular environment*, 2002/07/19
- [12] Anne Brüggemann-Klein: *Einführung in die Dokumentverarbeitung*, B.G. Teubner, Stuttgart, 1989
