# Supplementary material for: Reentrant phenomenon in the exactly solvable mixed spin-1/2 and spin-1 Ising-Heisenberg model on diamond-like decorated planar lattices
Source: arXiv:0909.4191 source file (2009-09-23)
Supplement: Supplementary file 3 [file caption2.pdf]

# The caption2 package\*

Axel Sommerfeldt  
caption@sommerfee.de

2007/04/06

## **THIS PACKAGE IS OBSOLETE!**

The caption2 package used to be an experimental side-version of the regular caption package. It was made public as beta test version without documentation in 1995 because of the demand for new features and adaptations to other packages like the longtable and subfigure package.

Even in the next years I found no time to reintegrate some of the well-tried features into the regular caption package. So I decided to release a version 2.1 of the caption2 package in 2002 instead, which included some minor bug fixes and adaptations to the new version 2.1 of the subfigure package. Furthermore I started to write a documentation for this package, but unfortunately did not get very far with this. . .

In 2003 I finally found some (more) time, so a new regular release 3.0 of the caption package could be build with massive help from Frank Mittelbach[5] and Steven Cochran[4]. It was released in December 2003 and superseded the neglected caption2 package.

(In parallel, Steven Cochran released the subfig package which superseded the subfigure package.)

So please don't use this package for new documents. It's old, it's obsolete and it starts to begin smell bad! Please ignore all hints in books or other documents which try to tell you that the caption2 package should be used instead of the caption package – these hints are outdated since December 2003.

## **How to migrate to the regular caption package?**

Usually replacing caption2 by caption is sufficient because the caption package emulates most of the options and commands of the caption2 package. If you get some errors or wired results afterwards, please take a closer look at the caption package documentation which will hopefully help you clearing these problems. You will also find a section called 'Compatibility to older versions' there which should help you with the migration process. If all this should fail you can write me an e-mail asking for help.

---

\*This package has version number v2.2a, last revised 2007/04/11.

## **What will happen to this package?**

The caption2 package is still some kind of supported, that means it will be part of future releases and bugs will still be fixed so existing documents using this package will still compile. But it will *not* be enhanced in the future or adapted to future versions of foreign packages.

This means migrating to the actual caption package should not be necessary for old documents – they should still compile fine as they are. If they don't please don't hesitate to write me an e-mail asking for maintainance.

# 1 The Implementation

## 1.1 Identificaton

```
1 \NeedsTeXFormat{LaTeX2e}[1994/12/01]
2 \ProvidesPackage{caption2}[2007/04/11 v2.2a Customising captions (AS)]
3 \PackageWarningNoLine{caption2}{%
4   *** THIS PACKAGE IS OBSOLETE, PLEASE USE caption ***}
```

## 1.2 Loading the caption3 kernel

```
5 \RequirePackage{caption3}[2007/03/04] % needs v3.0m or newer
```

## 1.3 Check against the regular caption package

```
6 \@ifpackageloaded{caption}{%
7   \PackageError{caption2}{You can't use both the caption *and* caption2 package}
8   \endinput
9 }{}
```

## 1.4 Preliminary declarations

`\captionlabeldelim` & `\captionlabelsep` will hold the iterim space between caption label and text. (`\captionlabeldelim` will be typeset within `\captionlabelfont`, `\captionlabelsep` not.)

```
10 \newcommand*\captionlabeldelim{}
11 \newcommand*\captionlabelsep{}
```

`\ifcaptionwidth` Either `\captionmargin` (with specifies an extra margin) or `\captionwidth` (with specifies an explicit width) can be set, therefore we need the flag `\ifcaptionwidth` to determine with parameter we should pay attention to.

```
12 \newcommand*\ifcaptionwidth{\ifdim\captionwidth>\z@}
```

```
13 \newif\ifcaption@temp
```

`\ifcaptionlabel` If `\ifcaptionlabel` is not set the caption label should be suppressed; we need this flag to support the `\caption*` command.

```
14 \def\ifcaptionlabel{%
15   \ifcaption@star
16     \caption@tempfalse
17   \else
18     \caption@temptrue
19   \fi
20 \ifcaption@temp}
21 \def\captionlabeltrue{\caption@starfalse}
22 \def\captionlabelfalse{\caption@startrue}
```

`\ifonelinecaptions` If `\ifonelinecaptions` is set we support the L<sup>A</sup>T<sub>E</sub>X base style 'one line captions', that means the caption will be typeset centered if it fits to one line.

```

23 \def\ifonelinecaptions{%
24   \caption@ifslc{\caption@temptrue}{\caption@tempfalse}%
25   \ifcaption@temp}
26 \def\onelinecaptionstrue{\caption@setbool{slc}{1}}
27 \def\onelinecaptionsfalse{\caption@setbool{slc}{0}}
```

`\ifignoreLTcapwidth` If `\ifignoreLTcapwidth` is set we ignore the `\LTcapwidth` of `longtable`.

```

28 \newif\ifignoreLTcapwidth
```

`\normalcaptionparams` `\normalcaptionparams` resets all caption related parameters to it's normal default values. `\captionfont` will be set to `\captionsize` so setting the obsolete `\captionsize` will still work. Same story with `\captiondelim` and the obsolete `\captionlabeldelim`.

```

29 \newcommand*\normalcaptionparams{%
30   \let\captionsize\@empty
31   \renewcommand*\captionfont{\captionsize}%
32   \let\captionlabelfont\@empty
33   \renewcommand*\captionlabeldelim{:}%
34   \renewcommand*\captionlabelsep{\space}%
35   \setcaptionmargin\z@
36   \setlength\captionindent\z@
37   \onelinecaptionstrue}
```

`\defcaptionstyle` `\newcaptionstyle` `\renewcaptionstyle` These macros will define a new caption style. `\newcaptionstyle` and `\renewcaptionstyle` will additionally check if the caption style already exists or not.

```

38 \newcommand*\defcaptionstyle[1]{%
39   \@namedef{caption@@#1}}
40 %
41 \newcommand*\newcaptionstyle[1]{%
42   \expandafter\ifx\csname caption@@#1\endcsname\relax
43     \expandafter\defcaptionstyle
44   \else
45     \PackageError{caption2}{Caption style `#1' already defined}{\caption@eh}%
46     \expandafter\@gobbletwo
47   \fi
48   {#1}}
49 %
50 \newcommand*\renewcaptionstyle[1]{%
51   \expandafter\ifx\csname caption@@#1\endcsname\relax
52     \PackageError{caption2}{Caption style `#1' undefined}{\caption@eh}%
53     \expandafter\@gobbletwo
54   \else
55     \expandafter\defcaptionstyle
56   \fi
57   {#1}}
```

`\dummycaptionstyle` This macro will also define a new caption style, but a one which is based on the actual set caption style. Therefore you can't set a caption style made with this command with `\captionstyle` – we check this to avoid an endless recursion.

```
58 \newcommand*\dummycaptionstyle[2]{%
59   \defcaptionstyle{#1}{%
60     \expandafter\ifx\csname caption@@\caption@style\expandafter\endcsname%
61       \csname caption@@#1\endcsname
62     \PackageError{caption2}{You can't use the caption style '#1' directly}{%
63       The caption style '#1' is only a dummy and does not really exist.%
64       \MessageBreak You have to redefine it (with \protect\renewcaptionstyle)
65       before you can select\MessageBreak it with \protect\captionstyle.
66       \space\caption@eh}%
67   \else
68     #2\usecaptionstyle\caption@style
69   \fi}}
```

`\captionstyle` `\captionstyle` sets the actual caption style. It includes a check if the given caption style is defined or not.

```
70 \newcommand*\captionstyle[1]{%
71   \expandafter\ifx\csname caption@@#1\endcsname\relax
72     \PackageError{caption2}{Undefined caption style '#1'}{\caption@eh}%
73   \else
74     \def\caption@style{#1}%
75   \fi}}
```

`style 'normal'` `style 'center'` `style 'centerlast'` `style 'flushleft'` `style 'flushright'` `style 'hang'` `style 'indent'` The predefined caption styles 'normal', 'center', 'flushleft', 'flushright', 'centerlast', 'hang', 'hang+X', and 'indent'. Because they are quite similar they all are based on the macro `\caption@make`.

```
76 \newcaptionstyle{normal}{\caption@make{normal}}
77 \newcaptionstyle{center}{\caption@make{center}}
78 \newcaptionstyle{centerlast}{\caption@make{centerlast}}
79 \newcaptionstyle{flushleft}{\caption@make{flushleft}}
80 \newcaptionstyle{flushright}{\caption@make{flushright}}
81 \newcaptionstyle{hang}{\caption@make{hang}}
82 \newcaptionstyle{hang+center}{\caption@make{hang@center}}
83 \newcaptionstyle{hang+centerlast}{\caption@make{hang@centerlast}}
84 \newcaptionstyle{hang+flushleft}{\caption@make{hang@flushleft}}
85 \newcaptionstyle{indent}{\caption@make{indent}}
```

`\caption@makecaption` Our predefined caption styles. `\caption@makecaption` takes the style name as parameter, it does the common stuff and calls a macro (build out of the style name) to do the uncommon stuff if necessary.

```
86 \newcommand*\caption@makecaption[1]{%
87   \usecaptionmargin

88   \ifcaptionlabel
89     \def\caption@label{%
```

```

90      {\captionlabelfont\captionlabel\captionlabeldelim}\captionlabelsep}%
91 \else
92   \let\caption@label\@empty
93 \fi

94 \captionfont
95 \onelinecaption
96   {\caption@label\captiontext}%
97   {\parbox[b]\captionlinewidth{\strut\@nameuse{caption@@@#1}\par}\par}}

```

`\caption@@@normal` The ‘normal’ caption style. Just typeset caption (label & text) as paragraph.

```

98 \newcommand*\caption@@@normal{%
99   \caption@label\captiontext}

```

`\caption@@@center` The ‘center’ caption style. Typeset the caption centered within a parbox.

```

100 \newcommand*\caption@@@center{%
101   \centering\caption@label\captiontext}%

```

`\caption@@@centerlast` The ‘centerlast’ caption style. The idea how to do this was taken from Brüggemann-Klein[6], it is also mentioned in Kopka[7, p227].

```

102 \newcommand*\caption@@@centerlast{%
103   \centerlast\caption@label\captiontext}

```

`\caption@@@flushleft` The ‘flushleft’ caption style. Typeset the caption raggedright within a parbox.

```

104 \newcommand*\caption@@@flushleft{%
105   \raggedright\caption@label\captiontext}%

```

`\caption@@@flushright` The ‘flushright’ caption style. Typeset the caption raggedleft within a parbox.

```

106 \newcommand*\caption@@@flushright{%
107   \raggedleft\caption@label\captiontext}%

```

`\caption@@@hang` The ‘hang’ caption style. This code was taken from The L<sup>A</sup>T<sub>E</sub>X Companion[5, p155] and modified.

`\caption@hangplus`

```

108 \newcommand*\caption@@@hang{%
109   \sbox\@tempboxa{\caption@label}%
110   \hangindent\wd\@tempboxa\noindent
111   \usebox\@tempboxa\caption@hangplus\captiontext}

```

```

112 \newcommand*\caption@hangplus{}

```

`\caption@@@hang@center` The ‘hang+flushleft’ caption style.

```

113 \newcommand*\caption@@@hang@center{%
114   \let\caption@hangplus\centering\caption@@@hang}

```

`\caption@@@hang@centerlast` The ‘hang+flushleft’ caption style.

```

115 \newcommand*\caption@@@hang@centerlast{%
116   \let\caption@hangplus\centerlast\caption@@@hang}

```

`\caption@@@hang@flushleft` The ‘hang+flushleft’ caption style.

```

117 \newcommand*\caption@@@hang@flushleft{%
118   \let\caption@hangplus\raggedright\caption@@@hang}

```

`\caption@@@indent` The ‘indent’ caption style. Is is quite like the ‘hang’ style but the indentation is given as `\captionindent`.

```

119 \newcommand*\caption@@@indent{%
120   \hangindent\captionindent\noindent
121   \caption@label\captiontext}

```

## 1.5 Options

`normal` These options will set the caption style. (‘normal’ is the default one.)

`center` The options ‘anne’ and ‘isu’ are for backward compatibility only.

`centerlast, anne`

`flushleft`

`flushright`

`hang, isu`

`indent`

```

122 \DeclareOption{normal}{\captionstyle{normal}}
123 \DeclareOption{center}{\captionstyle{center}}
124 \DeclareOption{centerlast}{\captionstyle{centerlast}}
125 \DeclareOption{flushleft}{\captionstyle{flushleft}}
126 \DeclareOption{flushright}{\captionstyle{flushright}}
127 \DeclareOption{anne}{\ExecuteOptions{centerlast}}
128 \DeclareOption{hang}{\captionstyle{hang}}
129 \DeclareOption{hang+center}{\captionstyle{hang+center}}
130 \DeclareOption{hang+centerlast}{\captionstyle{hang+centerlast}}
131 \DeclareOption{hang+flushleft}{\captionstyle{hang+flushleft}}
132 \DeclareOption{isu}{\ExecuteOptions{hang}}
133 \DeclareOption{indent}{\captionstyle{indent}}

```

`scriptsize` These options will set the caption size. We use `\g@addto@macro` so more than one

`footnotesize` option can be set.

`small`

`normalsize`

`large, Large`

```

134 \DeclareOption{scriptsize}{\g@addto@macro\captionsize\scriptsize}
135 \DeclareOption{footnotesize}{\g@addto@macro\captionsize\footnotesize}
136 \DeclareOption{small}{\g@addto@macro\captionsize\small}
137 \DeclareOption{normalsize}{\g@addto@macro\captionsize\normalsize}
138 \DeclareOption{large}{\g@addto@macro\captionsize\large}
139 \DeclareOption{Large}{\g@addto@macro\captionsize\Large}

```

`up, it, sl, sc` These options will set the caption label.

`md, bf`

`rm, sf, tt`

```

140 \DeclareOption{up}{\g@addto@macro\captionlabelfont\upshape}
141 \DeclareOption{it}{\g@addto@macro\captionlabelfont\itshape}
142 \DeclareOption{sl}{\g@addto@macro\captionlabelfont\slshape}
143 \DeclareOption{sc}{\g@addto@macro\captionlabelfont\scshape}

```

```

144 \DeclareOption{md}{\g@addto@macro\captionlabelfont\mdseries}
145 \DeclareOption{bf}{\g@addto@macro\captionlabelfont\bfseries}
146 \DeclareOption{rm}{\g@addto@macro\captionlabelfont\rmfamily}
147 \DeclareOption{sf}{\g@addto@macro\captionlabelfont\sffamily}
148 \DeclareOption{tt}{\g@addto@macro\captionlabelfont\ttfamily}

oneline  These options will set the ‘oneline’ flag. (‘oneline’ is the default.)
nooneline
149 \DeclareOption{oneline}{\onelinecaptionstrue}
150 \DeclareOption{nooneline}{\onelinecaptionsfalse}

\caption@setpackage  A helper macro, a value of 1 within parameter #2 will activate the support of the package
given in parameter #1, a value of 0 will deactivate it.
151 \newcommand*\caption@setpackage[1]{\@namedef{caption@pkt@#1}}

float  These options will enable or suppress the support of the packages float, longtable, and
longtable  subfigure.
subfigure
152 \DeclareOption{float}{\caption@twozerofalse\caption@setpackage{float}{1}}
153 \DeclareOption{longtable}{\caption@twozerofalse\caption@setpackage{longtable}{1}}
154 \DeclareOption{subfigure}{\caption@twozerofalse\caption@setpackage{subfigure}{1}}

none  These options will enable or suppress the support of all the above packages.
all
155 \DeclareOption{none}{\caption@twozerofalse
156 \caption@setpackage{float}{0}\caption@setpackage{longtable}{0}%
157 \caption@setpackage{subfigure}{0}}
158 \DeclareOption{all}{\ExecuteOptions{float,longtable,subfigure}}

ruled  The option ‘ruled’ introduced in caption v1.2 is obsolete now, but we will still support it.
boxed  The option ‘boxed’ was introduced in version 2.0 and is obsolete now, too.
159 \newif\ifcaption@ruled
160 \DeclareOption{ruled}{\caption@ruledtrue}
161 \DeclareOption{boxed}{}

ignoreLTcapwidth  This option will make the caption code ignore the setting of \LTcapwidth and use the
setting of \setcaptionmargin or \setcaptionwidth instead.
162 \DeclareOption{ignoreLTcapwidth}{\ignoreLTcapwidthtrue}

debug  This option will put additional debug information in the log file.
163 \DeclareOption{debug}{\captionsetup{debug}}

That’s it! Now set the default values and start processing the options. (If \caption@twozero
is set to true (default) we will emulate the package load algorithm of caption v2.0: If the
package is already loaded patch it, otherwise do nothing.)
164 \newif\ifcaption@twozero
165 \normalcaptionparams

```

```

166 \ExecuteOptions{none,normal}
167 \caption@twozerotrue
168 \ProcessOptions*
169 \ifcaption@twozero
170 \PackageInfo{caption2}{Running in caption2 v2.0 compatibility mode}
171 \fi

```

## 1.6 More declarations

`\captionof` `\captionof resp. \captionof*` will just set `\@capttype` and do the normal `\captionof*` `\caption resp. \caption*`, so we can also typeset captions outside floating environments.

```

172 \def\captionof{\@ifstar{\caption@of{\caption*}}{\caption@of\caption}}
173 \newcommand*\caption@of[2]{\def\@capttype{#2}#1}

```

`\abovecaptionskip` `\belowcaptionskip` Not all document classes define `\abovecaptionskip` and `\belowcaptionskip` (like `ucthesis`), so we do it here if not already done.

```

174 \@ifundefined{abovecaptionskip}{%
175   \newlength\abovecaptionskip\setlength\abovecaptionskip{10\p}}{}
176 \@ifundefined{belowcaptionskip}{%
177   \newlength\belowcaptionskip\setlength\belowcaptionskip{0\p}}{}

```

`\captionlinewidth` `\captionlabel` `\captiontext` These values are only set and used within the caption code itself. `\captionlinewidth` will be set to the given vertical space for the caption, normally this is `\linewidth`. (This value was called `\realcaptionwidth` within `caption2 2.0`, so we will offer this, too.)

`\captionlabel` and `\captiontext` will be set to the caption label resp. the caption text. (Because `\captionlabel` and `\captiontext` will be locally defined with `\def` we do not need to define them here.)

```

178 \newdimen\captionlinewidth
179 \newdimen\realcaptionwidth

```

`\usecaptionmargin` A helper macro for caption style authors: It calculates `\leftskip` and `\rightskip` out of `\captionlinewidth` and `\captionmargin resp. \captionwidth`. Also `\captionlinewidth` will be corrected to the appropriate value.

```

180 \newcommand*\usecaptionmargin{%
181   \ifcaptionwidth
182     \leftskip\captionlinewidth
183     \advance\leftskip by -\captionwidth
184     \divide\leftskip by 2
185     \rightskip\leftskip
186     \captionlinewidth\captionwidth
187   \else
188     \leftskip\captionmargin
189     \rightskip\captionmargin

```

```

190 \advance\captionlinewidth by -2\captionmargin
191 \fi
192 \realcaptionwidth\captionlinewidth}

```

`\onelinecaption` This macro definition helps setting captions the  $\LaTeX$  base classes way: If `\ifonelinecaptions` is set and the 1st argument fits within `\captionlinewidth`, we typeset it centered – otherway we typeset the 2nd argument. (We use the savebox `\@tempboxa` as helper for this.)

```

193 \newcommand\onelinecaption[1]{%
194 \let\next\@firstofone
195 \ifonelinecaptions
196 \sbox\@tempboxa{#1}%
197 \ifdim\wd\@tempboxa >\captionlinewidth
198 \else
199 \def\next{{\centering\usebox\@tempboxa\par}\@gobble}%
200 \fi
201 \fi\next}

```

`\usecaptionstyle` First we check if we are inside a caption – if `\captiontext` is undefined we are not. If we are we call the appropriate caption definition.

```

202 \newcommand*\usecaptionstyle[1]{%
203 \@ifundefined{captiontext}{%
204 \PackageError{caption2}{You can't use \protect#1
205 in normal text}{The usage of \protect#1 is only
206 allowed inside code declared with\MessageBreak \protect\defcaptionstyle,
207 \protect\newcaptionstyle \space or \protect\renewcaptionstyle.
208 \space\caption@eh}
209 }{%
210 \@ifundefined{caption@@#1}%
211 {\PackageError{caption2}{Caption style '#1' undefined}{\caption@eh}}%
212 {\let\caption@make\caption@makecaption
213 \@nameuse{caption@@#1}}%
214 }}

```

`\@makecaption` This is the heart of the `caption2` package – the redefinition of the core caption code. It was taken from the  $\LaTeX 2\epsilon$  standard classes and modified. It's very easy – apart from using `\abovecaptionskip` and `\belowcaptionskip` we just set `\captionlinewidth`, `\captionlabel` and `\captiontext` to its appropriate values and using the code of the actual caption style via `\usecaptionstyle`.

```

215 \renewcommand\@makecaption[2]{%
216 \vskip\abovecaptionskip
217 \captionlinewidth\hsize
218 \realcaptionwidth\hsize
219 \def\captionlabel{#1}%
220 \def\captiontext{#2}%
221 \usecaptionstyle\caption@style
222 \vskip\belowcaptionskip}

```

## 1.7 Support of other packages

`\caption@ifpackage` This macro will execute the code needed to support the package named within argument #1. The parameter #2 is the command which shows if the package is loaded – it is defined, it is already loaded, otherwise not. The parameter #3 contains code which will be executed if no support is required – this is for cleanup purposes. The final parameter #4 contains the code itself.

```
223 \newcommand*\caption@ifpackage[3]{%
224   \if1\@nameuse{caption@pkt@#1}%
225     \ifundefined{#2}%
226       {\let\next\AtBeginDocument}%
227       {\let\next\@firstofone}%
228   \else\ifcaption@twozero
229     \ifundefined{#2}%
230       {#3\let\next\@gobble}%
231       {\let\next\@firstofone}%
232   \else
233     #3\let\next\@gobble
234   \fi\fi
235   \expandafter\let\csname caption@pkt@#1\endcsname\undefined
236   \caption@ifdebug{%
237     \ifx\next\@gobble\PackageInfo{caption2}{#1 => gobble}%
238     \else\ifx\next\@firstofone\PackageInfo{caption2}{#1 => firstofone}%
239     \else\ifx\next\AtBeginDocument\PackageInfo{caption2}{#1 => AtBeginDocument}%
240     \fi\fi\fi}{}%
241   \next}
```

### 1.7.1 Support of the float package

```
242 \caption@ifpackage{float}{floatc@plain}{}{%
243   \ifx\floatc@plain\relax
244     \PackageWarning{caption2}{%
245       Option 'float' was set but there is no float package loaded}
246   \else
247     \PackageInfo{caption2}{float package v1.2 (or newer) detected}
```

`\caption@floatc` First we define a helper macro to typeset the caption via `\usecaptionstyle`, the 1st parameter is the caption style name, the 2nd and 3rd are the caption label and text.

`caption2` has the goal not to modify the output just by loading it (without options), therefore we have to be tricky here to support `\@fs@cfont` which is in fact the same as our `\captionlabelfont`. So we test if a `\captionlabelfont` has been set by the user – if not `\@fs@cfont` will be used, otherwise `\captionlabelfont`.

```
248   \newcommand\caption@floatc[3]{%
249     \ifx\captionlabelfont\@empty
250       \let\captionlabelfont\@fs@cfont
251     \fi
252     \captionlinewidth\hsize
253     \realcaptionwidth\hsize
```

```

254     \def\captionlabel{#2}%
255     \def\captiontext{#3}%
256     \usecaptionstyle{#1}}

```

`\floatc@plain` Now we can redefine the caption code of the float package. Here we redefine `\floatc@plain` to use our caption code, so plain and boxed float types will use the actual caption style set by the user.

```

257     \renewcommand*\floatc@plain{\caption@floatc{\caption@style}}

```

`\floatc@ruled` The support of the ruled float type is a little more complex. First we define a caption style ‘ruled’ so the end-user can change this caption style afterwards. If the (obsolete) option ‘ruled’ is set, we define it in a caption v1.x compatible way, otherwise we define it in a float compatible way.

Then we redefine `\floatc@ruled` so the caption style ‘ruled’ will be used.

```

258     \ifcaption@ruled
259         \dummycaptionstyle{ruled}{\onelinecaptionsfalse\setcaptionmargin{\z@}}%
260     \else
261         \newcaptionstyle{ruled}{%
262             \ifcaptionlabel
263                 {\@fs@cfont\captionlabel}\space%
264             \fi\captiontext\par}%
265     \fi
266     \renewcommand*\floatc@ruled{\caption@floatc{ruled}}

```

`\caption@of` Typesetting captions outside floats is not so easy with redefined floats, because

- The caption code of the float package needs not only `\@capttype` defined, but `\@fs@capt` (the command which will typeset the caption itself) either.
- The caption is only saved within a `\vbox`, so the float package can typeset the caption later at it’s float style specific place (that means at top or at the bottom of the float).

Here is the new code: First we check if it’s a restyled float by checking if `\fst@<floattype>` is defined. If yes, we use this command (it will define `\@fs@capt`). Then we execute `\@float@setevery`, if it exists (that means we are dealing with the float package 1.3 or newer here). Now comes the basic trick: We redefine the caption typesetting command `\@fs@capt`, so it will close the `\vbox`, typeset the caption outside the `vbox` and finally start the group again so the original `\@fs@capt` is happy with closing the group.

```

267     \renewcommand*\caption@of[2]{\def\@capttype{#2}%
268         \@ifundefined{fst@#2}{}{%
269             \@nameuse{fst@#2}%
270             \@ifundefined{@float@setevery}{}{\@float@setevery{#2}}%
271             \let\caption@fs@capt\@fs@capt
272             \let\@fs@capt\caption@of@float}%
273     #1}

```

```

274 \newcommand\caption@of@float[2]{\egroup
275 \vskip\abovecaptionskip
276 \normalsize\caption@fs@capt{#1}{#2}%
277 \vskip\belowcaptionskip
278 \bgroup}%

279 \fi}

```

## 1.7.2 Support of the longtable package

```

280 \caption@ifpackage{longtable}{LT@makecaption}{}%
281 \ifx\LT@makecaption\relax
282 \PackageWarning{caption2}{%
283 Option 'longtable' was set but there is no longtable package loaded}
284 \else
285 \PackageInfo{caption2}{longtable package v3.15 (or newer) detected}

```

\LT@makecaption David Carlisle was so kind to introduce a macro called \LT@makecaption in version 3.15 of the longtable package which typeset the caption and can be easily redefined.

This is the original definition:

```

\def\LT@makecaption#1#2#3{%
\LT@mcol\LT@cols c{\hbox to\z@{\hss\parbox[t]\LTcapwidth{%
  \typeset #1{#2: }#3 as caption}
\endgraf\vskip\baselineskip}%
\hss}}

```

So we do here: First we define a new (dummy) caption style 'longtable', than we redefine \LT@makecaption so this style will be used. (Remember: #1 is \@gobble in star form of \caption, and \@firstofone otherwise.)

```

286 \dummycaptionstyle{longtable}{%
287 \renewcommand\LT@makecaption[3]{%
288 \LT@mcol\LT@cols c{\hbox to\z@{\hss\parbox[t]\hsize{%
289 \ifignoreLTcapwidth
290 \else
291 \setcaptionwidth\LTcapwidth
292 \fi
293 \captionlinewidth\hsize
294 \realcaptionwidth\hsize
295 \captionlabelfalse#1\captionlabeltrue
296 \def\captionlabel{#2}%
297 \def\captiontext{#3}%
298 \usecaptionstyle{longtable}%
299 \endgraf\vskip\baselineskip}%
300 \hss}}
301 \fi}

```

### 1.7.3 Support of the subfigure package

Some of the following code will not work within `\if`, because of the (yet) undefined `\ifxxx`. So we simply define the critical code within the helper commands `\setsubcapstyle` and `\caption@makesubcaption` already here.

`\setsubcapstyle` This sets the `subcaptionstyle` to a appropriate value.

If `\ifsubcapraggedright` is undefined (it was introduced into v2.1 of the subfigure package) we define it first.

```
302 \newcommand*\setsubcapstyle{%
303   \@ifundefined{subcapraggedright}{false}{%
304     \newif\ifsubcapraggedright}{}%
305   \ifsubcaphang
306     \ifsubcapcenter
307       \subcapstyle{hang+center}%
308     \else\ifsubcapcenterlast
309       \subcapstyle{hang+centerlast}%
310     \else\ifsubcapraggedright
311       \subcapstyle{hang+flushleft}%
312     \else
313       \subcapstyle{hang}%
314     \fi\fi\fi
315   \else\ifsubcapcenter
316     \subcapstyle{center}%
317   \else\ifsubcapcenterlast
318     \subcapstyle{centerlast}%
319   \else\ifsubcapraggedright
320     \subcapstyle{flushleft}%
321   \else
322     \subcapstyle{normal}%
323   \fi\fi\fi\fi}
```

`\caption@makesubcaption` This will typeset the subcaption. We just set all our `\captionxxx` values to the values of `\subcapxxx` and typeset the caption like subfigure within a `\hbox`, but with the help of `\usecaptionstyle`.

But this is not as easy as it seems. We typeset the caption like this:

```
\captionfont
  {\captionlabelfont\captionlabel\captionlabeldelim}%
\captionlabelsep\captiontext
```

Within subfigure 2.0 the caption will be set quite similar to:

```
\subcapsize
  {\subcaplabelfont\captionlabel}%
\space\captiontext
```

But within subfigure 2.1 this has changed to:

```

\subcapsize
  {\subcaplabelfont\captionlabel}%
\hskip\subfiglabelskip
  {\subcapfont\captiontext}}

```

So we have to be tricky here: We set `\captionlabelfont` to `\normalfont` plus `\subcapsize` & `\subcaplabelfont`, so the font setting in `\captionfont` will not affect the caption label in subfigure captions.

Note that `\hfil` has changed to `\hss` from subfigure 2.0 to 2.1, so we use `\caption@subfig@hss` instead. (We will define this later on.)

```

324 \newcommand\caption@makesubcaption[2]{%
325   \renewcommand*\captionfont{\subcapsize\subcapfont}%
326   \renewcommand*\captionlabelfont{\normalfont\subcapsize\subcaplabelfont}%
327   \let\captionlabeldelim\subcaplabeldelim
328   \let\captionlabelsep\subcaplabelsep
329   \ifsubfigcapwidth\captionwidthtrue\else\captionwidthfalse\fi
330   \setlength\captionmargin\subfigcapmargin
331   \setlength\captionwidth\subfigcapwidth
332   \captionindent\subcapindent
333   \ifsubcapnoonline\onelinecaptionsfalse\else\onelinecaptionstrue\fi
334   \hbox to\@tempdima{%
335     \caption@subfig@hss\parbox[t]\@tempdima{%
336       \captionlinewidth\@tempdima
337       \realcaptionwidth\@tempdima
338       \captionlabeltrue
339       \def\captionlabel{#1}%
340       \def\captiontext{\ignorespaces #2}%
341       \usecaptionstyle\caption@substyle}%
342     \caption@subfig@hss}}

```

If the subfigure support is not needed, we throw the helper macros in the garbage can.

```

343 \caption@ifpackage{subfigure}{@makesubfigurecaption}{%
344   \let\setsubcapstyle\undefined
345   \let\caption@makesubcaption\undefined}{%
346   \ifx\@makesubfigurecaption\relax
347     \PackageWarning{caption2}{%
348       Option 'subfigure' was set but there is no subfigure package loaded}
349     \let\setsubcapstyle\undefined
350     \let\caption@makesubcaption\undefined
351   \else

```

Some stuff has changed from version 2.0 to 2.1 of the subfigure package, so we make a branch here. If `\subcapfont` is undefined we assume v2.0, otherwise we assume v2.1 or newer.

```

352   \ifx\subcapfont\undefined
353     \PackageInfo{caption2}{subfigure package v2.0 detected}

```

```

\subcapfont We define \subcapfont here so we can use it later in common code for subfigure v2.0
and v2.1 (or newer).
354     \let\subcapfont\@empty

\subfigcapwidth Analogous to \captionwidth, \setcaptionmargin, and \setcaptionwidth
\setsubcapmargin we define \subfigcapwidth, \setsubcapmargin, and \setsubcapwidth.
\setsubcapwidth Note: \subfigcapmargin is a command in v2.0 of subfigure. So we make
\subfigcapwidth a command, too.
355     \newcommand*\subfigcapwidth{\z@}
356     \newcommand*\setsubcapmargin{%
357         \subfigcapwidthfalse
358         \renewcommand*\subfigcapmargin}
359     \newcommand*\setsubcapwidth{%
360         \subfigcapwidthtrue
361         \renewcommand*\subfigcapwidth}

\subcaplabelsep Analogous to \captionlabelsep we define \subcaplabelsep.
362     \newcommand*\subcaplabelsep{\space}

\caption@subfig@hss This will be uses within the caption code itself.
363     \let\caption@subfig@hss\hfil

364     \else
365     \PackageInfo{caption2}{subfigure package v2.1 (or newer) detected}

\subfigcapwidth Analogous to \captionwidth, \setcaptionmargin, and \setcaptionwidth
\setsubcapmargin we define \subfigcapwidth, \setsubcapmargin, and \setsubcapwidth.
\setsubcapwidth Note: \subfigcapmargin is a length in v2.1 of subfigure. So we make \subfigcapwidth
a length, too.
366     \newdimen\subfigcapwidth
367     \newcommand*\setsubcapmargin{%
368         \subfigcapwidthfalse
369         \setlength\subfigcapmargin}
370     \newcommand*\setsubcapwidth{%
371         \subfigcapwidthtrue
372         \setlength\subfigcapwidth}

\subcaplabelsep Analogous to \captionlabelsep we define \subcaplabelsep.
373     \newcommand*\subcaplabelsep{\hskip\subfiglabelskip}

\caption@subfig@hss This will be uses within the caption code itself.
374     \let\caption@subfig@hss\hss
375     \fi

```

Here starts the common code for subfigure v2.0 and v2.1.

```
\ifsubfigcapwidth Analogous to \ifcaptionwidth, \captionindent & \captionlabeldelim
\subcapindent we define \ifsubfigcapwidth, \subcapindent & \subcaplabeldelim
\subcaplabeldelim
376 \newif\ifsubfigcapwidth
377 \newdimen\subcapindent
378 \newcommand*\subcaplabeldelim{}

\subcapstyle Analogous to \captionstyle we define \subcapstyle and set it (via \setsubcapstyle)
to a appropriate value.
379 \newcommand*\subcapstyle[1]{%
380 \expandafter\ifx\csname caption@#1\endcsname\relax
381 \PackageError{caption2}{Undefined caption style '#1'}{\caption@eh}%
382 \else
383 \def\caption@substyle{#1}%
384 \fi}
385 \setsubcapstyle
```

```
\@thesubfigure The subfigure package makes use of \subcaplabelfont and \subfiglabelskip
\@thesubtable within its \@thesubxxx macros. This is totally in contrast to the way the caption2
package handle these settings. So we redefine the \@thesubxxx to be just the plain
label and nothing else.
```

```
386 \renewcommand*\@thesubfigure{\thesubfigure}
387 \renewcommand*\@thesubtable{\thesubtable}
```

```
\@makesubfigurecaption Now we are ready to redefine \@makesubfigurecaption.
```

```
\@makesubtablecaption
388 \let\@makesubfigurecaption\caption@makesubcaption
389 \let\@makesubtablecaption\caption@makesubcaption
390 \fi}
```

That's all folks!

```
391 \let\caption@ifpackage\undefined
```

## References

- [1] Anselm Lingnau: *An Improved Environment for Floats*, 2001/11/08
- [2] David Carlisle: *The longtable package*, 2000/10/22
- [3] Sebastian Rahtz and Leonor Barroca: *A style option for rotated objects in L<sup>A</sup>T<sub>E</sub>X*, 1997/09/26
- [4] Steven Douglas Cochran: *The subfigure package*, 2002/02/14

- [5] Michel Goossens, Frank Mittelbach and Alexander Samarin: *The L<sup>A</sup>T<sub>E</sub>X Companion*, Addison-Wesley, Reading, Massachusetts, 1994.
- [6] Anne Brüggemann-Klein: *Einführung in die Dokumentverarbeitung*, B.G. Teubner, Stuttgart, 1989
- [7] Helmut Kopka: *L<sup>A</sup>T<sub>E</sub>X- Erweiterungsmöglichkeiten*, 3. überarbeitete Auflage, Addison-Wesley, Bonn, 1991
