# Supplementary material for: Reentrant phenomenon in the exactly solvable mixed spin-1/2 and spin-1 Ising-Heisenberg model on diamond-like decorated planar lattices
Source: arXiv:0909.4191 source file (2009-09-23)
Supplement: Supplementary file 4 [file subfig.pdf]

# The **Subfig** Package\*

Steven Douglas Cochran

Digital Mapping Laboratory, School of Computer Science  
Carnegie-Mellon University, 5000 Forbes Avenue  
Pittsburgh, PA 15213-3890  
USA

`cochran@ieee.org`  
`sdc@cs.cmu.edu`

2005/07/05

## **Abstract**

This article documents the  $\LaTeX$  package ‘**subfig**’, which provides support for the inclusion of small, ‘sub’, figures and tables. It simplifies the positioning, captioning and labeling of such objects within a single **figure** or **table** environment and to continue a **figure** or **table** across multiple pages. In addition, this package allows such sub-captions to be written to a List-of-Floats page as desired. The ‘**subfig**’ package requires the ‘**caption**’ package by H.A. Sommerfeldt and replaces the older ‘**subfigure**’ package.

---

\*This paper documents the **subfig** package version 1.3, last revised 2005/06/28.



## Contents

|          |                                                                                                                               |           |
|----------|-------------------------------------------------------------------------------------------------------------------------------|-----------|
| <b>1</b> | <b>Introduction</b>                                                                                                           | <b>1</b>  |
| 1.1      | Do You Need This Package? . . . . .                                                                                           | 1         |
| <b>2</b> | <b>Package Commands</b>                                                                                                       | <b>2</b>  |
| 2.1      | Preamble Commands . . . . .                                                                                                   | 2         |
| 2.1.1    | The <code>\usepackage</code> Command . . . . .                                                                                | 2         |
| 2.1.2    | The <code>\newsfloat</code> Command . . . . .                                                                                 | 3         |
| 2.1.3    | The <code>\DeclareCaptionListOfFormat</code> Command . . . . .                                                                | 3         |
| 2.1.4    | The <code>\DeclareSubrefFormat</code> Command . . . . .                                                                       | 3         |
| 2.2      | General Commands . . . . .                                                                                                    | 4         |
| 2.2.1    | The <code>\subfloat</code> Command . . . . .                                                                                  | 4         |
| 2.2.2    | The <code>\subref</code> Command . . . . .                                                                                    | 4         |
| 2.2.3    | The <code>\ContinuedFloat</code> Command . . . . .                                                                            | 5         |
| 2.2.4    | The <code>\listsubcaptions</code> Command . . . . .                                                                           | 6         |
| 2.2.5    | The <code>\captionsetup</code> Command . . . . .                                                                              | 6         |
| <b>3</b> | <b>Options: Keywords and Values</b>                                                                                           | <b>7</b>  |
| 3.1      | Options from the <code>caption</code> Package . . . . .                                                                       | 7         |
| 3.1.1    | The <code>caption</code> Font Settings . . . . .                                                                              | 10        |
| 3.1.2    | The <code>caption</code> Shape Settings . . . . .                                                                             | 10        |
| 3.1.3    | The <code>caption</code> Justification Options . . . . .                                                                      | 28        |
| 3.1.4    | The <code>caption</code> Label Options . . . . .                                                                              | 28        |
| 3.1.5    | The <code>caption</code> Position Option . . . . .                                                                            | 31        |
| 3.2      | Options from the <code>subfig</code> Package . . . . .                                                                        | 32        |
| 3.2.1    | The <code>subfig</code> Configuration Specification . . . . .                                                                 | 32        |
| 3.2.2    | The <code>subfig</code> List-of-Floats Specification . . . . .                                                                | 33        |
| 3.2.3    | The <code>subfig</code> Layout . . . . .                                                                                      | 33        |
| 3.2.4    | The <code>subfig</code> Package Startup . . . . .                                                                             | 34        |
| <b>4</b> | <b>Compatibility With Other Packages.</b>                                                                                     | <b>36</b> |
| 4.1      | <code>caption</code> Package . . . . .                                                                                        | 36        |
| 4.2      | <code>float</code> Package . . . . .                                                                                          | 36        |
| 4.3      | <code>floatrow</code> Package . . . . .                                                                                       | 37        |
| 4.4      | <code>verbatim</code> and <code>fancyvrb</code> packages . . . . .                                                            | 38        |
| 4.5      | <code>IEEEtrns</code> Class . . . . .                                                                                         | 39        |
| 4.6      | Other Packages . . . . .                                                                                                      | 39        |
| 4.7      | Backward Compatibility with the <code>Subfigure</code> Package . . . . .                                                      | 40        |
| <b>5</b> | <b>Some Examples</b>                                                                                                          | <b>41</b> |
| 5.1      | A Simple Example . . . . .                                                                                                    | 42        |
| 5.2      | A More Advanced Example . . . . .                                                                                             | 43        |
| 5.3      | An Example Without Sub-caption Text . . . . .                                                                                 | 44        |
| 5.4      | Another Example . . . . .                                                                                                     | 44        |
| <b>6</b> | <b>Frequently Asked Questions (FAQs)</b>                                                                                      | <b>46</b> |
| 6.1      | “My sub-floats are not aligned along their bottoms. Why?” . . . . .                                                           | 46        |
| 6.2      | “How can I get my floats/sub-floats to line up the way I want?” . . . . .                                                     | 46        |
| 6.3      | “I have too many sub-floats for one page, How can I spread them over two or more pages and continue the numbering?” . . . . . | 46        |
| 6.4      | “Why do I get a garbled caption or an error when I use square brackets?” . . . . .                                            | 46        |
| 6.5      | “How do I make my subcaptions print on the List-of-Floats pages?” . . . . .                                                   | 47        |
| 6.6      | “I set an option and it had no effect. What is happening?” . . . . .                                                          | 47        |
| 6.7      | “How do I make a change in the settings for just a single float?” . . . . .                                                   | 47        |
| 6.8      | “How do I put text labels on an imported sub-float?” . . . . .                                                                | 47        |

|          |                                                                                                |           |
|----------|------------------------------------------------------------------------------------------------|-----------|
| 6.9      | “I want my sub-floats to be ordered by column rather than by row, how do I do that?” . . . . . | 48        |
| 6.10     | “How do I put a verbatim environment in a sub-float?” . . . . .                                | 48        |
| <b>7</b> | <b>The Code</b> . . . . .                                                                      | <b>49</b> |
| 7.1      | Identification . . . . .                                                                       | 49        |
| 7.2      | Check for Nasty Classes . . . . .                                                              | 49        |
| 7.3      | Load The Caption Package . . . . .                                                             | 49        |
| 7.3.1    | Load The Keyval Package and Scan Options . . . . .                                             | 49        |
| 7.3.2    | Load and Extend the Caption Package . . . . .                                                  | 50        |
| 7.4      | Options Processing . . . . .                                                                   | 52        |
| 7.5      | Generalized List-of-Floats . . . . .                                                           | 53        |
| 7.6      | Create New Sub-floats . . . . .                                                                | 54        |
| 7.7      | Layout Parameters . . . . .                                                                    | 54        |
| 7.8      | Process the Package Options . . . . .                                                          | 55        |
| 7.9      | Define the Sub-float Layout . . . . .                                                          | 56        |
| 7.10     | Use the Caption Package to Build the Sub-float Captions . . . . .                              | 59        |
| 7.11     | Subfig Caption Processing for the List-of-Floats Files . . . . .                               | 60        |
| 7.12     | Sub-float Label Handling . . . . .                                                             | 61        |
| 7.13     | Support for Continued Figures . . . . .                                                        | 63        |
| 7.14     | Automate the Sub-float Listings . . . . .                                                      | 64        |
| 7.15     | Provide Compatibility with Other Packages . . . . .                                            | 65        |
| 7.15.1   | The Hyperref Package . . . . .                                                                 | 65        |
| 7.15.2   | The Float Package . . . . .                                                                    | 65        |
| 7.15.3   | The Fixltx2e Package . . . . .                                                                 | 65        |
| <b>8</b> | <b>Acknowledgments</b> . . . . .                                                               | <b>66</b> |

## List of Figures

|   |                                                                                                                                           |    |
|---|-------------------------------------------------------------------------------------------------------------------------------------------|----|
| 1 | Here are two figures side-by-side. . . . .                                                                                                | 2  |
| 2 | First. . . . .                                                                                                                            | 2  |
| 3 | Second. . . . .                                                                                                                           | 2  |
| 4 | Here are the first two figures of a continued figure. . . . .                                                                             | 5  |
| 5 | Levels at which keyword/values pairs may be set to apply to, or override earlier keyword/values pairs, for floats and sub-floats. . . . . | 7  |
| 6 | Float caption. . . . .                                                                                                                    | 10 |
|   | (a) Sub-float caption. . . . .                                                                                                            | 10 |
| 7 | Font size options. . . . .                                                                                                                | 10 |
|   | (a) Option <code>[font=Large]</code> . . . . .                                                                                            | 10 |
|   | (b) Option <code>[font=large]</code> . . . . .                                                                                            | 10 |
|   | (c) Option <code>[font=normalsize]</code> . . . . .                                                                                       | 10 |
|   | (d) Option <code>[font=small]</code> . . . . .                                                                                            | 10 |
|   | (e) Option <code>[font=footnotesize]</code> . . . . .                                                                                     | 10 |
|   | (f) Option <code>[font=scriptsize]</code> . . . . .                                                                                       | 10 |
| 8 | Other Font Options. . . . .                                                                                                               | 11 |
|   | (a) Option <code>[font={rm,md,up}]</code> . . . . .                                                                                       | 11 |
|   | (b) Option <code>[font={rm,md,it}]</code> . . . . .                                                                                       | 11 |
|   | (c) Option <code>[font={rm,md,sl}]</code> . . . . .                                                                                       | 11 |
|   | (d) Option <code>[font={rm,md,sc}]</code> . . . . .                                                                                       | 11 |
|   | (e) Option <code>[font={rm,bf,up}]</code> . . . . .                                                                                       | 11 |
|   | (f) Option <code>[font={rm,bf,it}]</code> . . . . .                                                                                       | 11 |
|   | (g) Option <code>[font={rm,bf,sl}]</code> . . . . .                                                                                       | 11 |
|   | (h) Option <code>[font={rm,bf,sc}]</code> . . . . .                                                                                       | 11 |

|    |                                                                                                       |    |
|----|-------------------------------------------------------------------------------------------------------|----|
|    | (i) Option [font={sf,md,up}]. . . . .                                                                 | 11 |
|    | (j) Option [font={sf,md,it}]. . . . .                                                                 | 11 |
|    | (k) Option [font={sf,md,sl}]. . . . .                                                                 | 11 |
|    | (l) Option [font={sf,md,sc}]. . . . .                                                                 | 11 |
|    | (m) Option [font={sf,bf,up}]. . . . .                                                                 | 11 |
|    | (n) Option [font={sf,bf,it}]. . . . .                                                                 | 11 |
|    | (o) Option [font={sf,bf,sl}]. . . . .                                                                 | 11 |
|    | (p) Option [font={sf,bf,sc}]. . . . .                                                                 | 11 |
|    | (q) Option [font={tt,md,up}]. . . . .                                                                 | 11 |
|    | (r) Option [font={tt,md,it}]. . . . .                                                                 | 11 |
|    | (s) Option [font={tt,md,sl}]. . . . .                                                                 | 11 |
|    | (t) Option [font={tt,md,sc}]. . . . .                                                                 | 11 |
|    | (u) Option [font={tt,bf,up}]. . . . .                                                                 | 11 |
|    | (v) Option [font={tt,bf,it}]. . . . .                                                                 | 11 |
|    | (w) Option [font={tt,bf,sl}]. . . . .                                                                 | 11 |
|    | (x) Option [font={tt,bf,sc}]. . . . .                                                                 | 11 |
| 9  | Options [singlelinecheck=false]. . . . .                                                              | 12 |
| 10 | Options [ ]. . . . .                                                                                  | 13 |
| 11 | Options [indentation=10pt,singlelinecheck=false]. . . . .                                             | 13 |
| 12 | Options [indentation=10pt]. . . . .                                                                   | 13 |
| 13 | Options [hangindent=10pt,singlelinecheck=false]. . . . .                                              | 14 |
| 14 | Options [hangindent=10pt]. . . . .                                                                    | 14 |
| 15 | Options [hangindent=10pt,indentation=10pt,<br>singlelinecheck=false]. . . . .                         | 14 |
| 16 | Options [hangindent=10pt,indentation=10pt]. . . . .                                                   | 14 |
| 17 | Options [parskip=5pt,singlelinecheck=false]. . . . .                                                  | 14 |
| 18 | Options [parskip=5pt]. . . . .                                                                        | 15 |
| 19 | Options [parskip=5pt,indentation=10pt,singlelinecheck=false]. . . . .                                 | 15 |
| 20 | Options [parskip=5pt,indentation=10pt]. . . . .                                                       | 15 |
| 21 | Options [parskip=5pt,hangindent=10pt,<br>singlelinecheck=false]. . . . .                              | 15 |
| 22 | Options [parskip=5pt,hangindent=10pt]. . . . .                                                        | 15 |
| 23 | Options [parskip=5pt,hangindent=10pt,indentation=10pt,<br>singlelinecheck=false]. . . . .             | 16 |
| 24 | Options [parskip=5pt,hangindent=10pt,indentation=10pt]. . . . .                                       | 16 |
| 25 | Options [format=hang,singlelinecheck=false]. . . . .                                                  | 16 |
| 26 | Options [format=hang]. . . . .                                                                        | 16 |
| 27 | Options [format=hang,indentation=10pt,singlelinecheck=false]. . . . .                                 | 17 |
| 28 | Options [format=hang,indentation=10pt]. . . . .                                                       | 17 |
| 29 | Options [format=hang,hangindent=10pt,<br>singlelinecheck=false]. . . . .                              | 17 |
| 30 | Options [format=hang,hangindent=10pt]. . . . .                                                        | 17 |
| 31 | Options [format=hang,hangindent=10pt,indentation=10pt,<br>singlelinecheck=false]. . . . .             | 18 |
| 32 | Options [format=hang,hangindent=10pt,indentation=10pt]. . . . .                                       | 18 |
| 33 | Options [format=hang,parskip=5pt,singlelinecheck=false]. . . . .                                      | 18 |
| 34 | Options [format=hang,parskip=5pt]. . . . .                                                            | 18 |
| 35 | Options [format=hang,parskip=5pt,indentation=10pt,<br>singlelinecheck=false]. . . . .                 | 19 |
| 36 | Options [format=hang,parskip=5pt,indentation=10pt]. . . . .                                           | 19 |
| 37 | Options [format=hang,parskip=5pt,hangindent=10pt,<br>singlelinecheck=false]. . . . .                  | 19 |
| 38 | Options [format=hang,parskip=5pt,hangindent=10pt]. . . . .                                            | 19 |
| 39 | Options [format=hang,parskip=5pt,hangindent=10pt,<br>indentation=10pt,singlelinecheck=false]. . . . . | 20 |

|    |                                                                                                                   |    |
|----|-------------------------------------------------------------------------------------------------------------------|----|
| 40 | Options [format=hang,parskip=5pt,hangindent=10pt,<br>indentation=10pt]. . . . .                                   | 20 |
| 41 | Options [margin=10pt,singlelinecheck=false]. . . . .                                                              | 20 |
| 42 | Options [margin=10pt]. . . . .                                                                                    | 20 |
| 43 | Options [margin=10pt,indentation=10pt,singlelinecheck=false]. . . . .                                             | 21 |
| 44 | Options [margin=10pt,indentation=10pt]. . . . .                                                                   | 21 |
| 45 | Options [margin=10pt,hangindent=10pt,<br>singlelinecheck=false]. . . . .                                          | 21 |
| 46 | Options [margin=10pt,hangindent=10pt]. . . . .                                                                    | 21 |
| 47 | Options [margin=10pt,hangindent=10pt,indentation=10pt,<br>singlelinecheck=false]. . . . .                         | 22 |
| 48 | Options [margin=10pt,hangindent=10pt,indentation=10pt]. . . . .                                                   | 22 |
| 49 | Options [margin=10pt,parskip=5pt,singlelinecheck=false]. . . . .                                                  | 22 |
| 50 | Options [margin=10pt,parskip=5pt]. . . . .                                                                        | 22 |
| 51 | Options [margin=10pt,parskip=5pt,indentation=10pt,<br>singlelinecheck=false]. . . . .                             | 23 |
| 52 | Options [margin=10pt,parskip=5pt,indentation=10pt]. . . . .                                                       | 23 |
| 53 | Options [margin=10pt,parskip=5pt,hangindent=10pt,<br>singlelinecheck=false]. . . . .                              | 23 |
| 54 | Options [margin=10pt,parskip=5pt,hangindent=10pt]. . . . .                                                        | 23 |
| 55 | Options [margin=10pt,parskip=5pt,hangindent=10pt,<br>indentation=10pt,singlelinecheck=false]. . . . .             | 24 |
| 56 | Options [margin=10pt,parskip=5pt,hangindent=10pt,<br>indentation=10pt]. . . . .                                   | 24 |
| 57 | Options [margin=10pt,format=hang,singlelinecheck=false]. . . . .                                                  | 24 |
| 58 | Options [margin=10pt,format=hang]. . . . .                                                                        | 24 |
| 59 | Options [margin=10pt,format=hang,indentation=10pt,<br>singlelinecheck=false]. . . . .                             | 25 |
| 60 | Options [margin=10pt,format=hang,indentation=10pt]. . . . .                                                       | 25 |
| 61 | Options [margin=10pt,format=hang,hangindent=10pt,<br>singlelinecheck=false]. . . . .                              | 25 |
| 62 | Options [margin=10pt,format=hang,hangindent=10pt]. . . . .                                                        | 25 |
| 63 | Options [margin=10pt,format=hang,hangindent=10pt,<br>indentation=10pt,singlelinecheck=false]. . . . .             | 26 |
| 64 | Options [margin=10pt,format=hang,hangindent=10pt,<br>indentation=10pt]. . . . .                                   | 26 |
| 65 | Options [margin=10pt,format=hang,parskip=5pt,<br>singlelinecheck=false]. . . . .                                  | 26 |
| 66 | Options [margin=10pt,format=hang,parskip=5pt]. . . . .                                                            | 26 |
| 67 | Options [margin=10pt,format=hang,parskip=5pt,<br>indentation=10pt,singlelinecheck=false]. . . . .                 | 27 |
| 68 | Options [margin=10pt,format=hang,parskip=5pt,<br>indentation=10pt]. . . . .                                       | 27 |
| 69 | Options [margin=10pt,format=hang,parskip=5pt,<br>hangindent=10pt,singlelinecheck=false]. . . . .                  | 27 |
| 70 | Options [margin=10pt,format=hang,parskip=5pt,<br>hangindent=10pt]. . . . .                                        | 27 |
| 71 | Options [margin=10pt,format=hang,parskip=5pt,<br>hangindent=10pt,indentation=10pt,singlelinecheck=false]. . . . . | 28 |
| 72 | Options [margin=10pt,format=hang,parskip=5pt,<br>hangindent=10pt,indentation=10pt]. . . . .                       | 28 |
| 73 | Options [justification=justified,singlelinecheck=false]. . . . .                                                  | 28 |
| 74 | Options [justification=centerfirst,singlelinecheck=false]. . . . .                                                | 29 |
| 75 | Options [justification=centerlast,singlelinecheck=false]. . . . .                                                 | 29 |
| 76 | Options [justification=centering,singlelinecheck=false]. . . . .                                                  | 29 |

|    |                                                                       |    |
|----|-----------------------------------------------------------------------|----|
| 77 | Options [justification=Centering,singlelinecheck=false]. . . . .      | 29 |
| 78 | Options [justification=raggedleft,singlelinecheck=false]. . . . .     | 29 |
| 79 | Options [justification=RaggedLeft,singlelinecheck=false]. . . . .     | 30 |
| 80 | Options [justification=raggedright,singlelinecheck=false]. . . . .    | 30 |
| 81 | Options [justification=RaggedRight,singlelinecheck=false]. . . . .    | 30 |
| 82 | Options [labelformat=empty]. . . . .                                  | 30 |
| 83 | Options [labelformat=simple]. . . . .                                 | 30 |
| 84 | Options [labelformat=parens]. . . . .                                 | 31 |
| 85 | Options [labelsep=none]. . . . .                                      | 31 |
| 86 | Options [labelsep=colon]. . . . .                                     | 31 |
| 87 | Options [labelsep=period]. . . . .                                    | 31 |
| 88 | Options [labelsep=space]. . . . .                                     | 32 |
| 89 | Options [labelsep=quad]. . . . .                                      | 32 |
| 90 | Options [labelsep=newline]. . . . .                                   | 32 |
| 91 | Sub-float Layout. . . . .                                             | 35 |
|    | (a) Standard layout (Sub-float: position=bottom). . . . .             | 35 |
|    | (b) Standard layout without a caption (Sub-float: position=bottom) .  | 35 |
|    | (c) Reversed layout (Sub-float: position=top). . . . .                | 35 |
|    | (d) Standard layout without a caption (Sub-float: position=top) . . . | 35 |
| 92 | Main Caption. . . . .                                                 | 39 |
|    | (a) Black box . . . . .                                               | 39 |
|    | (b) Caption 2. . . . .                                                | 39 |
| 93 | Three sub-floats. . . . .                                             | 42 |
|    | (a) First. . . . .                                                    | 42 |
|    | (b) Second figure. . . . .                                            | 42 |
|    | (c) Third. . . . .                                                    | 42 |
| 94 | Two sub-floats. . . . .                                               | 43 |
|    | 94.1 First. . . . .                                                   | 43 |
|    | 94.2 Second. . . . .                                                  | 43 |
| 95 | A set of four sub-floats. . . . .                                     | 45 |
| 96 | Two more sub-floats. . . . .                                          | 45 |
|    | (a) Big figure . . . . .                                              | 45 |
|    | (b) Small figure . . . . .                                            | 45 |

## List of Tables

|   |                                                                     |    |
|---|---------------------------------------------------------------------|----|
| 1 | Example of internals created by a \newsubfloat “subfigure”. . . . . | 3  |
| 2 | \subfloat calling arguments. . . . .                                | 4  |
| 3 | Keywords with defaults and values. . . . .                          | 8  |
| 4 | Example font attribute substitutions. . . . .                       | 12 |
| 5 | Subfig specific options. . . . .                                    | 33 |
| 6 | Results in Two Tables. . . . .                                      | 38 |
|   | (a) First Table of Results. . . . .                                 | 38 |
|   | (b) Second Table of Results. . . . .                                | 38 |

## List of Maps

|   |                                            |    |
|---|--------------------------------------------|----|
| 1 | This example shows two small maps. . . . . | 37 |
|   | 1a First map. . . . .                      | 37 |
|   | 1b Second map. . . . .                     | 37 |



## 1 Introduction

This package provides support for the manipulation and reference of small or ‘sub’ floats within a single floating (*e.g.*, `figure` or `table`) environment<sup>1</sup> It is convenient to use this package when your sub-floats are to be separately captioned, referenced, or when such sub-captions are to be included on a List-of-Floats page.

This package is a replacement for the `subfigure` package, from which it was derived. However, the new `subfig` package is not completely backward compatible (see section 4.7). Therefore, a new name was called for. The newer package is smaller and easier to use than the older package, however, it now uses the following additional packages:

- `caption` (required)
- `everysel` (optional)
- `keyval` (required)
- `ragged2e` (optional)

It will work without the `ragged2e` and `everysel` packages if you do not use the following justification options: ‘Center’, ‘RaggedRight’ and ‘RaggedLeft’. The other justification options ‘center’, ‘raggedright’ and ‘raggedleft’ will work without the above two packages.

**Note:** If the `ragged2e` package is present, than the `caption` package will load it and it will, in turn, load the `everysel` package. This happens whether or not you will be using the justification options that require it. If it cannot find the `ragged2e` package, than the `caption` package will print a message that ‘RaggedRight’, *etc.* will not be available.

### 1.1 Do You Need This Package?

Before using the `subfig` package, consider the following to see if you really need it.

1. If you simply want to center your figure on the page, then you can use `\centerline`, `\centering` or the `center` environment to do so, see [6, page 112].
2. If your figure has a short width or if you wrap your figure in a `\parbox` or a `minipage` of a short width, then you can place multiple figures or tables side-by-side<sup>2</sup>. For example, the following will put two images side-by-side in a single figure as shown in figure 1:

```
\begin{figure}%
  \centering
  \parbox{1.2in}{...figure code...}%
  \quad
  \begin{minipage}{1.2in}%
    ...figure code...
  \end{minipage}%
  \caption{Here are two figures side-by-side.}%
  \label{fig:1figs}%
\end{figure}
```

3. Finally, if you place the caption inside the `\parbox` or `minipage`, then the width of the caption will be limited to the width of the `parbox` or `minipage` as shown in figures 2 and 3:

```
\begin{figure}%
  \centering
```

---

<sup>1</sup>Section 4.2 describes how to add support for additional `float` environments.

<sup>2</sup>You might have to use the optional position arguments ‘[b]’ or ‘[t]’ if the figures are of different heights, see sections 5 and 6.1 as well as [6, page 218].

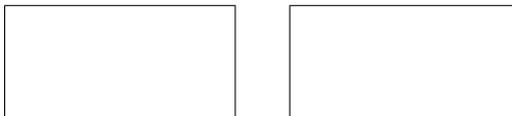

Figure 1: Here are two figures side-by-side.

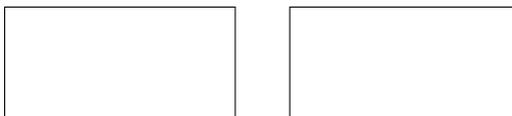

Figure 2: First.

Figure 3: Second.

```

\parbox{1.2in}{%
  ...figure code...
  \caption{First.}%
  \label{fig:2figsA}}%
\quad
\begin{minipage}{1.2in}%
  ...figure code...
  \caption{Second.}%
  \label{fig:2figsB}}%
\end{minipage}%
\end{figure}

```

For more information on typesetting figures and tables, see the book “The L<sup>A</sup>T<sub>E</sub>X Companion” by Mittelbach and Goossens [3, § 5 & 6] and the document “Using Imported Graphics in L<sup>A</sup>T<sub>E</sub>X 2<sub>ε</sub>” by Keith Reckdahl [5].

## 2 Package Commands

In this section, we describe the commands defined by the `subfig` package and three commands from the `caption` package that are needed or very useful in setting and changing the package options.

### 2.1 Preamble Commands

In the preamble of your L<sup>A</sup>T<sub>E</sub>X file, you may load the `subfig` package, define new and extended options and create new sub-floats. See the documentation for the `caption` package for other preamble commands that may be used to customize the caption portion of a sub-float.

#### 2.1.1 The `\usepackage` Command

```
\usepackage[<KV-list>]{subfig}
```

The optional argument list to the `subfig` package is in the form of a KV-list or “Key-Value list” (see [4] for more detail). The KV-list is composed of a comma-separated list of keywords with optional values. The keywords without a value indicate that a default value is to be used. This list is bound to the variable “subfloat” and is re-evaluated each time a `\subfloat` is encountered. These initial values may also be viewed, removed or changed with the `\showcaptionsetup[uniq]{subfloat}`, `\clearcaptionsetup[subfloat]` or `\captionsetup[subfloat]{<KV-list>}` commands.

Table 1: Example of internals created by a `\newsfloat` “subfigure”.

| Function/<br>Keyword           | Default                                                                                                  | Description                                                                            |
|--------------------------------|----------------------------------------------------------------------------------------------------------|----------------------------------------------------------------------------------------|
| <code>\c@subfigure</code>      | 0                                                                                                        | Internal counter variable.                                                             |
| <code>\c@subfigure@save</code> | 0                                                                                                        | Internal variable to save last counter value in case of a continued figure.            |
| <code>\subfigurename</code>    |                                                                                                          | Name prepended to the subcaption number (empty by default).                            |
| <code>\p@subfigure</code>      | <code>\thefigure</code>                                                                                  | Figure number prepended to the subcaption number in references via <code>\ref</code> . |
| <code>\thesubfigure</code>     | <code>\alph{subfigure}</code>                                                                            | Format of the subcaption number.                                                       |
| <code>\ext@subfigure</code>    | lof                                                                                                      | List-of-Floats file extension.                                                         |
| <code>\l@subfigure</code>      | <code>\@dottedxxxline{figure}</code><br><code>{lof}{2}{\sf@indent}</code><br><code>{\sf@numwidth}</code> | Format of List-of-Floats entry.                                                        |
| <code>\c@lofdepth</code>       | 1                                                                                                        | List-of-Floats depth variable.                                                         |
| <code>'lofdepth'</code>        | 2                                                                                                        | Sets <code>\c@lofdepth</code> .                                                        |

### 2.1.2 The `\newsfloat` Command

```
\newsfloat      \newsfloat[(KV-list)]{float-name}
```

This command creates all of the internal structures and commands needed to support the new subfloat (the corresponding float structure must already exist, see section 4.2). For instance when the “subfigure” is created the set of internals instantiated are shown in table 1.

The two internals `\subfigurename` and `\thesubfigure` are left for easy adjustment by the user, the rest should not be directly changed under normal circumstances. Note that you may change the values of any counter variable `\c@cnt` with the counter functions `\setcounter` or `\addtocounter` (see [6, pg. 194]). Also, the internals `\sf@indent` and `\sf@numwidth` may be change with the keywords `'listofindent'` and `'listofnumwidth'`, respectively.

Once the new float is created, the KV-list is placed at the top “level”. For example the options for the above *subfigure* are added to the name “subfigure”. See section 2.2.5 below, for more detail about option layers.

### 2.1.3 The `\DeclareCaptionListFormat` Command

```
\DeclareCaptionListFormat \DeclareCaptionListFormat{keyword value}{code}
```

The `\DeclareCaptionListFormat` command allows the specification of how the subcaption references are shown on the List-of-Floats pages. See section 3.2.2 for more details on setting up and adjusting the List-of-Floats entries.

The `{code}` section is passed two parameters that may be used or ignored. These are the value of the associated `\p@subfloati` type and the `\thesubfloati` respectively.

### 2.1.4 The `\DeclareSubrefFormat` Command

```
\DeclareSubrefFormat \DeclareSubrefFormat{keyword value}{code}
```

The `\DeclareSubrefFormat` command allows the specification of how the `\subref*` command generates its reference to a sub-caption label in the text.

Table 2: `\subfloat` calling arguments.

| Sub-float Command                                       | List-of-Floats Caption | Sub-float Caption |
|---------------------------------------------------------|------------------------|-------------------|
| <code>\subfloat{body}</code>                            |                        |                   |
| <code>\subfloat[ ]{body}</code>                         | (b) . . . . .          | (b)               |
| <code>\subfloat[Sub-caption.]{body}</code>              | (c) Sub-caption. . . . | (c) Sub-caption.  |
| <code>\subfloat[ ][Sub-caption.]{body}</code>           |                        | (d) Sub-caption.  |
| <code>\subfloat[ ][ ]{body}</code>                      |                        | (e)               |
| <code>\subfloat[List_entry.][Sub-caption.]{body}</code> | (f) List_entry. . . .  | (f) Sub-caption.  |
| <code>\subfloat[List_entry.][ ]{body}</code>            | (g) List_entry. . . .  | (g)               |

The `{code}` section is passed four parameters that may be used or ignored. The first two are the values of the associated `\p@<sub-float>` type and the `\the<sub-float>` (e.g., `\p@subfigure` and `\thesubfigure`), like the `\DeclareCaptionListOffFormat` command. The second two are the *raw* values of the `<float>` and the `<sub-float>` counters.

## 2.2 General Commands

These commands are available within the body of the paper and the commands `\captionsetup`, `\showcaptionsetup` and `\clearcaptionsetup` are available anytime after loading either the `caption` or `subfig` packages.

### 2.2.1 The `\subfloat` Command

```
\subfloat      \subfloat [⟨list_entry⟩] [⟨sub-caption⟩] {⟨body⟩}
```

This command creates the sub-float in the floating environment. In a `figure` environment it creates a subfigure. The required argument contains the sub-float object or “body”. This is the code that imports or creates the figure portion of the sub-float.

The two optional arguments control the caption. If only one optional argument is present, than a caption label is generated and if any text is included in the optional argument, than it becomes the caption argument.

Normally, if a caption is present, it is also included on the List-of-Floats page. However, if a second optional argument is present, than the first one controls what is on the List-of-Floats page and the second is the caption text. If the List-of-Floats argument is empty, than nothing is printed on the List-of-Floats page. Otherwise, if there is text in the List-of-Floats argument, than that text is used on the List-of-Floats page rather than the text in the other optional argument.

See table 2 for more detail on the `\subfloat` command’s arguments.

### 2.2.2 The `\subref` Command

```
\subref      \subref{⟨label⟩}  
\subref*    \subref*{⟨label⟩}
```

The `\subref` command is provided to give an alternative reference to a sub-float. The standard `\ref` command returns a label built by concatenating the `\p@float` + `\thesubfloat`, which is often of the form “1a”. The `\subref` command returns the label shown on the List-of-Floats page, which may be in the format “(a)” (i.e., if ‘listofformat=subparens’, see section 2.2.4). This may be combined with a reference to the main caption to give something of the form “1(a)”, or used within the main caption to refer to a specific local sub-float.

By default, the starred form of the command simply returns the `\thesubfloat` value, which, for sub-floats is usually something like “a”. However, this may be changed by setting ‘subrefformat’, similar to the above ‘listofformat’, to a predefined format (see table 3 or to a unique format defined with the `\DeclareSubrefFormat` command (section 2.1.4).

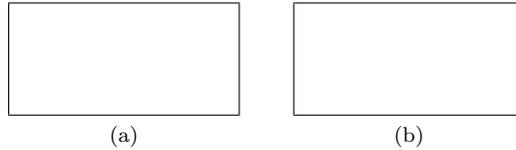

Figure 4: Here are the first two figures of a continued figure.

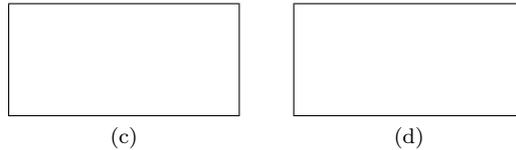

Figure 4: Here are the last two figures of a continued figure.

### 2.2.3 The `\ContinuedFloat` Command

`\ContinuedFloat`      `\ContinuedFloat`

It sometimes occurs, especially when using sub-floats, that a single figure needs to be continued across pages. The `\ContinuedFloat` command is placed at the beginning of the floating environment or after changing `\@capttype` inside the floating environment to make the next figure, table or other floating `\caption` a continuation of the last float `\caption` of the same type. It does this by saving the sub-float numbering internally and keeping the float numbering from advancing.

In order to keep subsequent float entries from appearing on the List-of-Floats page, you can use the `\caption` command with the optional argument present, but empty; as shown in figure 4 (and on the list-of-figures page).<sup>3</sup> We also suppress the sub-caption entry with the optional List-of-Floats page argument empty since there is no accompanying text.

```

\begin{figure}%
  \centering
  \subfloat[] [] {...figure code...}%
  \quad
  \subfloat[] [] {...figure code...}
  \caption{Here are the first two figures of a continued figure.}%
  \label{fig:cont}%
\end{figure}

\begin{figure}%
  \ContinuedFloat
  \centering
  \subfloat[] [] {...figure code...}%
  \quad
  \subfloat[] [] {...figure code...}
  \caption[] {Here are the last two figures of a continued figure.}%
  \label{fig:cont}%
\end{figure}

```

---

<sup>3</sup>Note: This only works if the `caption` package is active. If the `'caption=true'` option is used to load the `caption` package or the `subfig` package, than an empty optional argument to the `\caption` command generates a List-of-Floats entry with no caption text unless the document class redefines the `\caption` command otherwise.

### 2.2.4 The `\listsubcaptions` Command

`\listsubcaptions`      `\listsubcaptions`

The last command provided by the subfig package is the `\listsubcaptions`. This is automatically called in most cases by the `\caption` command and at the end of the float environment. However, the following example shows a rare situation in which the user will every have to use the `\listsubcaptions` command as shown in the definition of the `\zapytype` command.

```

\documentclass{article}
\usepackage[lofdepth,lotdepth]{subfig}
:
\makeatletter
\def\zapytype#1{%
    \listsubcaptions % Finish the last set of sub-floats before
    \def\@capttype{#1}}% switching to another float type.
\makeatother
:
\begin{document}
:
\listoffigures
\listoftables
\clearpage
\begin{table}%
\begin{center}%
\caption{Table caption.}%
\subfloat[Tab one]{X}\quad
\subfloat[Tab two]{X}\quad
%
\zapytype{figure}%
%
\subfloat[Fig one]{Y}\quad
\subfloat[Fig two]{Y}
\caption{Figure caption.}%
\end{center}%
\end{table}
:
\end{document}

```

**Hint:** Don't change the List-of-Floats page properties of any sub-floats until just before you use a `\subfloat` command, or just after you have executed a `\listsubcaptions` command. Otherwise, the wrong 'listofformat' or spacing might use the new values for sub-floats that have not been fully processed yet.

### 2.2.5 The `\captionsetup` Command

`\captionsetup`      `\captionsetup[<variable>]{<KV-list>}`

The `\captionsetup` command is actually part of the `caption` package, but is very important if you want to adjust some option in the subfig package. If the optional "variable" is left out, then the settings are made at the global level; otherwise, the settings are bound to the variable and executed just before being used.

There are four "levels" at which you can define options to apply to a sub-float (figure 5). The first level is the default or global values of the various options, which are

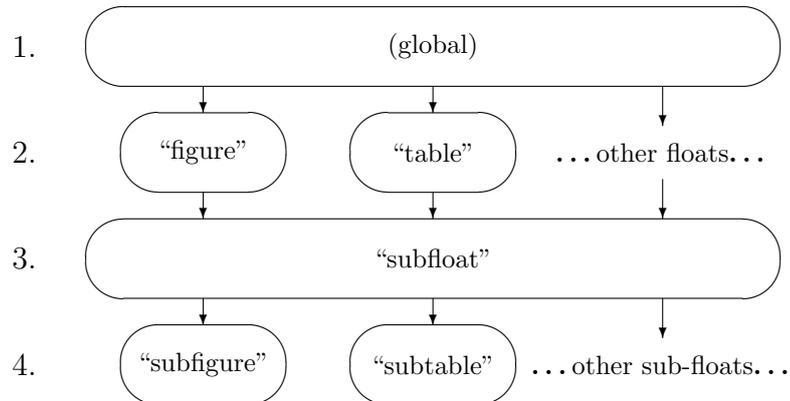

Figure 5: Levels at which keyword/values pairs may be set to apply to, or override earlier keyword/values pairs, for floats and sub-figures.

set either by the package, by a configuration file or by the optional Key-Value list in the `\usepackage` command when loading the `caption` package.

The second “level” consists of those options bound to the various floats. These are set by the `\captionsetup` with the optional argument set to the float name. For example, the command:

```
\captionsetup[table]{position=top}
```

would indicate that the “table” caption will come before its subfigures rather than after, as is the default.

The third “level” consists of those options bound to the special variable “subfloat”. These are value that hold across all sub-figures, but which are different than the global or float values. One such item is the “font” size, which is usually either null or **normal-sized**, but which is set to be **footnotesized** for the sub-figure captions.

The fourth “level” holds those options bound to a specific sub-figure, say “subfigure”. An example is the caption ‘position’ relative to the subfigure itself.

### 3 Options: Keywords and Values

Table 3 shows all of the formal keywords and values from both the `caption` and the `subfig` packages. These may be used on the `\usepackage` options line, or with the `\captionsetup` command.

If these are not desired, than they may be removed at the beginning of a configuration file with the command:

```
\clearcaptionsetup{subfloat}
```

The options are not added to the “subfloat” list until after the configuration file(s) are loaded.

#### 3.1 Options from the `Caption` Package

The `subfig` package uses the `caption` package commands to typeset the captions under each sub-figure. The settings used in the captions come from three sources. The first is the global settings provided by the `caption` package. The second is the keys and key/value pairs stored on the “subfloat” variable. The third is the keys and key/value

Table 3: Keywords with defaults and values. (Note: Entries enclosed in ‘[ ]’ indicate initial values rather than defaults.)

| PACKAGE            | KEYWORD              | DEFAULT<br>/ [INIT] | VALUE(S)                          |                                                                                                                                      |
|--------------------|----------------------|---------------------|-----------------------------------|--------------------------------------------------------------------------------------------------------------------------------------|
| Caption<br>Package | caption <sup>4</sup> | true                | <Boolean>                         |                                                                                                                                      |
|                    | config               | “caption.cfg”       | <filename>                        |                                                                                                                                      |
|                    | font (size)          | [default]           | default                           |                                                                                                                                      |
|                    | labelfont            | [default]           | scriptsize    rm    md    up      |                                                                                                                                      |
|                    | textfont             | [default]           | footnotesize    sf    bf    it    |                                                                                                                                      |
|                    |                      |                     | small            tt            sl |                                                                                                                                      |
|                    |                      |                     | normalsize                    sc  |                                                                                                                                      |
|                    |                      |                     | large                             |                                                                                                                                      |
|                    |                      |                     | Large                             |                                                                                                                                      |
|                    |                      | style               | [default]                         | default<br>ruled                                                                                                                     |
|                    |                      | singlelinecheck     | true                              | <Boolean>                                                                                                                            |
|                    |                      | format              | [default]                         | default<br>hang                                                                                                                      |
|                    |                      | indention           | [0pt]                             | <length>                                                                                                                             |
|                    |                      | hangindent          | [0pt]                             | <length>                                                                                                                             |
|                    |                      | width               | [\hspace]                         | <length>                                                                                                                             |
|                    |                      | margin              | [0pt]                             | <length>                                                                                                                             |
|                    |                      | parskip             | [5pt]                             | <length>                                                                                                                             |
|                    |                      | justification       | [default]                         | justified (default)<br>centering<br>centerfirst<br>centerlast<br>raggedleft<br>raggedright<br>Centering<br>RaggedLeft<br>RaggedRight |
|                    |                      | labelformat         | [default]                         | empty<br>simple (default)<br>parens                                                                                                  |
|                    |                      | aboveskip           | [10pt]                            | <length>                                                                                                                             |
|                    | belowskip            | [0pt]               | <length>                          |                                                                                                                                      |

pairs stored on (for figure sub-floats) the “subfigure” variable. In these three sources, if a key appears most recent value is used.

<sup>4</sup>The ‘caption’ option is only allowed on the caption or subfigure package option list. In addition, the ‘caption’ option can only be used in the subfigure package option list *if* the caption package has *not* been loaded.

<sup>5</sup>Only the ‘top’/‘above’ and ‘bottom’/‘below’ values are allowed for the ‘position’ option with the subfig package. If no value is set, than ‘bottom’ is assumed.

<sup>6</sup>Similar keywords are created automatically by the \newsfloat command, see section 2.1.2.

Table 3: Keywords with Defaults and Values (cont.).

| PACKAGE                       | KEYWORD                      | DEFAULT<br>/ [INIT] | VALUE(S)                                                      |
|-------------------------------|------------------------------|---------------------|---------------------------------------------------------------|
| Caption<br>Package<br>(cont.) | labelseparator<br>(labelsep) | [default]           | none<br>colon (default)<br>period<br>space<br>quad<br>newline |
|                               | position <sup>5</sup>        |                     | top (above)<br>bottom (below)                                 |
| Subfig<br>Package             | caption <sup>4</sup>         | true                | <Boolean>                                                     |
|                               | config                       | “subfig.cfg”        | <filename>                                                    |
|                               | lofdepth <sup>6</sup>        | 1                   | <number>                                                      |
|                               | lotdepth <sup>6</sup>        | 1                   | <number>                                                      |
|                               | listofformat                 | [subparens]         | empty<br>simple<br>parens<br>subsimple<br>subparens           |
|                               | subrefformat                 | [subsimple]         | empty<br>simple<br>parens<br>subsimple<br>subparens           |
|                               | listofindent                 | 3.8em               | <length>                                                      |
|                               | listofnumwidth               | 2.5em               | <length>                                                      |
|                               | farskip                      | 10pt                | <length>                                                      |
|                               | captionskip                  | 4pt                 | <length>                                                      |
|                               | topadjust                    | 0pt                 | <length>                                                      |
|                               | nearskip                     | 0pt                 | <length>                                                      |

Therefore, you can keep all of your common settings associated with the “subfloat” variable and, if needed, special settings for individual sub-float types (figure, table, etc.) on the associated variable (*e.g.*, “subfigure”, “subtable”, etc.).

The package options supplied with the `\usepackage` command are bound to the “subfloat” variable, and so, affect all of the sub-floats. The one exception to this is the ‘config’ or ‘config=filename’ option that is executed immediately. This is handy for two reasons, the first is that you only want to load a configuration file once (not every time you use a sub-float; and, second the ‘config’ keyword, without a value, will only load the “subfig.cfg” file when used on the options line, therefore you can set common options in both the float and sub-float captions with the command:

```
\usepackage[config, labelfont={sf,bf}, textfont=sf]{caption,subfig}
```

which will load the “caption.cfg” file and set the label and text fonts and also load the `subfig.cfg` file and set the sublabel and subtext fonts. Here we don’t use the ‘font’ key, since this is initialized with the default font sizes to be used and defaults to

[Sub-float Body]

(a) Sub-float caption.

Figure 6: Float caption.

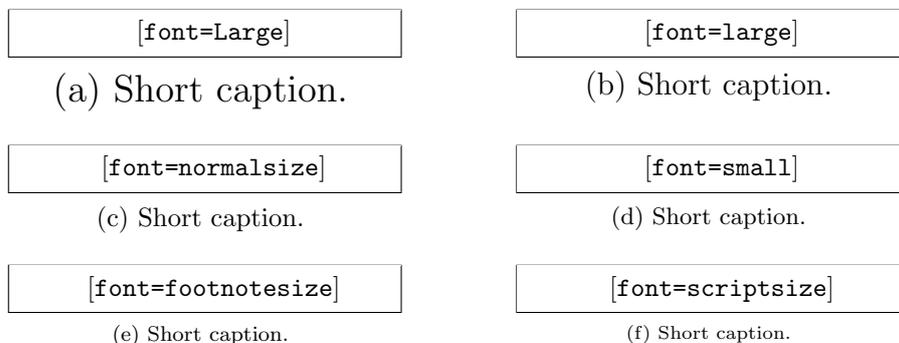

Figure 7: Font size options.

‘normalized’ for the float captions and to ‘footnotesized’ for the sub-float captions, as shown in figure 6.

Next we will review the options provided by the `caption` package. First the font settings, then the shape options, the justification and the other caption options that affect the sub-floats. Next, we review the options provided by the `subfig` package.

### 3.1.1 The Caption Font Settings

There are three font variables that can be set to control the float or sub-float captions. They are ‘font’, ‘labelfont’ and ‘textfont’. The “font” variable is applied to both the caption label and text; and is usually<sup>7</sup> used to specify the size of the caption and the other two variables are used to specify the other aspects of the font, the family, series and shape. The “labelfont” variable is used to specify the font used for the caption label and separator, while the “textfont” specifies that for the caption text.

Each of these variables can have one value from each of the four columns in the “VALUE” section of table 3 associated with the font keywords. If nothing is specified for one of the four sections, than that aspect of the current font is used.

Figures 7(a)–(f) show the effect of the font size options on the “font” variable.

Figures 8(a)–(x) show the effect of all combinations of the other font settings on the “textfont” variable. Note that not all combinations are necessarily available.<sup>8</sup> Where the specified font attributes are not available  $\LaTeX$  will substitute an alternate font. For instance, when compiling this file on one system,  $\LaTeX$  substituted alternate fonts for the requested ones in ten of the twenty-four cases (see table 4). Recompiling this documentation on your system and looking at the  $\LaTeX$  warnings will show you any combinations that are not available for you.

### 3.1.2 The Caption Shape Settings

There are seven options for setting the sub-caption shape or “format”. The default setting is produced by

<sup>7</sup>But not always, careful use of these three variables can produce useful effects. Their application is as:

```
{\font {\labelfont <label><separator>}{\textfont <text>}
```

<sup>8</sup>To modify the fonts used in your document and make specific combinations of family, shape and style available, see the NFSS documentation in The Latex Companion [3].

|                                                                                                                                                            |                                                                                                                                                                   |
|------------------------------------------------------------------------------------------------------------------------------------------------------------|-------------------------------------------------------------------------------------------------------------------------------------------------------------------|
| <div style="border: 1px solid black; padding: 2px; display: inline-block;">[font={rm,md,up}]</div><br>(a) Short caption.                                   | <div style="border: 1px solid black; padding: 2px; display: inline-block;">[font={rm,md,it}]</div><br>(b) <i>Short caption.</i>                                   |
| <div style="border: 1px solid black; padding: 2px; display: inline-block;">[font={rm,md,sl}]</div><br>(c) <i>Short caption.</i>                            | <div style="border: 1px solid black; padding: 2px; display: inline-block;">[font={rm,md,sc}]</div><br>(D) SHORT CAPTION.                                          |
| <div style="border: 1px solid black; padding: 2px; display: inline-block;">[font={rm,bf,up}]</div><br><b>(e) Short caption.</b>                            | <div style="border: 1px solid black; padding: 2px; display: inline-block;">[font={rm,bf,it}]</div><br><b>(f) <i>Short caption.</i></b>                            |
| <div style="border: 1px solid black; padding: 2px; display: inline-block;">[font={rm,bf,sl}]</div><br><b>(g) <i>Short caption.</i></b>                     | <div style="background-color: #cccccc; border: 1px solid black; padding: 2px; display: inline-block;">[font={rm,bf,sc}]</div><br><b>(h) Short caption.</b>        |
| <div style="border: 1px solid black; padding: 2px; display: inline-block;">[font={sf,md,up}]</div><br>(i) Short caption.                                   | <div style="background-color: #cccccc; border: 1px solid black; padding: 2px; display: inline-block;">[font={sf,md,it}]</div><br><b>(j) <i>Short caption.</i></b> |
| <div style="border: 1px solid black; padding: 2px; display: inline-block;">[font={sf,md,sl}]</div><br>(k) <i>Short caption.</i>                            | <div style="background-color: #cccccc; border: 1px solid black; padding: 2px; display: inline-block;">[font={sf,md,sc}]</div><br><b>(L) SHORT CAPTION.</b>        |
| <div style="border: 1px solid black; padding: 2px; display: inline-block;">[font={sf,bf,up}]</div><br><b>(m) Short caption.</b>                            | <div style="background-color: #cccccc; border: 1px solid black; padding: 2px; display: inline-block;">[font={sf,bf,it}]</div><br><b>(n) Short caption.</b>        |
| <div style="background-color: #cccccc; border: 1px solid black; padding: 2px; display: inline-block;">[font={sf,bf,sl}]</div><br><b>(o) Short caption.</b> | <div style="background-color: #cccccc; border: 1px solid black; padding: 2px; display: inline-block;">[font={sf,bf,sc}]</div><br><b>(p) Short caption.</b>        |
| <div style="border: 1px solid black; padding: 2px; display: inline-block;">[font={tt,md,up}]</div><br>(q) Short caption.                                   | <div style="border: 1px solid black; padding: 2px; display: inline-block;">[font={tt,md,it}]</div><br>(r) <i>Short caption.</i>                                   |
| <div style="border: 1px solid black; padding: 2px; display: inline-block;">[font={tt,md,sl}]</div><br>(s) <i>Short caption.</i>                            | <div style="border: 1px solid black; padding: 2px; display: inline-block;">[font={tt,md,sc}]</div><br>(T) SHORT CAPTION.                                          |
| <div style="background-color: #cccccc; border: 1px solid black; padding: 2px; display: inline-block;">[font={tt,bf,up}]</div><br>(u) Short caption.        | <div style="background-color: #cccccc; border: 1px solid black; padding: 2px; display: inline-block;">[font={tt,bf,it}]</div><br>(v) <i>Short caption.</i>        |
| <div style="background-color: #cccccc; border: 1px solid black; padding: 2px; display: inline-block;">[font={tt,bf,sl}]</div><br>(w) Short caption.        | <div style="background-color: #cccccc; border: 1px solid black; padding: 2px; display: inline-block;">[font={tt,bf,sc}]</div><br>(x) Short caption.               |

Figure 8: Other Font Options (shaded boxes indicate font combinations that were not available, see table 4).

```
\captionsetup[subfigure]{style=default, margin=0pt, parskip=0pt,
                        hangindent=0pt, indentation=0pt, singlelinecheck=true}
```

which is shown in figure 10. Figure 9 shows the same thing, but without setting the ‘singlelinecheck’ to true. You can see that the ‘singlelinecheck’ option only affects the short caption.

Table 4: Example font attribute substitutions.<sup>9</sup>

| Figure | Desired Options | Substitution Reason    | Actual Options |
|--------|-----------------|------------------------|----------------|
| 8(h)   | {rm,bf,sc}      | undefined              | {rm,bf,up}     |
| 8(j)   | {sf,md,it}      | unavailable in size 10 | {sf,md,sl}     |
| 8(l)   | {sf,md,sc}      | unavailable in size 10 | {rm,md,sc}     |
| 8(n)   | {sf,bf,it}      | undefined              | {sf,bf,up}     |
| 8(o)   | {sf,bf,sl}      | undefined              | {sf,bf,up}     |
| 8(p)   | {sf,bf,sc}      | undefined              | {sf,bf,up}     |
| 8(u)   | {tt,bf,up}      | unavailable in size 10 | {tt,md,up}     |
| 8(v)   | {tt,bf,it}      | unavailable in size 10 | {tt,md,it}     |
| 8(w)   | {tt,bf,sl}      | unavailable in size 10 | {tt,md,up}     |
| 8(x)   | {tt,bf,sc}      | unavailable in size 10 | {tt,md,up}     |

(a) Short caption.

(b) Non fuit causa cur postulare. Qui hoc intellegi potest? Naevio neque ex societatis ratione neque privatim quicumquam debuit Quinctius. Quis huic rei testis est? Idem qui acerrimus adversarius; in hanc rem te, te inquam, testem, Naevi, citabo.

Figure 9: Options [`singlelinecheck=false`].

Any or all of the other shape option may be used at one time, since they define orthogonal aspects of the caption shape. The other options are:

- ‘singlelinecheck’, (Boolean) which causes a caption that will fit on one line to be centered below the figure (actually, to use the singlelinecheck format);
- ‘indentation’, (length) which indents the caption text of each line of each paragraph (except the first line of the first paragraph);
- ‘hangindent’, (length) which indents the caption text of all but the first line of each paragraph;
- ‘parskip’, (length) which adds some extra space between separate paragraphs in a caption;
- ‘hang’, which causes the label to hang out to the left of the caption text, ‘normal’ turns it off; and,
- ‘margin’, (length) which sets extra space to either side of the caption, the option ‘width’ may also be used. This sets the margins to provide the requested width of the caption.<sup>10</sup>

Figures 9 thru 72 show all of the different combinations of these formats.

<sup>9</sup>This table may differ with different distributions of L<sup>A</sup>T<sub>E</sub>X and the choice of the base font families. Examine the L<sup>A</sup>T<sub>E</sub>X log for font warnings for your specific system.

<sup>10</sup>Internally, the initial width of the sub-float is set equal to the width of the sub-float body (see figure 91). This value is modified by either the ‘margin’ or the ‘width’, if defined (if both are defined than whichever is specified last is used). Note that the ‘width’ may be larger than the width of the sub-float body, or equivalently, the ‘width’ may be negative to provide more room for a caption if the sub-float body is small. The box holding the caption is centered relative to the sub-float body.

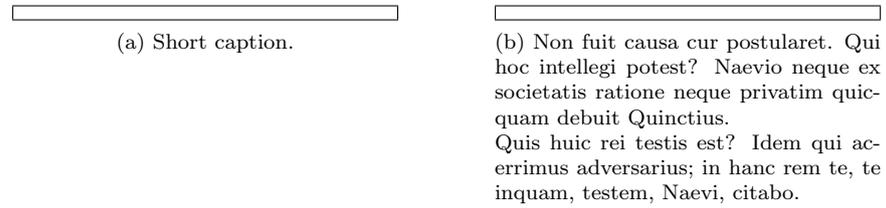

Figure 10: Options [ ].

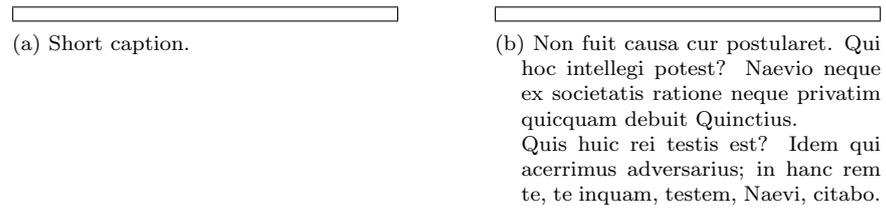

Figure 11: Options [indentation=10pt,singlelinecheck=false].

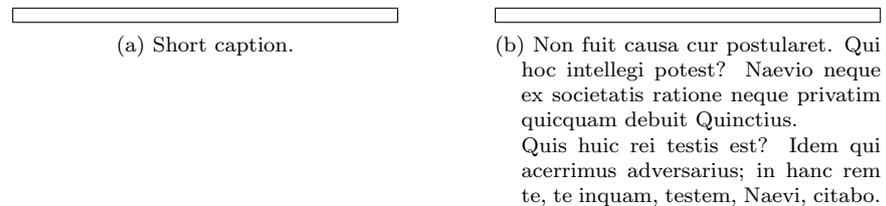

Figure 12: Options [indentation=10pt].

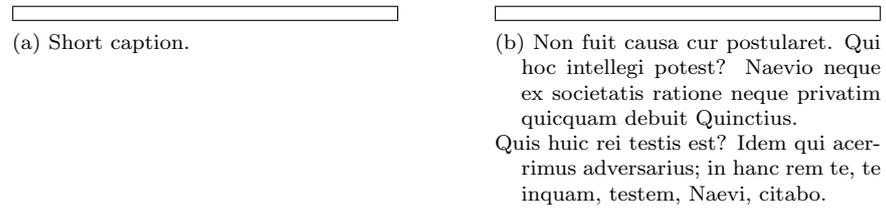

Figure 13: Options [hangindent=10pt, singlelinecheck=false].

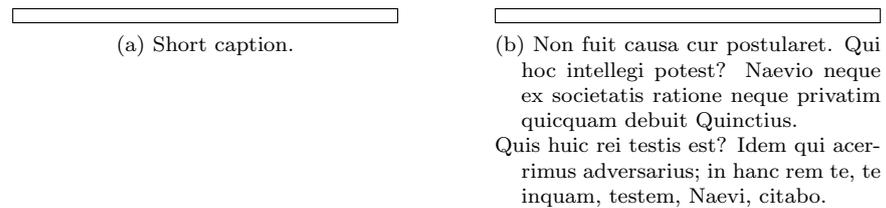

Figure 14: Options [hangindent=10pt].

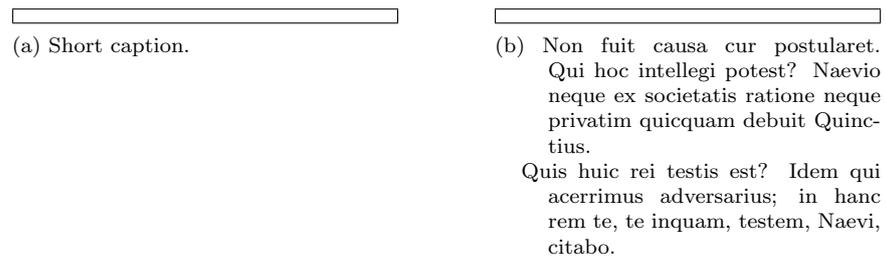

Figure 15: Options [hangindent=10pt, indention=10pt, singlelinecheck=false].

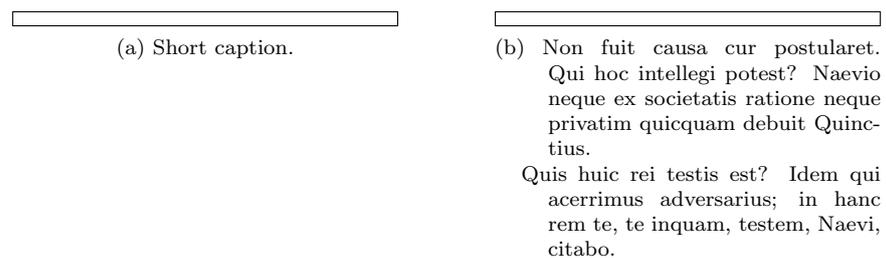

Figure 16: Options [hangindent=10pt, indention=10pt].

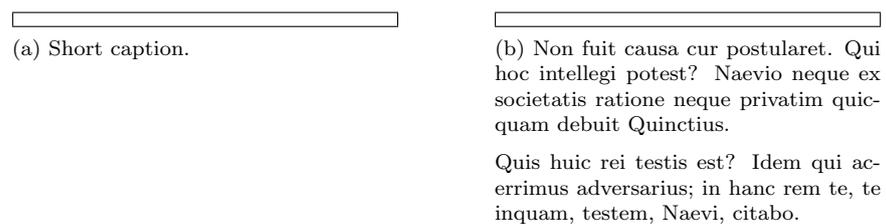

Figure 17: Options [parskip=5pt, singlelinecheck=false].

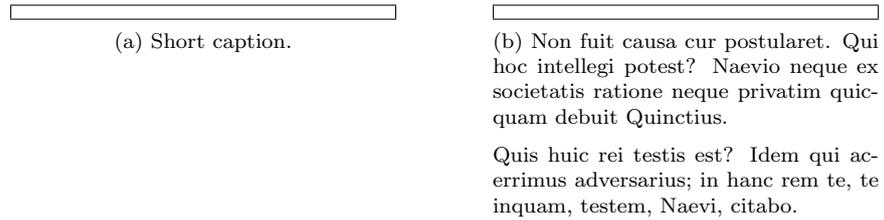

Figure 18: Options [parskip=5pt].

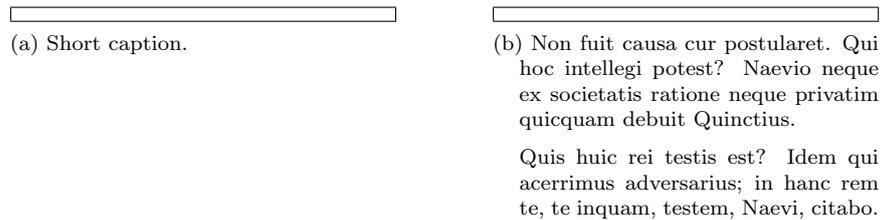

Figure 19: Options [parskip=5pt, indention=10pt, singlelinecheck=false].

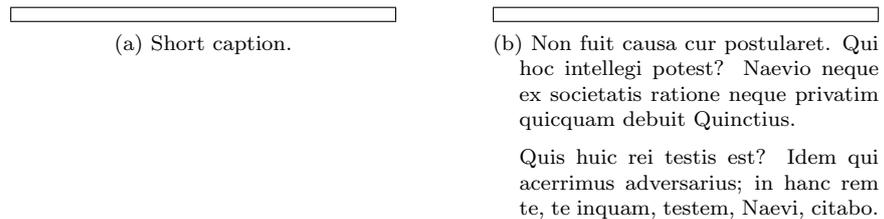

Figure 20: Options [parskip=5pt, indention=10pt].

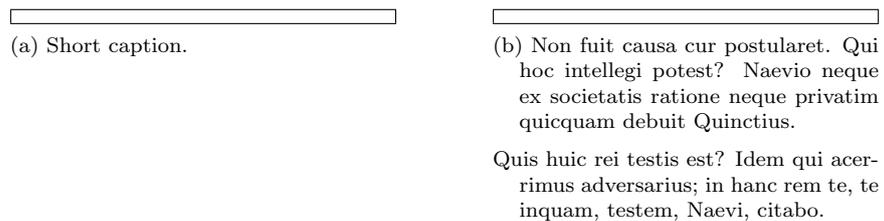

Figure 21: Options [parskip=5pt, hangindent=10pt, singlelinecheck=false].

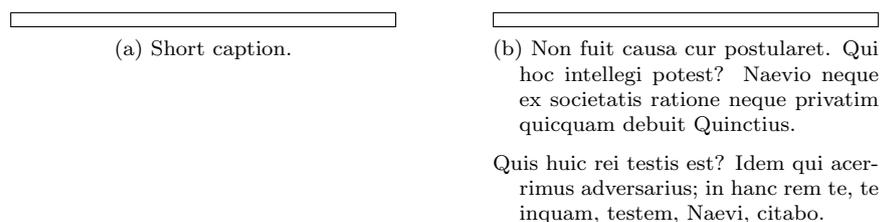

Figure 22: Options [parskip=5pt, hangindent=10pt].

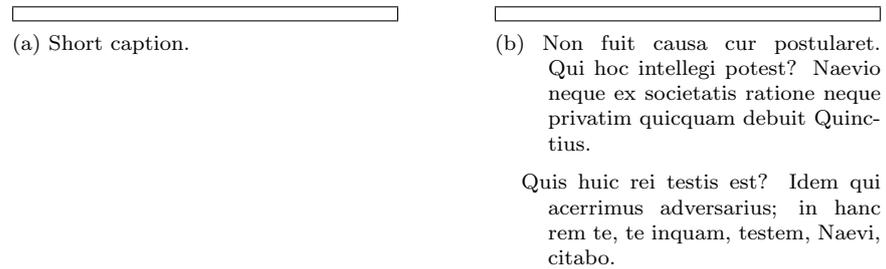

Figure 23: Options [parskip=5pt, hangindent=10pt, indention=10pt, singlelinecheck=false].

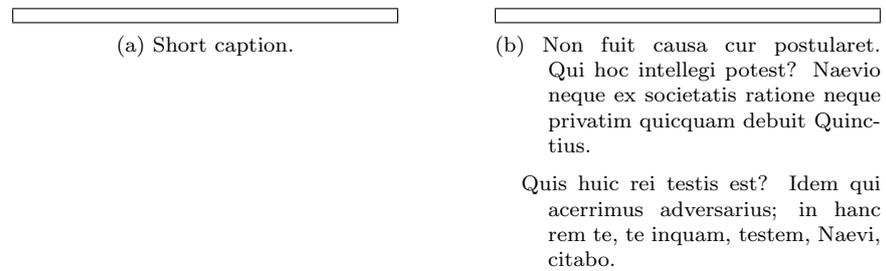

Figure 24: Options [parskip=5pt, hangindent=10pt, indention=10pt].

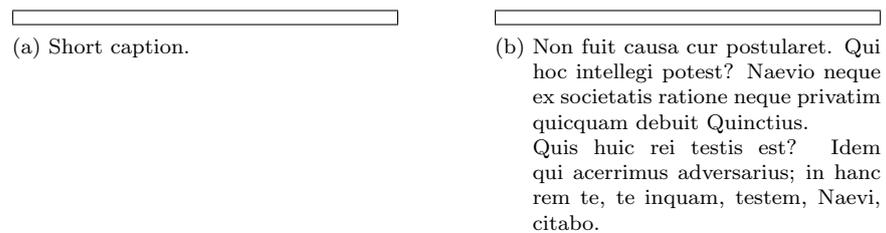

Figure 25: Options [format=hang, singlelinecheck=false].

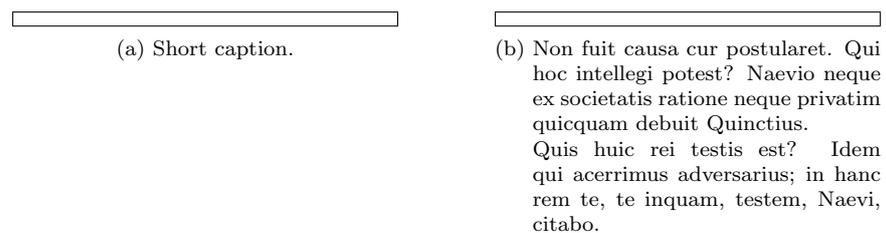

Figure 26: Options [format=hang].

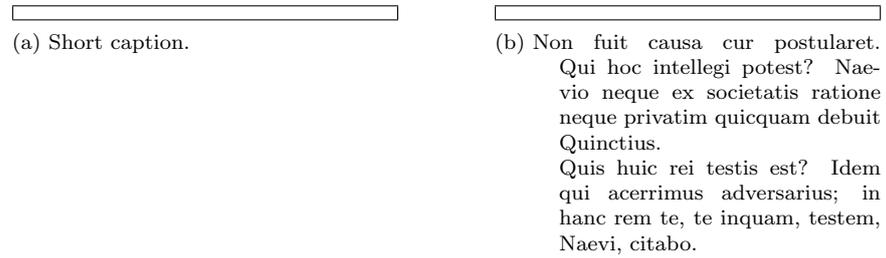Figure 27: Options `[format=hang,indentation=10pt,singlelinecheck=false]`.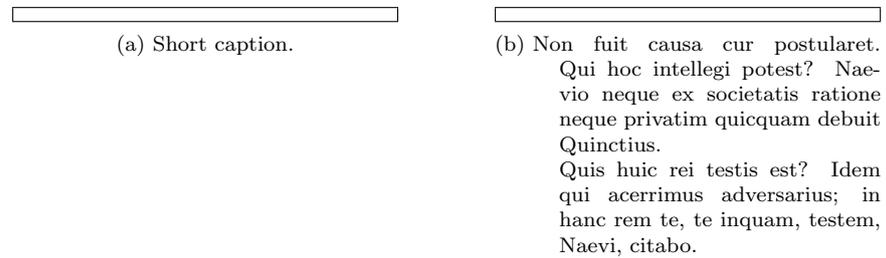Figure 28: Options `[format=hang,indentation=10pt]`.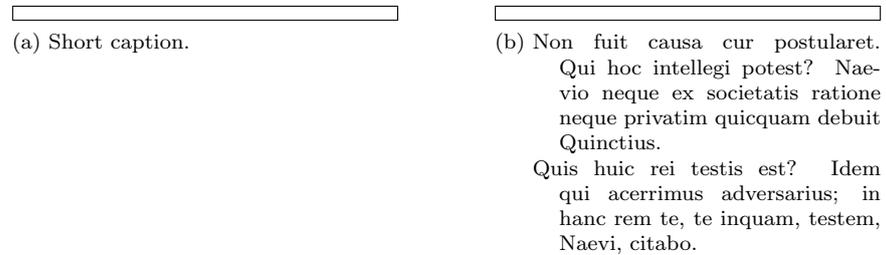Figure 29: Options `[format=hang,hangindent=10pt,singlelinecheck=false]`.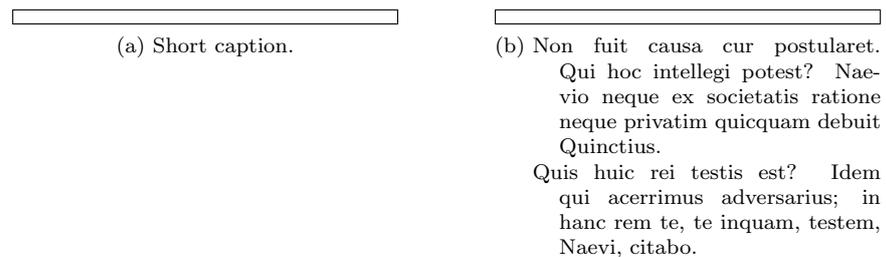Figure 30: Options `[format=hang,hangindent=10pt]`.

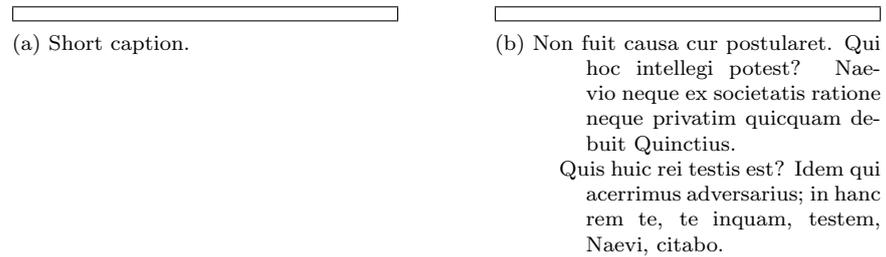

Figure 31: Options `[format=hang, hangindent=10pt, indention=10pt, singlelinecheck=false]`.

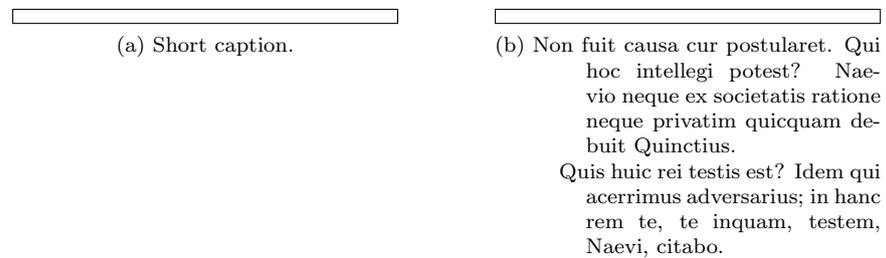

Figure 32: Options `[format=hang, hangindent=10pt, indention=10pt]`.

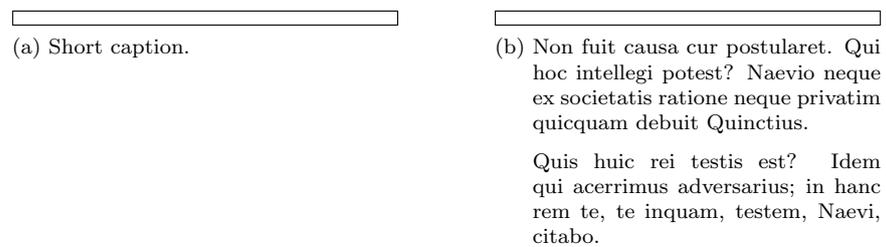

Figure 33: Options `[format=hang, parskip=5pt, singlelinecheck=false]`.

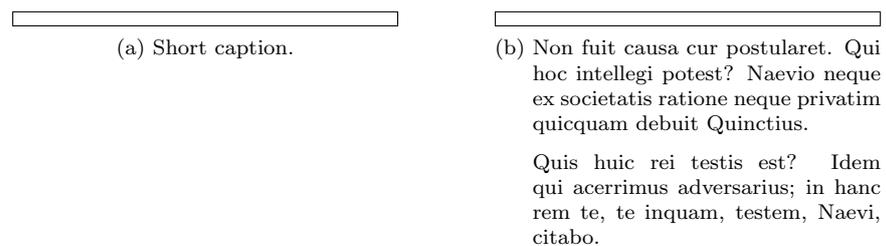

Figure 34: Options `[format=hang, parskip=5pt]`.

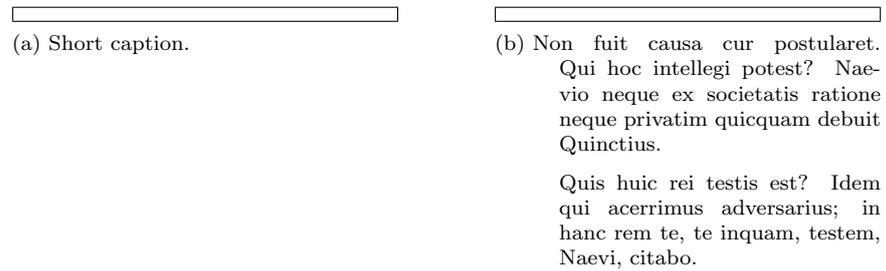

Figure 35: Options [format=hang, parskip=5pt, indention=10pt, singlelinecheck=false].

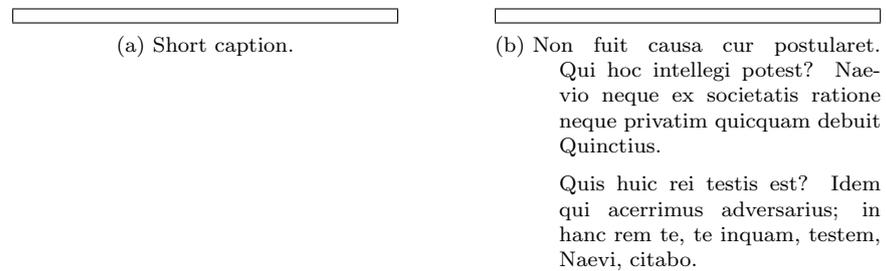

Figure 36: Options [format=hang, parskip=5pt, indention=10pt].

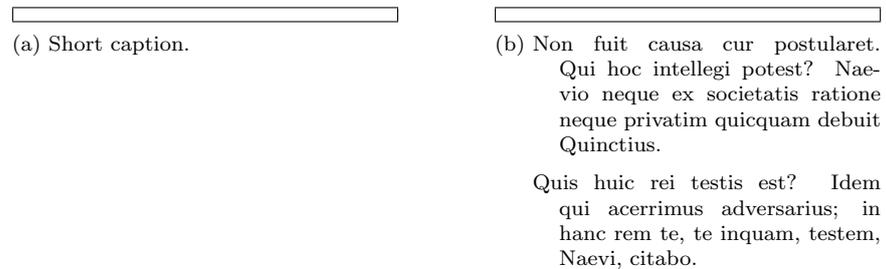

Figure 37: Options [format=hang, parskip=5pt, hangindent=10pt, singlelinecheck=false].

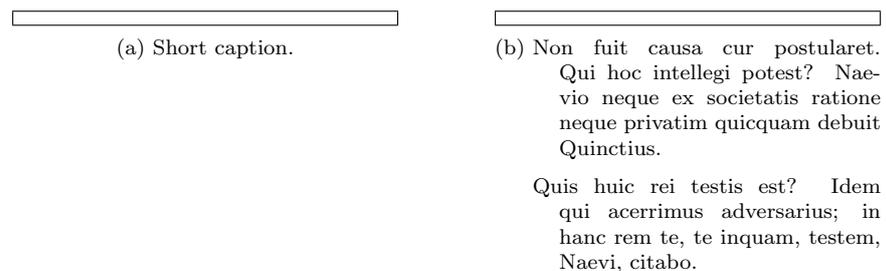

Figure 38: Options [format=hang, parskip=5pt, hangindent=10pt].

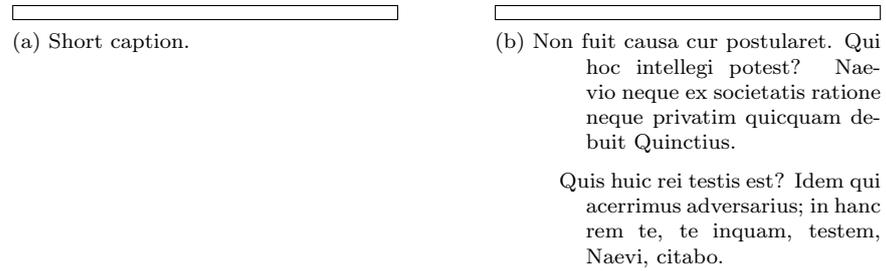

Figure 39: Options [format=hang, parskip=5pt, hangindent=10pt, indention=10pt, singlelinecheck=false].

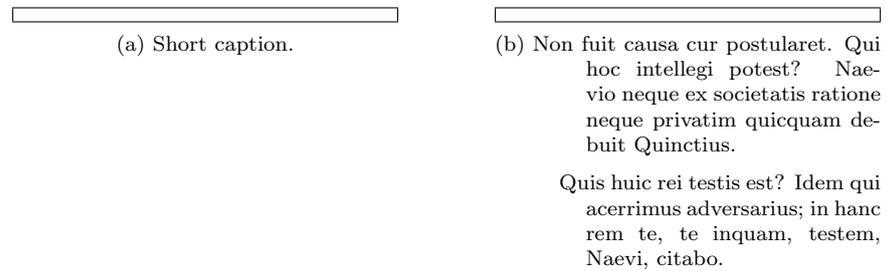

Figure 40: Options [format=hang, parskip=5pt, hangindent=10pt, indention=10pt].

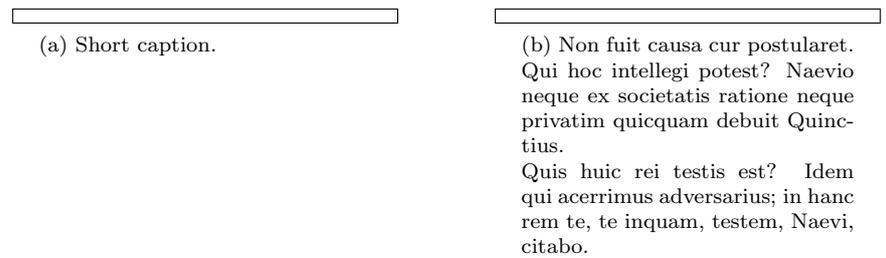

Figure 41: Options [margin=10pt, singlelinecheck=false].

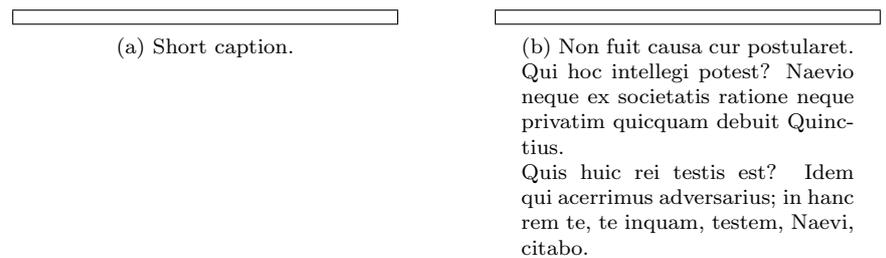

Figure 42: Options [margin=10pt].

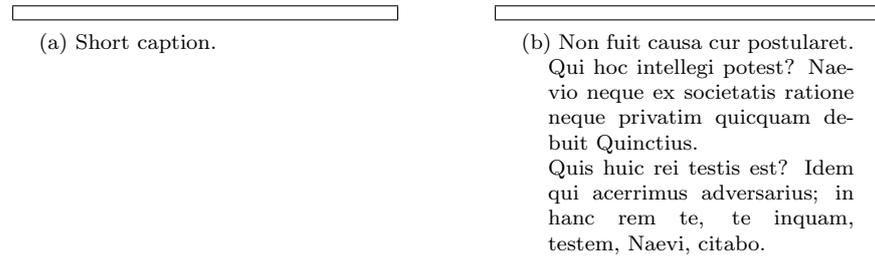

Figure 43: Options [margin=10pt,indentation=10pt,singlelinecheck=false].

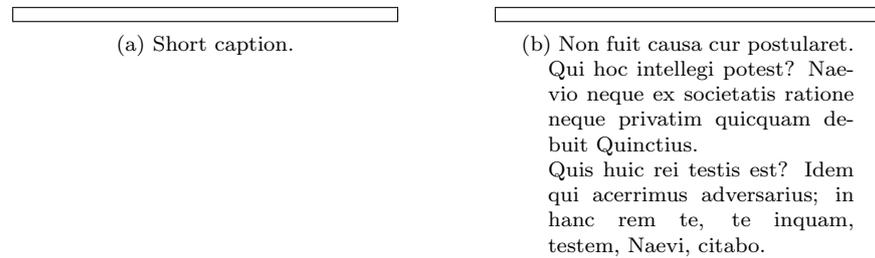

Figure 44: Options [margin=10pt,indentation=10pt].

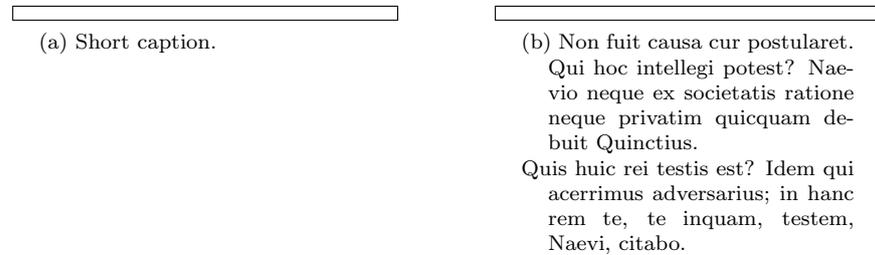

Figure 45: Options [margin=10pt,hangindent=10pt,singlelinecheck=false].

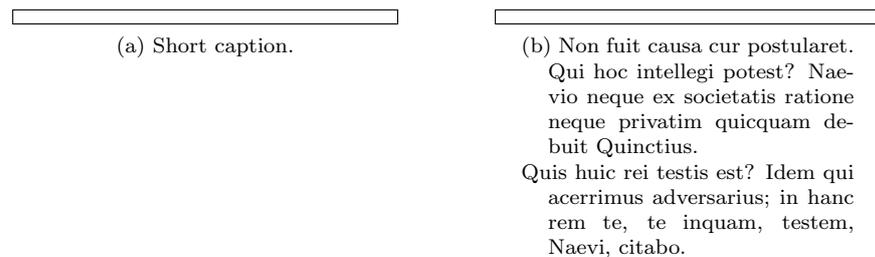

Figure 46: Options [margin=10pt,hangindent=10pt].

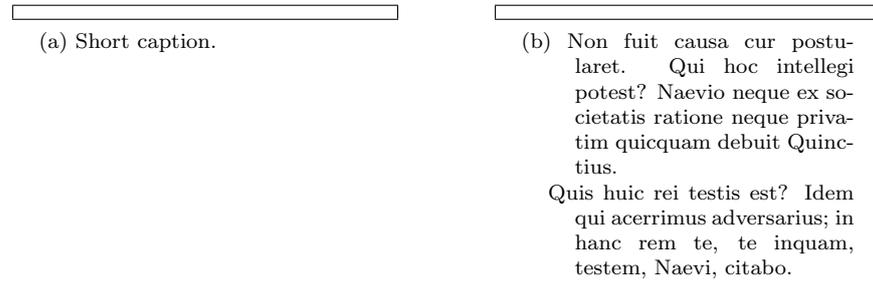

Figure 47: Options `[margin=10pt, hangindent=10pt, indention=10pt, singlelinecheck=false]`.

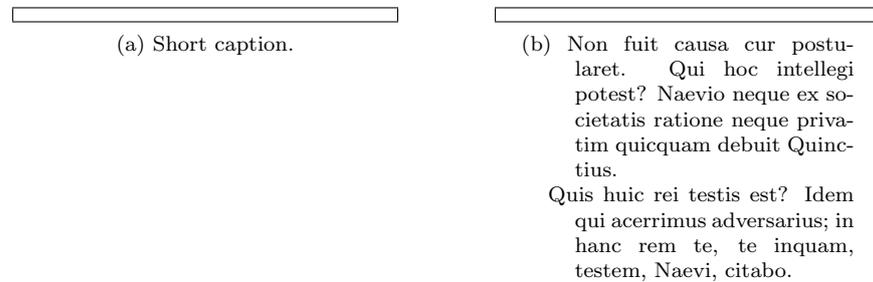

Figure 48: Options `[margin=10pt, hangindent=10pt, indention=10pt]`.

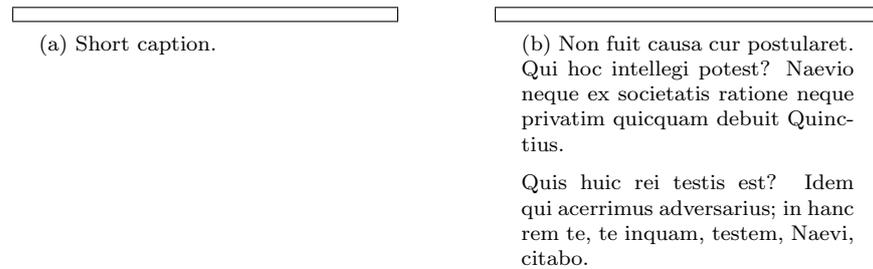

Figure 49: Options `[margin=10pt, parskip=5pt, singlelinecheck=false]`.

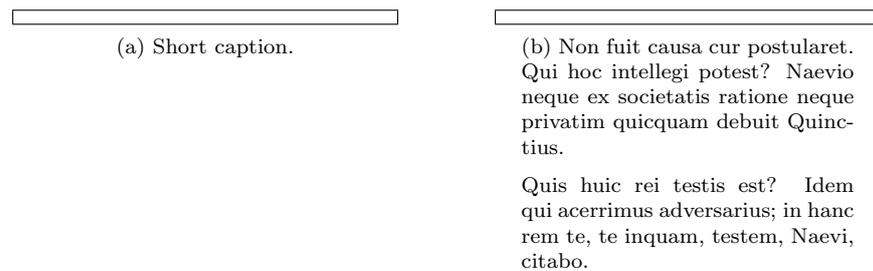

Figure 50: Options `[margin=10pt, parskip=5pt]`.

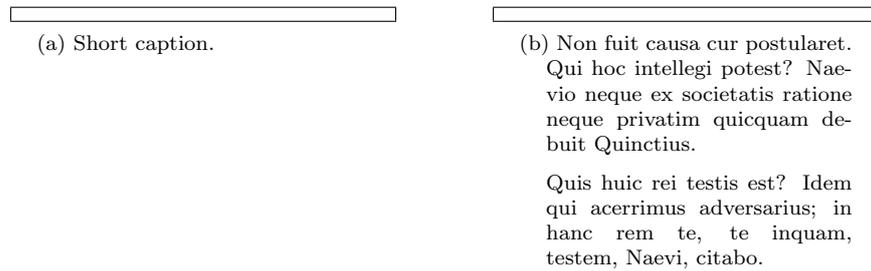

Figure 51: Options [margin=10pt,parskip=5pt,indentation=10pt, singlelinecheck=false].

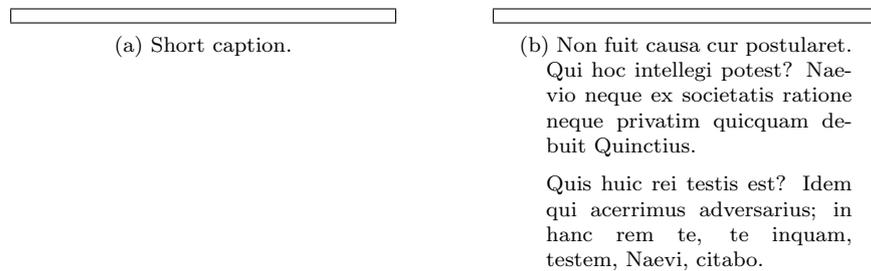

Figure 52: Options [margin=10pt,parskip=5pt,indentation=10pt].

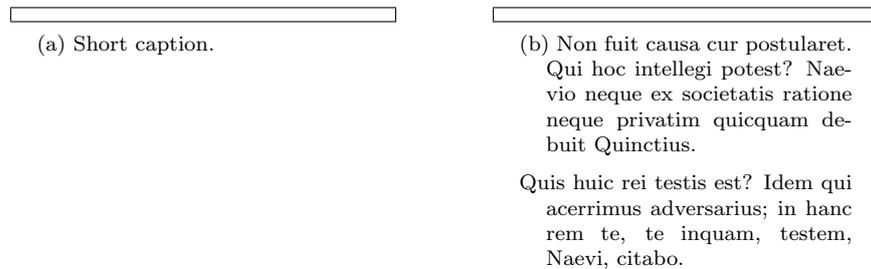

Figure 53: Options [margin=10pt,parskip=5pt,hangindent=10pt, singlelinecheck=false].

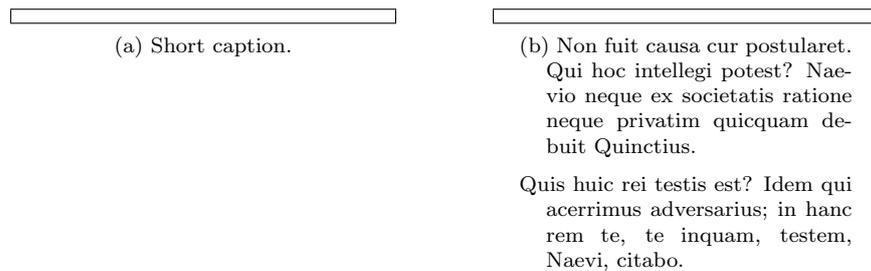

Figure 54: Options [margin=10pt,parskip=5pt,hangindent=10pt].

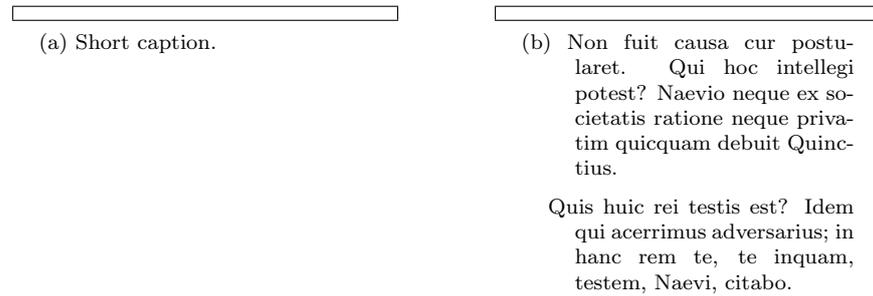

Figure 55: Options `[margin=10pt,parskip=5pt,hangindent=10pt,indentation=10pt,singlelinecheck=false]`.

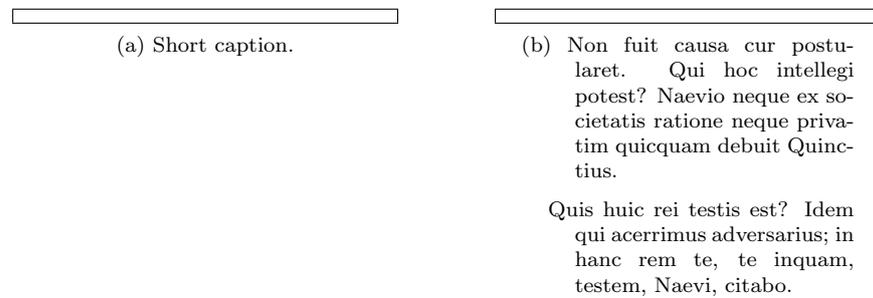

Figure 56: Options `[margin=10pt,parskip=5pt,hangindent=10pt,indentation=10pt]`.

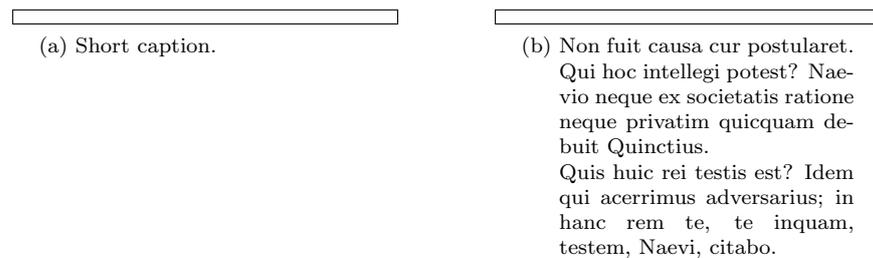

Figure 57: Options `[margin=10pt,format=hang,singlelinecheck=false]`.

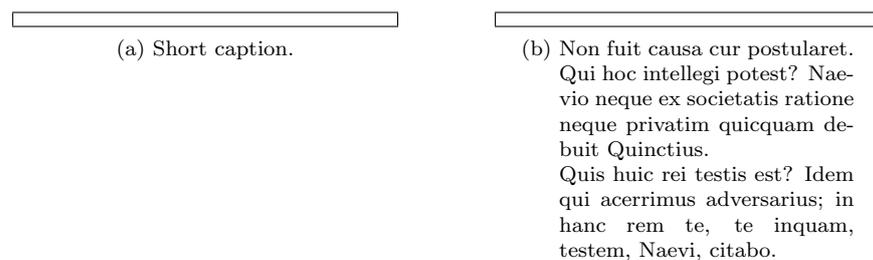

Figure 58: Options `[margin=10pt,format=hang]`.

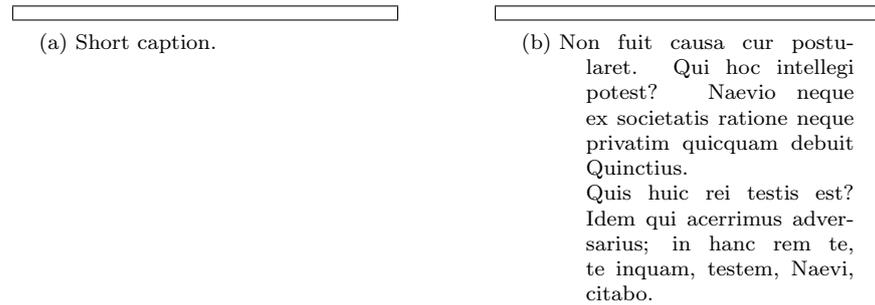

Figure 59: Options `[margin=10pt,format=hang,indention=10pt,singlelinecheck=false]`.

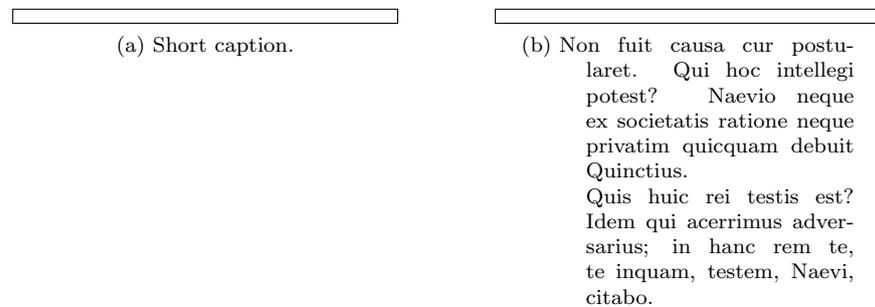

Figure 60: Options `[margin=10pt,format=hang,indention=10pt]`.

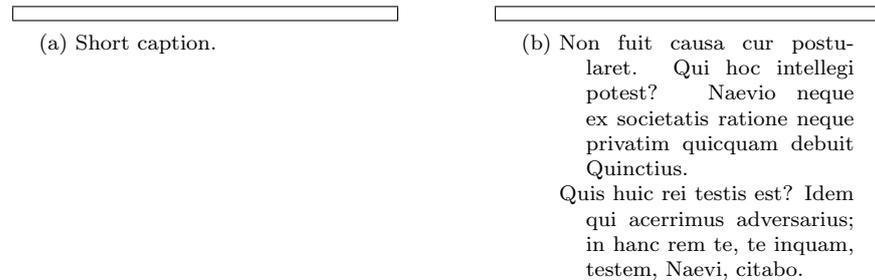

Figure 61: Options `[margin=10pt,format=hang,hangindent=10pt,singlelinecheck=false]`.

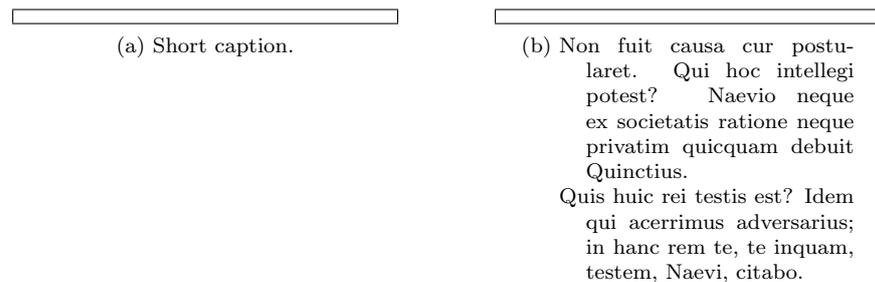

Figure 62: Options `[margin=10pt,format=hang,hangindent=10pt]`.

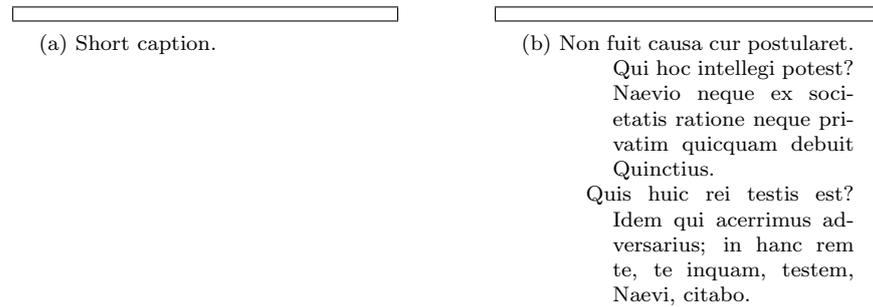

Figure 63: Options `[margin=10pt,format=hang,hangindent=10pt,indentation=10pt,singlelinecheck=false]`.

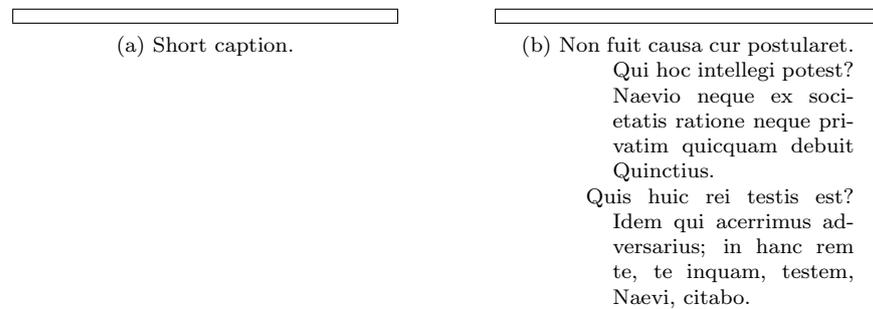

Figure 64: Options `[margin=10pt,format=hang,hangindent=10pt,indentation=10pt]`.

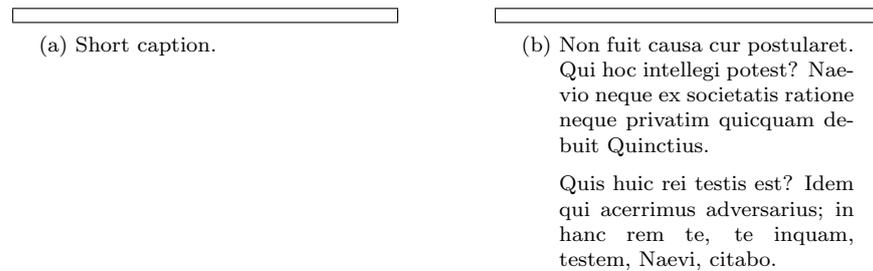

Figure 65: Options `[margin=10pt,format=hang,parskip=5pt,singlelinecheck=false]`.

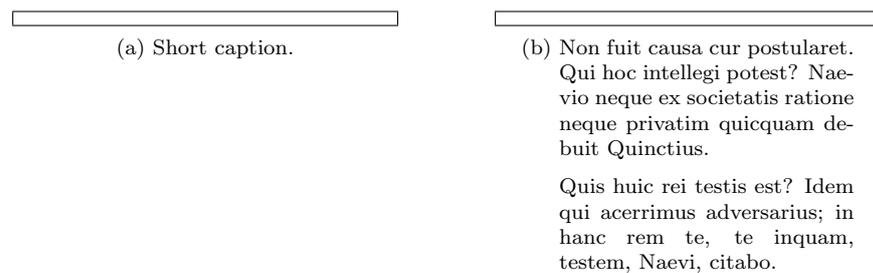

Figure 66: Options `[margin=10pt,format=hang,parskip=5pt]`.

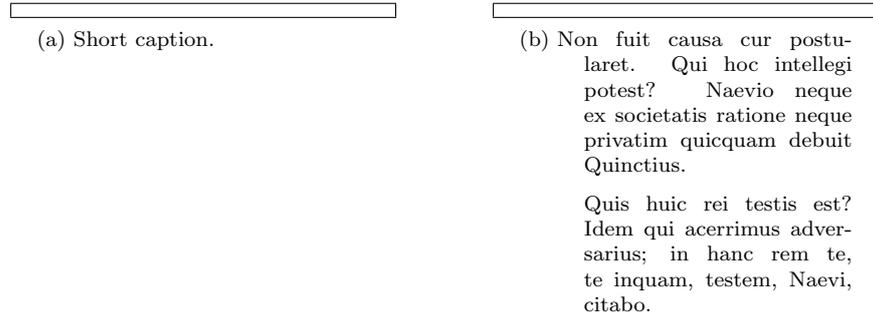

Figure 67: Options [margin=10pt,format=hang,parskip=5pt,indentation=10pt,singlelinecheck=false].

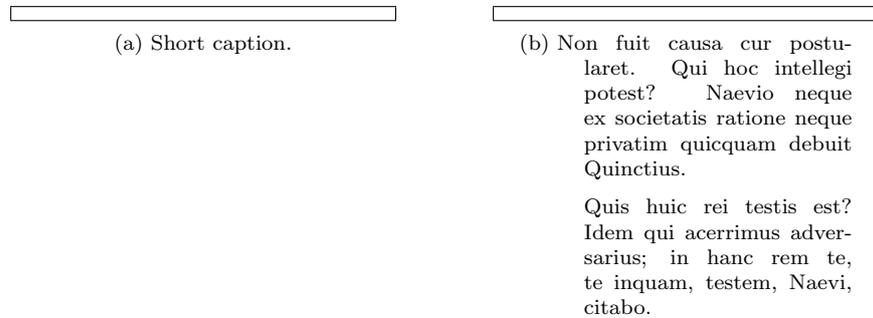

Figure 68: Options [margin=10pt,format=hang,parskip=5pt,indentation=10pt].

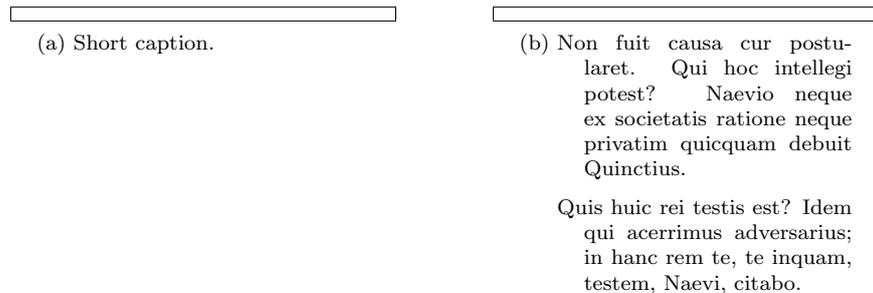

Figure 69: Options [margin=10pt,format=hang,parskip=5pt,hangindent=10pt,singlelinecheck=false].

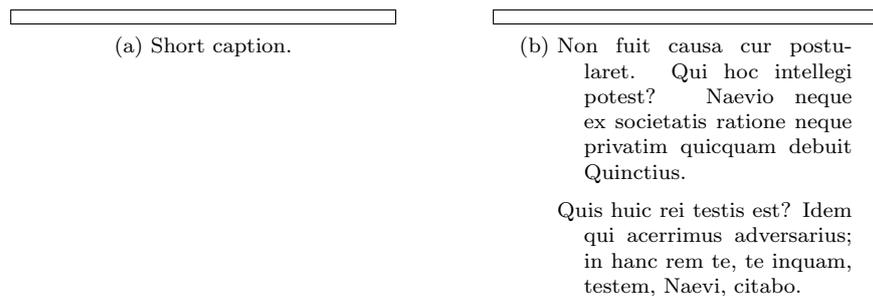

Figure 70: Options [margin=10pt,format=hang,parskip=5pt,hangindent=10pt].

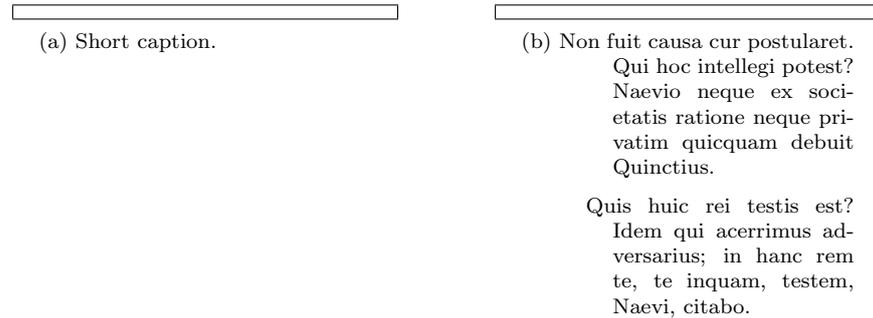

Figure 71: Options `[margin=10pt,format=hang,parskip=5pt,hangindent=10pt,indentation=10pt,singlelinecheck=false]`.

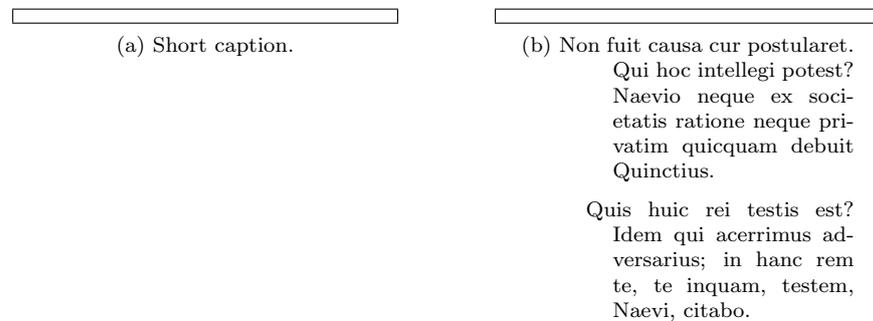

Figure 72: Options `[margin=10pt,format=hang,parskip=5pt,hangindent=10pt,indentation=10pt]`.

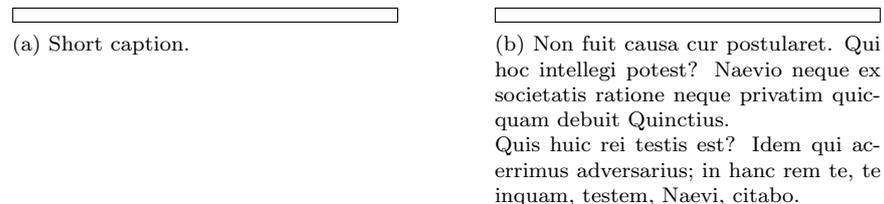

Figure 73: Options `[justification=justified,singlelinecheck=false]`.

### 3.1.3 The Caption Justification Options

There are nine options for setting the sub-caption format. The first is ‘justified’ which produces the format shown in figure 73. Only one of these options is allowed at a time. If multiple options appear, then only the last is used. The figures 74 thru 81 show the rest of these formats. The shape options selected along with each format option is the default (see figure 10), this shows the effect of the justification option on a single line caption.

#### 3.1.4 The Caption Label Options

There are three options for setting the sub-caption ‘labelformat’ as shown in figures 82–84. This is the label number and not any following punctuation or separator space (see below for setting these). The three cases are:

- ‘empty’: Without any label.

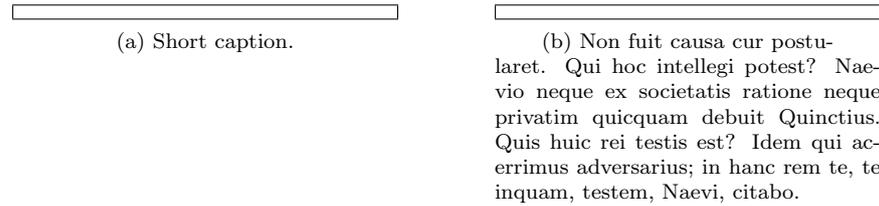

Figure 74: Options [justification=centerfirst, singlelinecheck=false].

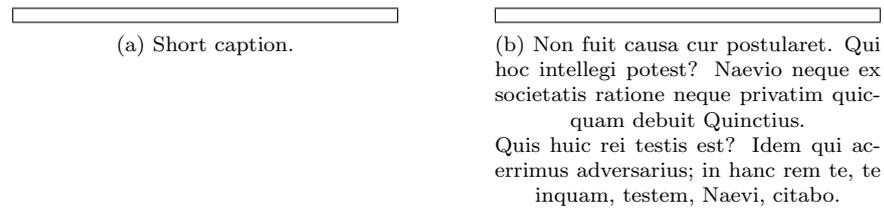

Figure 75: Options [justification=centerlast, singlelinecheck=false].

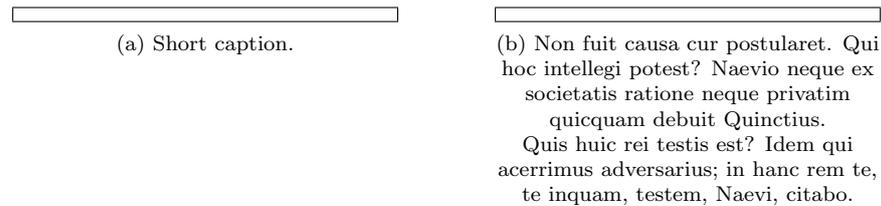

Figure 76: Options [justification=centering, singlelinecheck=false].

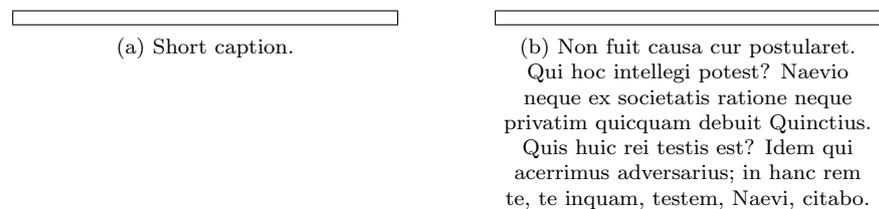

Figure 77: Options [justification=Centering, singlelinecheck=false].

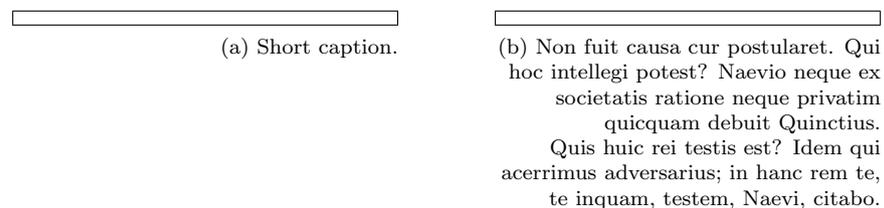

Figure 78: Options [justification=raggedleft, singlelinecheck=false].

- ‘simple’: Just the label number.
- ‘parens’: The label number surrounded by ‘()’.

The latter option, ‘parens’, is the default for sub-floats.

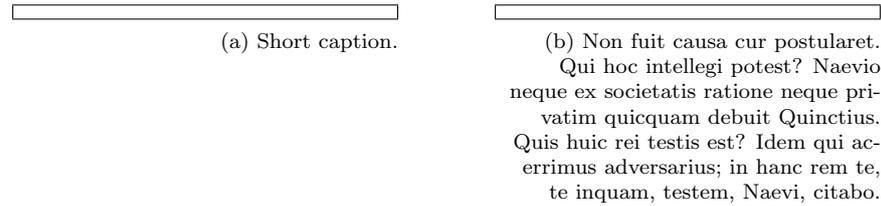Figure 79: Options `[justification=RaggedLeft, singlelinecheck=false]`.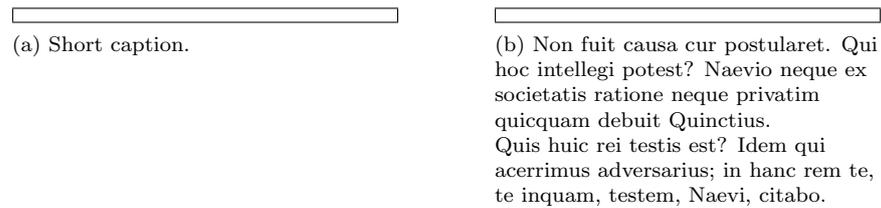Figure 80: Options `[justification=RaggedRight, singlelinecheck=false]`.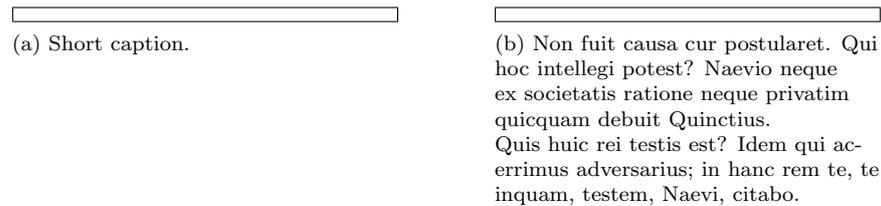Figure 81: Options `[justification=RaggedRight, singlelinecheck=false]`.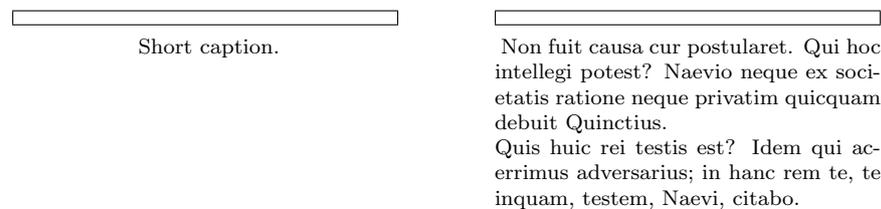Figure 82: Options `[labelformat=empty]`.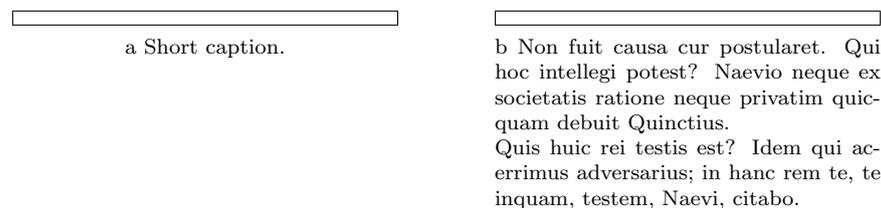Figure 83: Options `[labelformat=simple]`.

Figures 85–90 show the options for setting the punctuation and separator space following the figure number. These options are set with the ‘labelseparator’ keyword.

The label separator options are:

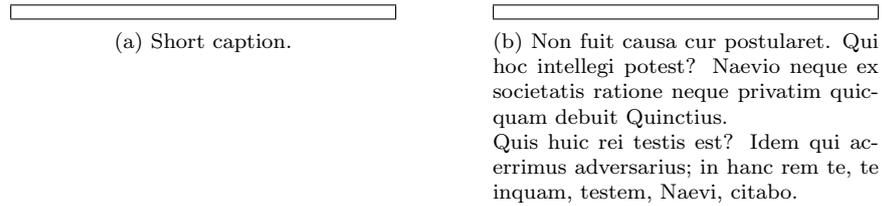

Figure 84: Options [labelformat=parens].

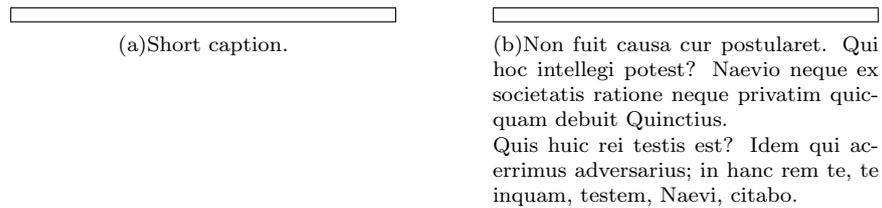

Figure 85: Options [labelsep=none].

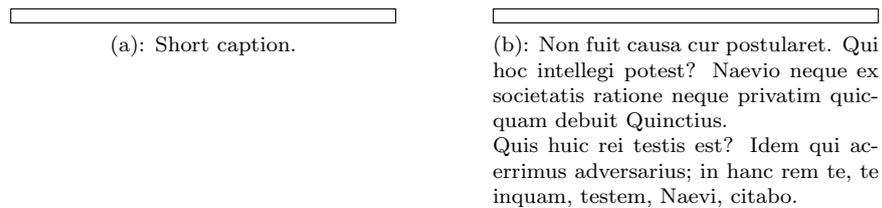

Figure 86: Options [labelsep=colon].

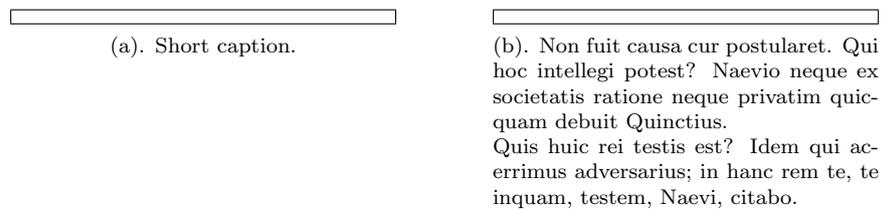

Figure 87: Options [labelsep=period].

- ‘none’ Nothing is added after the label.
- ‘colon’ A colon followed by a `\space` is added following the label.
- ‘period’ A period followed by a `\space` is added following the label.
- ‘space’ Just a `\space` is added following the label.
- ‘quad’ A `\quad` space is added following the label.
- ‘newline’ A new line is inserted after the label.

### 3.1.5 The Caption Position Option

The `caption` package ‘position’ option specifies whether the caption appears before or after the figure or table. This can adjust the relative spacing used to separate the float from the surrounding text. However, for the `subfig` package, it serves a more important function. That is it determines if the sub-floats belong to or are associated with the

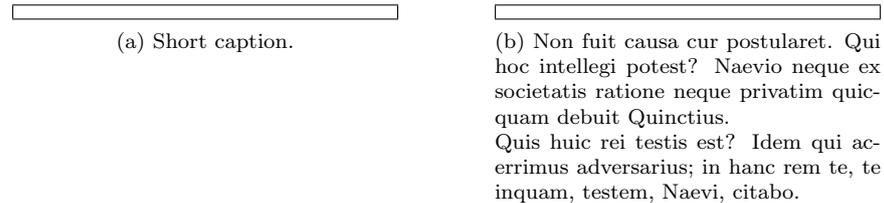Figure 88: Options [`labelsep=space`].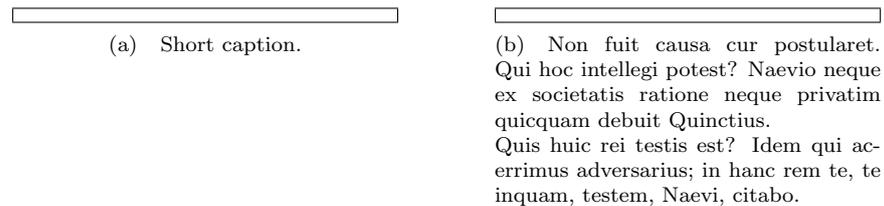Figure 89: Options [`labelsep=quad`].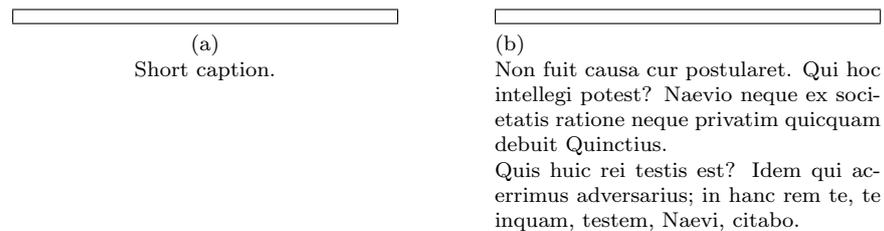Figure 90: Options [`labelsep=newline`].

last `\caption` command to be given, or the next one to be executed sometime in the future. If you find that your sub-references do not agree with the top-level labels, then you may need to specifically set the ‘`position`’. This is best done when loading the `caption` package, but may be done at anytime with the `\captionsetup` command.

## 3.2 Options from the Subfig Package

In addition to the options provided by the `caption` package, the `subfig` package provides the options shown in table 5.

### 3.2.1 The Subfig Configuration Specification

The default settings and layout of the `subfig` package can be modified by loading one or more configuration files. The `subfig` ‘`config`’ option loads the configuration file(s) after the package is setup, but before the “subfigure” or “subtable” sub-floats have been created (with the `\newsubfloat` command) and before the package options have been processed. See section 4.7 for an example of using the `subfigold.cfg` file to emulate the `subfigure` package.

Without a value, the ‘`config`’ keyword loads the file `subfig.cfg`. Use the value to load another file, for instance, ‘`config=altsf.cfg`’. If more than one configuration file is specified in the package options, then they are loaded in the order in which they appear in the option list. When used outside the package option list, the ‘`config`’ keyword is processed by the `caption` package and loads `caption.cfg` by default.

Table 5: Subfig specific options.

| KeyWord                    | Value       | Notes                                                       |
|----------------------------|-------------|-------------------------------------------------------------|
| 'config'                   | <filename>  | The default value is "subfig.cfg"                           |
| '<ext>depth' <sup>11</sup> | <number>    | The default value is 2.                                     |
| 'listofformat'             | 'empty'     | Label format: (none)                                        |
|                            | 'simple'    | Label format: ##                                            |
|                            | 'parens'    | Label format: #(#)                                          |
|                            | 'subsimple' | Label format: #                                             |
|                            | 'subparens' | Label format: (#)                                           |
| 'listofindent'             | <length>    | Entry indentation on List-of-Floats page.                   |
| 'listofnumwidth'           | <length>    | Space allocated for entry label.                            |
| 'farskip'                  | <glue>      | Glue placed opposite the sub-float caption.                 |
| 'captionskip'              | <glue>      | Glue placed between the sub-float and the caption.          |
| 'topadjust'                | <glue>      | Extra glue added to 'captionskip' when above the sub-float. |
| 'nearskip'                 | <glue>      | Glue placed opposite the caption from the sub-float.        |

**Note:** The package pre-defines the following values by adding them to the "subfloat" variable list with the `\captionsetup` command before loading the configuration file(s):

```
\captionsetup[subfloat]{%
  font=footnotesize,
  labelformat=parens,labelsep=space,
  listofformat=subparens}
```

### 3.2.2 The Subfig List-of-Floats Specification

The next two options, 'lofdepth' and 'lotdepth', are created along with the internal subfigure and subtable sub-floats. If other sub-floats are created, than the associated depth counter and keyword is created for them if it does not already exist. In order for the sub-captions to be shown in the List-of-Floats page, the related depth counter must be set to 2 or greater. These keywords allow the counters to be easily set in the option list or with the `\captionsetup` command.<sup>12</sup> The default value is 1, which turns off the printing of the sub-captions.

The next three options, 'listofformat', 'listofindent', and 'listofnumwidth', control and adjust the way that the sub-float number is displayed on the respective List-of-Floats page. The 'listofformat' shows how or if the sub-float number is shown. Where there are two '#' signs in the List-of-Page label formats, the first one stands for the `\p@<sub-float_type>` value and the second for the `\the<sub-float_type>` value. Where there is only one '#' it stands for the latter.

The 'listofindent' keyword sets the total indentation from the left margin, while the 'listofnumwidth' keyword controls the width of box for the label number. This is also the amount of extra indentation added to second and later lines of a multiple line entry.

### 3.2.3 The Subfig Layout

The layout of the sub-float contains several internal values which may be changed to customize appearance of the object. The following illustration shows the relationship of these values. Figure 91(a) shows the standard layout with the caption following the

<sup>11</sup>Where '<ext>depth' is initially only 'lofdepth' and 'lotdepth'. More such keywords may be added by the `\newsfloat` command (see section 2.1.2).

<sup>12</sup>The sub-caption depth counters must be set at the "global" level (see section 2.2.5) and before the corresponding `\listof...` command is used.

figure. The figure is vertically centered with some vertical space added above. If this is a float at the top of the page, than the space is suppressed. If the caption of the float follows the subfigures, than ‘farskip’ indicates the amount of space to skip. Otherwise, if the float caption precedes the subfigures, than ‘nearskip’ indicates the value to use. The best way to think of these two skips is that the ‘nearskip’ is closer to the main float caption than the ‘farskip’. After the subfigure, more vertical space, ‘captionskip’, is added between the subfigure and the sub-caption. Finally, ‘nearskip’ (or ‘farskip’) of vertical space added below. The baseline is located at the bottom of the figure. It is along this baseline that adjacent subfigure boxes are aligned.

Figure 91(c) shows the reversed case where the sub-caption precedes the figure (*i.e.*, ‘position=top’). In this case the ‘farskip’ and ‘nearskip’ are placed according to the position of the float caption as above and the ‘captionskip’ is increased by ‘topadjust’. The other two cases, figures 91(b) and (d)), show the cases where there is no caption. Note that the ‘captionskip’ (and ‘topadjust’ is left out when there is no caption. Again, note also, for all of these cases, that the space at the top of the subfigure is automatically removed for items that are the first box in a vertical list or other than the first box in a horizontal list. This allows tighter packing of the sub-floats and the full use of the page or `minipage`.

Each of these values, ‘farskip’, ‘captionskip’, ‘topadjust’, and ‘nearskip’<sup>13</sup>, may be changed from their defaults (see table 3) to adjust the subfigure for the current layout style. In addition, they may all assume negative values, which in some cases may solve problems with the layout, but is not recommended, in general.

### 3.2.4 The Subfig Package Startup

The startup sequence for the `subfig` package is to first load the `caption` package (with no options) if it has not already been loaded. Next it sets the following default values on the “subfloat” variable:

```
\captionsetup[subfloat]{font=footnotesize,
                        labelformat=parens,labelsep=space,
                        listofformat=subparens}
```

This overrides the `caption` package default in which the font is undefined and uses that of the surrounding document<sup>14</sup>; the label is ‘simple’ and followed by a ‘colon’ and space. It also defines the ‘listofformat’ at this level in the case that it is added to the `caption` package. Note that if the default settings to the “subfloat” list are not desired, they may be removed with a `\clearcaptionsetup` command (see section 3.2.1). Also the current settings may be checked using the following (here for a subfigure):

```
\showcaptionsetup{figure}
\showcaptionsetup{subfloat}
\showcaptionsetup{subfigure}
```

placed just before the `\subfloat` will show in the log what overrides are being applied at that point.

Second, any configuration files are loaded. If there are more than one listed in the `\usepackage` options list, than they are loaded in the order specified in the list.

<sup>13</sup>Also the ‘margin’ and ‘width’ keywords affect the `subfig` layout, see section 3.1.2

<sup>14</sup>If, in fact, ‘font’ is defined in the `caption` options list before loading the `subfig` package; than the above redefinition on the “subfloat” variable will hide that setting from all of the sub-floats. If you want them to have the same overall font setting (let’s say “bf,sl”), than you will need to add one of the following sets of commands:

```
\captionsetup[subfloat]{font={footnotesize,bf,sl}}
```

or

```
\captionsetup{labelfont={bf,sl},textfont={bf,sl}}
```

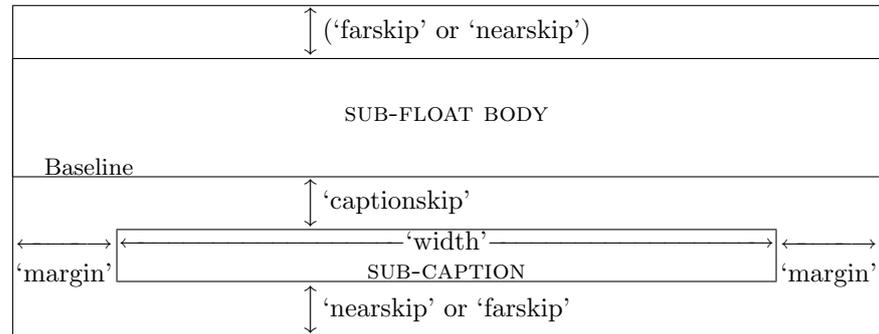

(a) Standard layout (Sub-float: position=bottom).

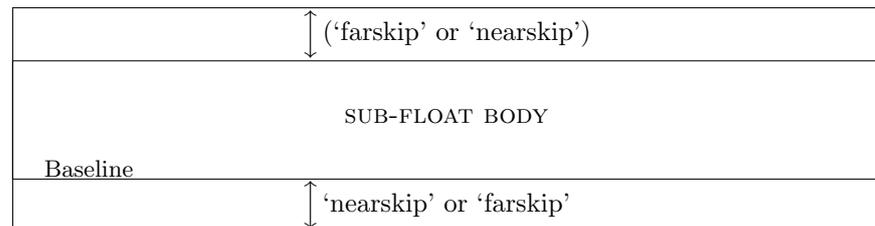

(b) Standard layout without a caption (Sub-float: position=bottom)

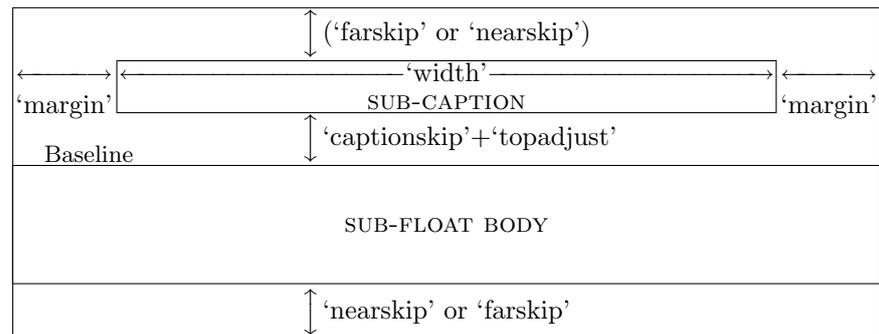

(c) Reversed layout (Sub-float: position=top).

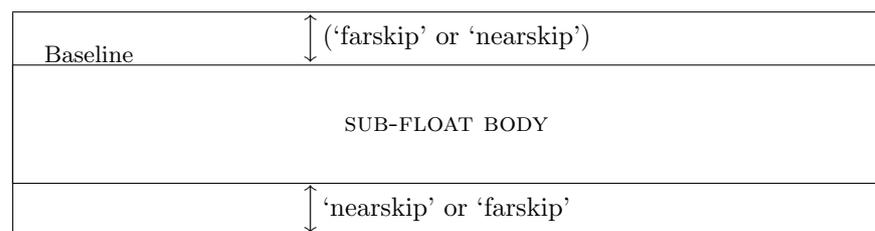

(d) Standard layout without a caption (Sub-float: position=top)

Figure 91: Sub-float Layout. If the respective float caption position is 'bottom', then the 'farskip' is used at the top and the 'narskip' is used at the bottom. If the respective float caption position is 'top', then these skips are reversed. Also, the top skip is suppressed at the top of a page.

Next, the other (non-'config') options in the `\usepackage` options list are added to the "subfloat" list.

Finally, the `subfig` package finishes defining its functions and if the configuration file(s) have not already defined the sub-floats: "subfigure" and "subtable", then they are defined.

## 4 Compatibility With Other Packages.

This section discusses specific aspects of compatibility with other packages with which the subfig package is often used.

### 4.1 Caption Package

The subfig package requires the caption package in order to format the sub-float captions. However, the ‘position’ keyword option may only take two values when used with the subfig package; those are, ‘top’ and ‘bottom’. Any other value will be treated as if ‘position=bottom’ was specified.

**Warning:** By default (without the subfig.cfg loaded), the ‘position’ values are expected to be defined prior to loading the subfig package or defined afterward. However they are defined, it is up to the user to insure that the captions are used correctly with the sub-captions, because using a caption, that is expected to precede the sub-captions, after the sub-captions (or *vice-versa*) will cause the List-of-Floats page and float label references to be incorrect.

For compatibility with other packages which modify the caption and where the standard caption package would interfere with the desired layout, the caption package has a special option, ‘caption=false’, which loads the internals (*i.e.*, the “kernel” caption3 package) without modifying the \caption command.

### 4.2 Float Package

To create a new sub-float, you first need a new floating environment. If you have that, great, otherwise, load the float package and create one with a series of commands similar to the following. Here we create a new map environment so that the subfig package will work with it. For this example we have indicated that we expect to place the main float caption before the sub-floats.

```
\usepackage{float}
\newfloat{map}{tbph}{lom}
\restylefloat*{map}
\floatstyle{plain}
\floatname{map}{Map}
\captionsetup[map]{position=top}
\newcommand{\listofmaps}{\listof{map}{List of Maps}}
```

Then you can then create the new sub-float with:

```
\newsfloat[position=top,listofformat=subsimple]{map}
```

Here we also indicate that we want the sub-caption to be placed above the submaps and that the reference label on the list-of-maps page will be in simple plain format without parentheses.

Now the \subfloat command will work in the map environment.

For example, the following code generates map 1:

```
\begin{map}%
  \centering
  \caption{This example shows two small maps.}%
  \label{map:example}%
  \subfloat[First map.]{...figure code...}%
  \qqquad
  \subfloat[Second map.]{...figure code...}%
\end{map}
```

Map 1: This example shows two small maps.

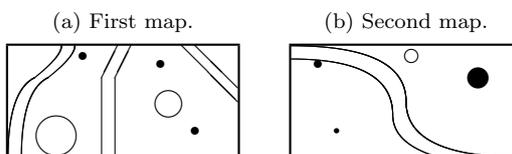

### 4.3 FloatRow Package

This package is compatible with the the `floatrow` package and contains hooks to allow it to work correctly with subfloats. In particular, the existence of the `\FBsc@max` command in the package turns on the hooks. See the code for the macros `\sf@@@subfloat` and `\sf@subcaption` for details.

The following code and table 6 show an example of using the `floatrow` package to align captions. Without it, the first caption, (a), would be located just above the first table rather than even with the first line of the second caption, (b).

```

:
\usepackage{booktabs}
\usepackage{subfig}
\captionsetup[table]{position=top}
\captionsetup[subtable]{position=top}
:
\usepackage[heightadjust=all,valign=t]{floatrow,fr-subfig}
\floatsetup{style=Plaintop}
:
\begin{table}%
\floatbox[table][\FBwidth]%
  {\caption{Results in Two Tables.}%
  \label{tab:floatrow}}{%
\begin{subfloatrow}
\subfloat[First Table of Results.]{\label{tab:floatrow:one}%
\begin{tabular}{lcc}
\begin{tabular}{lcc}
\multicolumn{1}{c}{\raisebox{-1.5ex}{\bf Result Type}} & \toprule
& \multicolumn{2}{c}{\bf Result Data} & \\\
& {\bf Set One} & {\bf Set Two} & \\\ \midrule
First type & 0.24 & 4.12 & \\\
Second type & 1.34 & 2.01 & \\\
Third type & 2.99 & 4.13 & \\\
Fourth type & 2.67 & 0.08 & \\\ \bottomrule
\end{tabular}}
\end{tabular}}
\subfloat[Second Table of Results.][Second Table of Results.
  However, this one has a very long caption that causes
  problems with alignment.]{\label{tab:floatrow:two}%
\begin{tabular}{lccc}
\begin{tabular}{lccc}
\multicolumn{1}{c}{\raisebox{-1.5ex}{\bf Result Type}} & \toprule
& \multicolumn{2}{c}{\bf Result Data} & \\\
& {\bf Set 1} & {\bf Set 2} & {\bf Set 3} & \\\ \midrule
First type & 4.20 & blue & 2.14 & \\\
Second type & 4.31 & red & 1.02 & \\\
Third type & 4.31 & green & 8.01 & \\\ \bottomrule
\end{tabular}}
\end{tabular}}
\end{subfloatrow}}% \end{table}

```

Table 6: Results in Two Tables.

(a) First Table of Results.

| Result Type | Result Data |         |
|-------------|-------------|---------|
|             | Set One     | Set Two |
| First type  | 0.24        | 4.12    |
| Second type | 1.34        | 2.01    |
| Third type  | 2.99        | 4.13    |
| Fourth type | 2.67        | 0.08    |

(b) Second Table of Results. However, this one has a very long caption that causes problems with alignment.

| Result Type | Result Data |       |       |
|-------------|-------------|-------|-------|
|             | Set 1       | Set 2 | Set 3 |
| First type  | 4.20        | blue  | 2.14  |
| Second type | 4.31        | red   | 1.02  |
| Third type  | 4.31        | green | 8.01  |

#### 4.4 verbatim and fancyvrb packages

You cannot place a `verbatim` environment inside of the `\subfloat` command because the `verbatim` environment needs to change the character classes before the text in the environment is read by  $\TeX$ . Therefore, if you really want to include verbatim text inside a sub-float, you will need to place the verbatim text into a box and then feed the box to the `\subfloat` command.

One way to do this is by defining and using a `SubFloat` environment, as shown in figure92. Such as placing the following in the preamble of your paper:

```

\makeatletter
\newbox\sf@box
\newenvironment{SubFloat}[2][ ]%
  {\def\sf@one{#1}%
   \def\sf@two{#2}%
   \setbox\sf@box\hbox
    \bgroup}%
  { \egroup
   \ifx\@empty\sf@two\@empty\relax
     \def\sf@two{\@empty}
   \fi
   \ifx\@empty\sf@one\@empty\relax
     \subfloat[\sf@two]{\box\sf@box}%
   \else
     \subfloat[\sf@one][\sf@two]{\box\sf@box}%
   \fi}
\makeatother

```

and then using it in your code as shown below. While this does not exactly produce the options shown in table 2, it is close enough for regular use and may be adjusted if necessary.

```

\begin{figure}
  \centering
  \begin{SubFloat}[Black box]{\label{fig:label1}Caption 1.}%
    \rule{4cm}{3cm}%...blackbox subfigure...
  \end{SubFloat}%
  \hspace{1.5cm}%
  \begin{SubFloat}{\label{fig:label2}Caption 2.}%...verbatim subfigure with
    \begin{minipage}[b]{0.3\linewidth}% a minipage to control the width...
      \begin{verbatim}

```

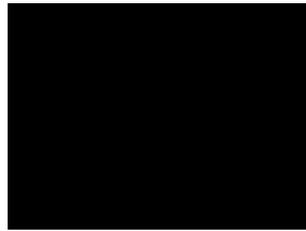

(a) Caption 1.

```
abc def ghi jkl
  xx  x  xxx
abc def ghi jkl
```

(b) Caption 2.

Figure 92: Main Caption.

```
abc def ghi jkl
  xx  x  xxx
abc def ghi jkl
  \end{verbatim}%
  \end{minipage}%
  \end{SubFloat}
  \caption{Main Caption.}
  \label{fig:label}
\end{figure}
```

#### 4.5 IEEEtrans Class

The `IEEEtrans` Class defines its own caption layout. Therefore to use the `subfig` package, you need to “turn off” the `caption` package. The following two setups are the same:

```
\usepackage[caption=false]{caption}
\usepackage[...]{subfig}
```

or

```
\usepackage[caption=false, ...]{subfig}
```

#### 4.6 Other Packages

The `subfig` package has been tested with the following packages and is known to work correctly.<sup>15</sup>

- `fixltx2e`
- `captcont`
- `hyperref`
- `hypcap`

Further, the following packages are known not to work with, or that have some problems when used with the `subfig` package:

- `ccaption`
- `hvfloat`
- `nonfloat`

<sup>15</sup>If you find any problem with these or any other package, please create a small example demonstrating the problem and send it to the author.

## 4.7 Backward Compatibility with the Subfigure Package

The following code sets up a configuration file to make the `subfig` package be nearly compatible with the older `subfigure` package. The first major difference is that the spacing is not quite the same due to internal changes in the sub-float setup and that some of the old tweaks that involved changing internal variables often will no longer work.

The other major change is that the old ‘topskip’ and ‘bottomskip’ no longer exist and their replacements ‘farskip’ and ‘narskip’ act differently. The new skips also surround the sub-caption and sub-float body, but where the ‘bottomskip’ was always next to the sub-caption, the new ‘narskip’ is always nearer the main (float) caption. The other two vary in the same way. Normally, this difference is minor and can be ignored, but in some cases you will need to adjust them to get your desired *look and feel*.

`\subfigure` The first section creates the `\subfigure` and the `\subtable` commands.

```
\subtable
1 \ifundefined{c@subfigure}{\newsfloat{figure}}{}
2 \def\subfigure{\subfloat}

3 \ifundefined{c@subtable}{\newsfloat{table}}{}
4 \def\subtable{\subfloat}
```

Next we restore the caption value-keywords for the option list. Currently these are available within the main document with the `\captionsetup` command. However, this may change in a later release of the `subfig` package.

```
5 \DeclareCaptionOption{normal}[]{\caption@setformat{default}}
6 \DeclareCaptionOption{isu}[]{\caption@setformat{format=hang}}
7 \DeclareCaptionOption{format=hang}[]{\caption@setformat{format=hang}}
8 \DeclareCaptionOption{center}[]{\caption@setjustification{centering}}
9 \DeclareCaptionOption{anne}[]{\caption@setjustification{centerlast}}
10 \DeclareCaptionOption{centerlast}[]{\caption@setjustification{centerlast}}
11 \DeclareCaptionOption{nooneline}[]{\sf@setbool{slc}{0}}
12 \DeclareCaptionOption{scriptsize}[]{\def\captionfont{\scriptsize}}
13 \DeclareCaptionOption{footnotesize}[]{\def\captionfont{\footnotesize}}
14 \DeclareCaptionOption{small}[]{\def\captionfont{\small}}
15 \DeclareCaptionOption{normalsize}[]{\def\captionfont{\normalsize}}
16 \DeclareCaptionOption{large}[]{\def\captionfont{\large}}
17 \DeclareCaptionOption{Large}[]{\def\captionfont{\Large}}
18 \DeclareCaptionOption{up}[]{\l@addto@macro\captionlabelfont\upshape}
19 \DeclareCaptionOption{it}[]{\l@addto@macro\captionlabelfont\itshape}
20 \DeclareCaptionOption{sl}[]{\l@addto@macro\captionlabelfont\slshape}
21 \DeclareCaptionOption{sc}[]{\l@addto@macro\captionlabelfont\scshape}
22 \DeclareCaptionOption{md}[]{\l@addto@macro\captionlabelfont\mdseries}
23 \DeclareCaptionOption{bf}[]{\l@addto@macro\captionlabelfont\bfseries}
24 \DeclareCaptionOption{rm}[]{\l@addto@macro\captionlabelfont\rmfamily}
25 \DeclareCaptionOption{sf}[]{\l@addto@macro\captionlabelfont\sffamily}
26 \DeclareCaptionOption{tt}[]{\l@addto@macro\captionlabelfont\ttfamily}
27 \DeclareCaptionOption{ruled}[1]{\sf@setbool{ruled}{#1}}
28 \DeclareCaptionOption{singlelinecheck}[true]{\sf@setbool{slc}{#1}}
29 \DeclareCaptionOption{oneline}[1]{\sf@setbool{slc}{#1}}
30 \DeclareCaptionOption{justified}[]{\caption@setjustification{justified}}
31 \DeclareCaptionOption{centering}[]{\caption@setjustification{centering}}
32 \DeclareCaptionOption{centerfirst}[]{\caption@setjustification{centerfirst}}
33 \DeclareCaptionOption{flushright}[]{\caption@setjustification{centerleft}}
34 \DeclareCaptionOption{raggedleft}[]{\caption@setjustification{raggedleft}}
35 \DeclareCaptionOption{raggedright}[]{\caption@setjustification{raggedright}}
36 \DeclareCaptionOption{RaggedRight}[]{\caption@setjustification{RaggedRight}}
37 \DeclareCaptionOption{RaggedLeft}[]{\caption@setjustification{RaggedLeft}}
38 \DeclareCaptionOption{Centering}[]{\caption@setjustification{Centering}}
```

The second list of value-keywords allows the uppercase font options to set the font for the caption text.

```

39 \DeclareCaptionOption{UP} [] {\l@addto@macro\captiontextfont\upshape}
40 \DeclareCaptionOption{IT} [] {\l@addto@macro\captiontextfont\itshape}
41 \DeclareCaptionOption{SL} [] {\l@addto@macro\captiontextfont\slshape}
42 \DeclareCaptionOption{SC} [] {\l@addto@macro\captiontextfont\scshape}
43 \DeclareCaptionOption{MD} [] {\l@addto@macro\captiontextfont\mdseries}
44 \DeclareCaptionOption{BF} [] {\l@addto@macro\captiontextfont\bfseries}
45 \DeclareCaptionOption{RM} [] {\l@addto@macro\captiontextfont\rmfamily}
46 \DeclareCaptionOption{SF} [] {\l@addto@macro\captiontextfont\sffamily}
47 \DeclareCaptionOption{TT} [] {\l@addto@macro\captiontextfont\ttfamily}

```

Next, the subfigure “...topcap” and “...bottomcap” options are emulated using the new “position” option.

```

48 \DeclareCaptionOption{figbotcap} [] {\captionsetup[figure]{position=bottom}}
49 \DeclareCaptionOption{tabbotcap} [] {\captionsetup[table]{position=bottom}}
50 \DeclareCaptionOption{FIGBOTCAP} [] {\captionsetup[figure]{position=bottom}%
51     \captionsetup[subfigure]{position=bottom}}
52 \DeclareCaptionOption{TABBOTCAP} [] {\captionsetup[table]{position=bottom}%
53     \captionsetup[subtable]{position=bottom}}
54 \DeclareCaptionOption{figtopcap} [] {\captionsetup[figure]{position=top}}
55 \DeclareCaptionOption{tabtopcap} [] {\captionsetup[table]{position=top}}
56 \DeclareCaptionOption{FIGTOPCAP} [] {\captionsetup[figure]{position=top}%
57     \captionsetup[subfigure]{position=top}}
58 \DeclareCaptionOption{TABTOPCAP} [] {\captionsetup[table]{position=top}%
59     \captionsetup[subtable]{position=top}}

```

Then, the “loose” and “tight” options are approximately emulated.

```

60 \DeclareCaptionOption{loose} [] {%
61     \captionsetup{farskip=10pt,topadjust=0pt,captionskip=10pt,%
62         nearskip=10pt,margin=10pt}}
63 \DeclareCaptionOption{tight} [] {%
64     \captionsetup{farskip=5pt,topadjust=0pt,captionskip=3pt,%
65         nearskip=5pt,margin=0pt}}

```

We can now set the sub-float defaults beyond what is set in the subfig package. We only need to set the default to the ‘loose’ settings.

```
66 \captionsetup[subfloat]{loose}
```

Finally, we redefine the starred form of `\subref` to `\Subref`.

```
67 \def\Subref{\subref*}
```

## 5 Some Examples

The easiest way to show the use of this package is to give a few examples. The two most important things to remember when working with the `subfig` package are that (1) the sub-floats are aligned along their baselines (see figure 91 and (2) that whitespace in the floating environments are significant and affect the layout.

The baseline of the sub-float is usually at the bottom of the sub-float body or (when the sub-caption appears at the top) at the bottom of the sub-caption *and* the ‘caption-skip’ space—which is usually the same as the top of the sub-float. However sometimes, especially when using the `tabular`, `array`, or `minipage` environments to build the figure, the baseline appears elsewhere. The above three environments are all aligned at their center by default but that may be changed with the optional ‘[t]’ or ‘[b]’ arguments. As a last resort you can wrap all of your figures in a `\vtop` box with a `\vbox to 0pt{\null}` at the top followed by the sub-float body.

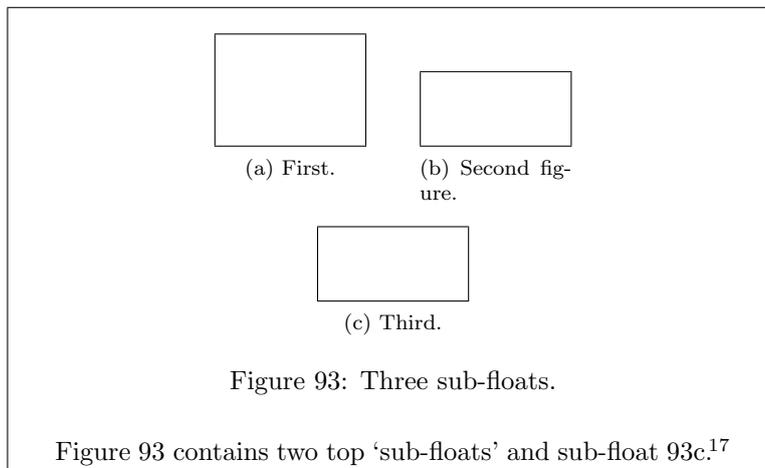

If your sub-float is not quite centered or where you want it to be, the problem is often a space character being placed to one side or the other of the sub-float body. Some general rules of thumb are:<sup>16</sup>

- Two end-of-lines following each other (ignoring any whitespace) are turned into a `\par` or paragraph break.
- Multiple whitespace (including the end-of-line) are compressed into a single space.
- The spaces after a macro command name (*e.g.*, `\foo`) are ignored.
- A `'%` character at the end of the line suppresses the end-of-line and all of the spaces (if any) at the beginning of the next line.

To suppress significant extra whitespace, you can add some `'%` characters at the end of each line that doesn't end with a command name. This is more than is required, but extra `'%` usually don't cause a problem.

## 5.1 A Simple Example

The first example, shown in figure 93, specifies `\centering` to horizontally center the set of sub-floats, and uses `\` and some horizontal space (using `\qqquad`) to control the placement of the sub-floats. Note that the alignment of the top two sub-floats is along the bottom of the body portion of each.

```

\begin{figure}%
  \centering
  \subfloat[First.]{...}\qqquad
  \subfloat[Second figure.]{...}\
  \subfloat[Third.]{\label{3figs-c}...}%
  \caption{Three sub-floats.}
  \label{3figs}
\end{figure}
:
Figure~\ref{3figs} contains two top 'sub-floats' and
sub-float~\ref{3figs-c}.

```

<sup>16</sup>See chapters 7 and 8 of “The TeXbook” [7] for details.

<sup>17</sup>In this and later boxed figures, the boxes are intended to represent a portion of the page in which the figure occurs. This is usually to show the figure along with some text or to show the effect of some option on multiple pages.

| <b>List of Figures</b> |                         |                    |
|------------------------|-------------------------|--------------------|
|                        | ⋮                       |                    |
| 94                     | Two sub-floats. . . . . | 43                 |
|                        | 94.1                    | First. . . . . 43  |
|                        | 94.2                    | Second. . . . . 43 |
|                        | ⋮                       |                    |

  

|                                                                                   |                                                                                    |
|-----------------------------------------------------------------------------------|------------------------------------------------------------------------------------|
| 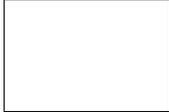 | 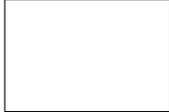 |
| 94.1: First.                                                                      | 94.2: Second.                                                                      |
| <p>Figure 94: Two sub-floats.<br/>See figures 94.1 and 94.2.</p>                  |                                                                                    |

## 5.2 A More Advanced Example

A second example, shown in figure 94, demonstrates how to change the sub-float labels and have the sub-captions printed on the List-of-Figures.

The first `\renewcommand` changes the reference to `\thesubfigure` to return both the figure number and the subfigure number separated with a period. The next two `\renewcommand`'s turn off the `\p@subfigure` (since it is now included in `\thesubfigure` and adds the colon and space to the subfigure label. Also, the `lofdepth` is set to “2” so as to allow the subfigure captions to show when the `\listoffigures` loads the `lof` file. Finally, the `figure` is defined and a little following text is given that refers to it.

```

\renewcommand{\thesubfigure}{\thefigure.\arabic{subfigure}}
\captionsetup[subfigure]{labelformat=simple,labelsep=colon,
                        listofformat=subsimple}
\captionsetup[lofdepth=2]
\makeatletter
\renewcommand{\p@subfigure}{}
\makeatother
⋮
\listoffigures
⋮
\begin{figure}%
\centering
\subfloat[First.]{%
\label{fig:first}%
...figure code...}%
\quad
\subfloat[Second.]{%
\label{fig:second}%
...figure code...}%
\caption{Two sub-floats.}
\end{figure}
⋮
See figures~\ref{fig:first} and \ref{fig:second}.

```

### 5.3 An Example Without Sub-caption Text

The next example, shown in figure 95, demonstrates a commonly required format where the subfigure are just labeled and the description occurs in the main caption. This is easy to do by using the “empty” optional caption arguments “[ ]”. This creates a label for the subfigure in the text, but it does not show on the list-of-figures page. However, by default the caption may not be perfectly centered, so `\subfiglabelskip` is reduced to zero points to ensure that there is not any extra space hidden in the sub-caption. To refer to the subfigure label within the text or the main caption, you can use the `\subref` command, which is similar to the `\ref` command, but does not carry the figure number.

```

\listoffigures
:
\begin{figure}%
  \centering
  \subfloat[] []{%
    \label{fig:ex3-a}%
    ...figure code...}%
  \hspace{8pt}%
  \subfloat[] []{%
    \label{fig:ex3-b}%
    ...figure code...}\
  \subfloat[] []{%
    \label{fig:ex3-c}%
    ...figure code...}%
  \hspace{8pt}%
  \subfloat[] []{%
    \label{fig:ex3-d}%
    ...figure code...}%
  \caption[A set of four sub-floats.]{A set of four sub-floats:
    \subref{fig:ex3-a} describes the first sub-float;
    \subref{fig:ex3-b} describes the second sub-float;
    \subref{fig:ex3-c} describes the third sub-float; and,
    \subref{fig:ex3-d} describes the last sub-float.}%
  \label{fig:ex3}%
\end{figure}
:
The text references the main figure as figure~\ref{fig:ex3}
or part of it as
figures~\subref*{fig:ex3-a}--\subref{fig:ex3-c}.

```

### 5.4 Another Example

I was asked if it was possible to center a smaller subfigure next to a larger one while keeping the sub-captions lined up. The answer is yes. The older way, shown here, is to vertically center the smaller subfigure in a `\vbox` the same height as the larger subfigure. To make it more interesting, we will also assume that we are not sure what the height of the larger subfigure will be.

First we place the larger subfigure in a “savebox” and then use the height of the “savebox” to build the `\vbox` to contain the smaller subfigure. The result is shown in figure 96.

```

\newsavebox{\tempbox}
:

```

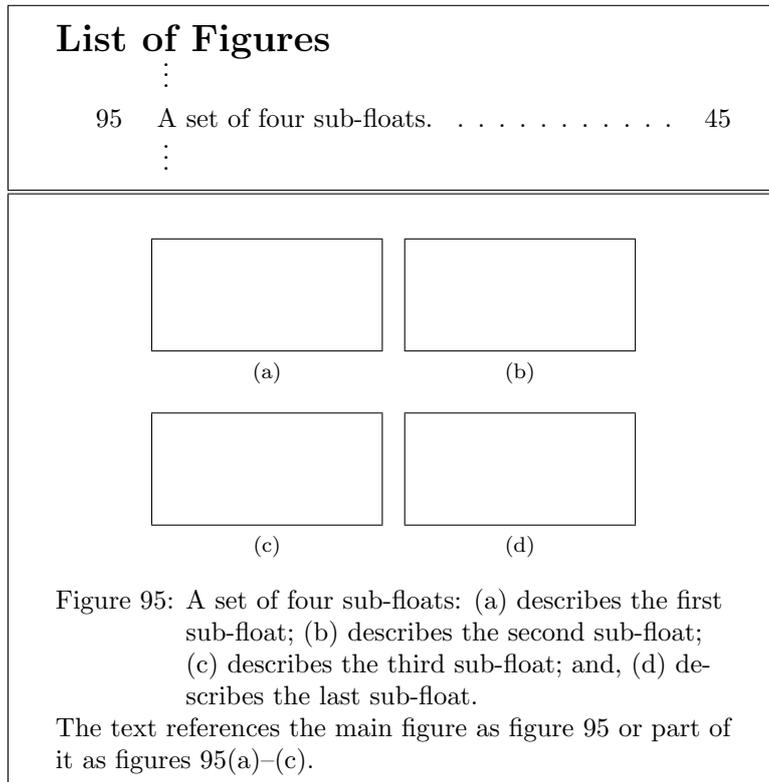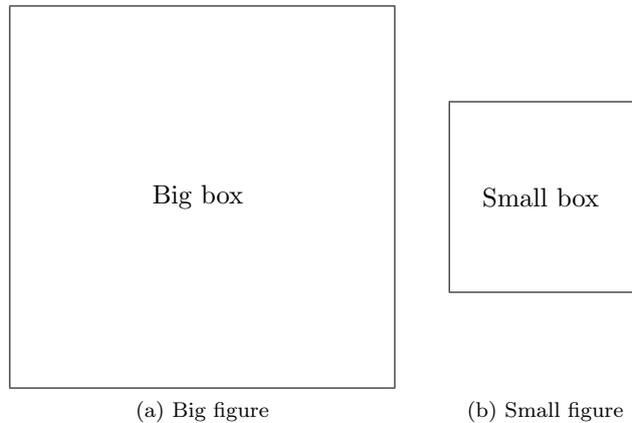

Figure 96: Two more sub-floats.

```

\begin{figure}%
  \centering
  \sbox{\tempbox}{...figure code...}%
  \subfloat[Big figure]{\usebox{\tempbox}}%
  \quad
  \subfloat[Small figure]{%
    \vbox to \ht\tempbox{%
      \vfil
      ...figure code...
      \vfil}}%
  \caption{Two more sub-floats.}

```

```

\label{fig:vertcenter}
\end{figure}

```

The floatrow package will automatically check the heights and widths of your figures and captions and can align your subfigures pretty much any way that you want. For more information, see the subfig package documentation [2].

## 6 Frequently Asked Questions (FAQs)

The ten most frequently asked questions about the subfig package are:

### 6.1 “My sub-floats are not aligned along their bottoms. Why?”

Remember! The subfig package aligns sub-floats along their baselines with the sub-caption (if any) sticking out above or below. The above problem is usually due to using a minipage, tabular or array environment that, by default, places the baseline at the center of the box that it generates. If the two sub-floats are different sizes, or if one sub-float is generated in some other way with its baseline not at the expected place (perhaps an \includegraphics), then the sub-float will be misaligned. One solution is to use the environment options ‘[t]’ or ‘[b]’ to move the baseline to the top or bottom rather than the center.

### 6.2 “How can I get my floats/sub-floats to line up the way I want?”

A similar question, but this one is caused by extra whitespace in the source text generating spaces next to the floats, and \par’s generated by blank lines. The main thing is *be aware* that extra whitespace can move floats and sub-floats around, sometimes a lot and sometimes just a little so that they look “wrong”. Placing too many ‘%’s at the end of the lines is better than too few in the various float environments. (See the discussion of “white space” in section 5.)

### 6.3 “I have too many sub-floats for one page, How can I spread them over two or more pages and continue the numbering?”

The \ContinuedFloat command makes creating continued floating environments easy. See the discussion in section 2.2.3.

### 6.4 “Why do I get a garbled caption or an error when I use square brackets?”

```

\subfloat[SHIFT: ‘‘register[3] $<=< $ 3;’’]{... float text ...}

```

Since the \subfloat command has an optional argument, delimited with square brackets, before their required argument, you cannot use the ‘]’ character at the top level of either the *<sub-caption>* or *<list-entry>* argument. To overcome this problem, you must wrap all or the portion of the text containing the ‘]’ character, in a pair of curly brackets (see [6, § C.1.1] for more detail). For example:

```

\subfloat[SHIFT: ‘‘register{[3]} $<=< $ 3;’’]{... float text ...}

```

or

```

\subfloat[{\SHIFT: ‘‘register[3] $<=< $ 3;’’}]{... float text ...}.

```

### 6.5 “How do I make my subcaptions print on the List-of-Floats pages?”

You need to set the depth counter for each type of List-of-Floats page to “2” or greater. You can do this in two ways. The first is by using the standard `\setcounter` command; for instance, if you want to show your subtable captions you will need to set the ‘lotdepth’ counter before the `\listoftables` command:

```
\setcounter{lotdepth}{2}
```

The other way of setting this is to use the package option list or the `\captionsetup` command and **globally** (see section 2.2.5) set the associated counter (again before using the `\listoftables` command), *e.g.*:

```
\captionsetup{lotdepth=2}
```

### 6.6 “I set an option and it had no effect. What is happening?”

Most likely, the option that you set is being overridden. Reread the option scoping in section 2.2.5 and use the following commands to find out if your option is being set and if it is being overridden (here for a subtable):

```
\showcaptionsetup{table}
\showcaptionsetup{subfloat}
\showcaptionsetup{subtable}
```

For instance, if you change the ‘textfont’ at the “table” level and the “subfloat” has another setting for ‘textfont’, then the change will work for table floats, but not for subtables, since the “subfloat” definition will override it. You can either add the ‘textfont’ change to the “subfloat” (which will affect all sub-floats) or to the “subtable” (which will affect all subtables) to override the overridden change.

### 6.7 “How do I make a change in the settings for just a single float?”

If you change the values using the `\captionsetup` command within a float environment, then the old values will be restored after you exit that float environment.

### 6.8 “How do I put text labels on an imported sub-float?”

The easiest way is to use the picture commands with the origin set at the bottom right corner of the imported image (actually at the right side of the image’s baseline, which is usually along the bottom of the image). For example, if the imported image is  $5 \times 5$  inches, then the following code will place the text “Label” in red at its center (**Note:** 5 inches is 360 big points).

```
\usepackage{graphics}
\usepackage{color}
:
\begin{figure}%
:
\subfloat[Labeled picture]{%
\label{fig:labeled-image}%
\includegraphics{...path to image file...}%
\unitlength=1bp%
\put(-180,180){\textcolor{red}{\textbf{Label}}}%
}
```

```

:
\end{figure}
:

```

### 6.9 “I want my sub-floats to be ordered by column rather than by row, how do I do that?”

The following example shows a schematic for laying out six sub-floats in column order. The only problem with this approach is that, if the floats and their respective captions are not the same height, then the sub-floats will not line up across the page.

```

\begin{figure}
  \begin{minipage}{\columnwidth}
  :
  \dots sub-floats (a)--(c) go here.
  :
  \end{minipage}
  \begin{minipage}{\columnwidth}
  :
  \dots sub-floats (e)--(f) go here.
  :
  \end{minipage}
  \caption{...}
\end{figure}

```

### 6.10 “How do I put a verbatim environment in a sub-float?”

See section 4.4.

## 7 The Code

### 7.1 Identification

Check L<sup>A</sup>T<sub>E</sub>X release and announce the subfig package.

```
68 \NeedsTeXFormat{LaTeX2e}[1995/06/01]
69 \ProvidesPackage{subfig}[2005/06/28 ver: 1.3 subfig package]
```

### 7.2 Check for Nasty Classes

`\sf@floatfix` Some “broken” document classes use `\let` on `\end@figure` and similar, which are used as hooks in the end-processing of, in this case, figures. The following code, courtesy of David Kastrup (dakgnu.org) fixes the problem and prints a warning.

```
70 \def\sf@floatfix#1#2{%
71   \ifx#1#2%
72     \ifx#1\undefined\else
73       \PackageWarningNoLine{subfig}{%
74 Your document class has a bad definition^^J
75 of \string#1, most likely^^J
76 \string\let\string#1=\string#2^^J
77 which has now been changed to^^J
78 \string\def\string#1{\string#2}^^J
79 because otherwise subsequent changes to \string#2^^J
80 (like done by several packages changing float behaviour)^^J
81 can't take effect on \string#1.^^J
82 Please complain to your document class author}%
83   \def#1{#2}%
84   \fi
85 \fi}

86 \begingroup
87 \def\next#1#2{%
88   \endgroup
89   \sf@floatfix\endfigure\end@float
90   \sf@floatfix\endtable\end@float
91   \sf@floatfix#1\end@dblfloat
92   \sf@floatfix#2\end@dblfloat}
93 \expandafter\next\csname endfigure*\expandafter\endcsname
94 \csname endtable*\endcsname
```

### 7.3 Load The Caption Package

This version of the subfig package is dependent on the new caption package by Axel Sommerfeldt [1]. The caption and the subfig (formerly subfigure) packages were rewritten in order to both improve the processing and to reduce the amount of redundant code.

#### 7.3.1 Load The Keyval Package and Scan Options

The user may want to load the caption package without affecting the caption setup from the class or other packages. In this case, the user can either separately load the caption package with the ‘caption=false’ option or the user may directly invoke the subfig package with this option. Here we check for the latter possibility by scanning the options passed to this package and determine the final setting (if any) of this particular option.

```
95 \RequirePackage{keyval}[1999/03/16]
```

`\sf@ifinlist` Since the caption package is not yet available to us, we need to check for alternate Boolean values ourselves. The `\sf@ifinlist` macro checks a value against a list of synonyms.

```

96 \def\sf@ifinlist#1#2{%
97   \let\next\@secondoftwo
98   \edef\caption@tempa{#1}%
99   \@for\caption@tempb:={#2}\do{%
100     \ifx\caption@tempa\caption@tempb
101       \let\next\@firstoftwo
102     \fi}%
103   \next}

```

`\sf@setbool` The `\sf@setbool` uses `\sf@ifinlist` to check if its second argument is *true* or *false* and set the associated *if* (argument one) accordingly.

```

104 \def\sf@setbool#1#2{%
105   \sf@ifinlist{#2}{1,true,yes,on}{%
106     \@nameuse{#1true}}%
107   }{\sf@ifinlist{#2}{0,false,no,off}}{%
108     \@nameuse{#1false}}%
109   }{%
110     \PackageError{subfig}{Undefined boolean value ‘#2’}{\@ehc}%
111   }}}}

```

`\sf@split` Next, we define a simple version of `\sf@split` here in order to check for the ‘caption’ option. Later, we will redefine it to process the rest of the options. The two new *if*’s are used to keep track of the state of the ‘caption’ option and also if it occurs in the subfig options list.

```

112 \def\sf@split#1=#2=#3\relax{%
113   \KV@sp@def\@tempa{#1}%
114   \ifx\@tempa\@empty
115     \else\ifx\@tempa\KV@caption
116       \sf@usecaptionfoundtrue
117       \ifx\@empty#3\@empty
118         \sf@usecaptiontrue
119       \else
120         \KV@sp@def\@tempb{#2}%
121         \sf@setbool{sf@usecaption}{\@tempb}%
122       \fi
123     \fi\fi}

124 \def\KV@caption{caption}

125 \newif\ifsf@usecaptionfound
126 \sf@usecaptionfoundfalse

127 \newif\ifsf@usecaption
128 \sf@usecaptiontrue

```

Now we get and scan the optionlist for this package and remember if the ‘caption’ option is set.

```

129 \edef\sf@temp{\@optionlist{\@currname.\@current}}
130 \let\caption@tempa\@empty
131 \@for\CurrentOption:=\sf@temp\do{%
132   \expandafter\sf@split\CurrentOption==\relax}

```

### 7.3.2 Load and Extend the Caption Package

First we load the `caption` package if it has not already been loaded using the ‘caption=false’ option if specified. Note that this can cause problems if the `caption` was already loaded with different options, so we issue warnings if the user as loaded the `caption` package and used the ‘caption’ option with the `subfig` packare.

```

133 \ifsf@usecaption

```

```

134 \@ifpackageloaded{caption}{%
135   \ifsf@usecaptionfound
136     \PackageWarning{subfig}{%
137       You cannot set the 'caption' option here if the\MessageBreak
138       caption package is already loaded (the option\MessageBreak
139       'caption=true' is ignored)}%
140   \fi
141 }{%
142   \RequirePackage{caption}[2005/06/26]
143 }%
144 \else
145   \RequirePackage{caption3}[2005/06/11]
146 \fi

```

`\sf@ifpositiontop` Then we make certain that the `\caption@position` is recognizable to the `subfig` package code. We assume that if it is not the same as `\@firstoftwo` (e.g., 'top'), than it must be `\@secondoftwo`, or 'bottom' (i.e., anything that isn't designated as '[position=top]' is forced to be '[position=bottom]').

```

147 \def\sf@ifpositiontop{%
148   \ifx\caption@position\@firstoftwo \let\next\@firstoftwo \else
149   \let\next\@secondoftwo \fi \next}

```

`\DeclareCaptionListOfFormat` Next, we define the `\DeclareCaptionListOfFormat` command which controls how the sub-float captions appear on the List-of-Floats pages. Note that this command can only be used to define new formats in the preamble of your paper. The format may be changed at anytime using the `\captionsetup` command.

```

\caption@setlistofformat
150 \def\DeclareCaptionListOfFormat#1{%
151   \@namedef{caption@lstfmt@#1}##1##2}
152 \@onlypreamble\DeclareCaptionListOfFormat
153 \def\caption@setlistofformat#1{%
154   \@ifundefined{caption@lstfmt@#1}{%
155     \PackageError
156       {subfig}%
157       {Undefined caption list-of format '#1'}%
158       {\caption@eh}%
159   }{%
160     \expandafter\let\expandafter\caption@lstfmt
161     \csname caption@lstfmt@#1\endcsname}}

```

Using the `\DeclareCaptionListOfFormat` command, we define some common formats and the new keyword, 'listofformat', which may be used in the key/value option list of the `\usepackage` command or with the `\captionsetup` command to change the listing format of the sub-float caption label.

```

162 \DeclareCaptionListOfFormat{empty}{}
163 \DeclareCaptionListOfFormat{simple}{#1#2}
164 \DeclareCaptionListOfFormat{parens}{#1(#2)}
165 \DeclareCaptionListOfFormat{subsimple}{#2}
166 \DeclareCaptionListOfFormat{subparens}{(#2)}
167 \DeclareCaptionOption{listofformat}{\caption@setlistofformat{#1}}

```

`\sf@indent` We also add two new keywords, 'listofindent' and 'listofnumwidth', which set the lengths used to show where and how wide the caption label will be when typeset. These are used as the fourth and fifth arguments of the `\dottedxxxline` command, see section 7.5 for more detail.

```

168 \def\sf@indent{3.8em}
169 \define@key{caption}{listofindent}[3.8em]{\def\sf@indent{#1}}

```

```
170 \def\sf@numwidth{2.5em}
171 \define@key{caption}{listofnumwidth}[2.5em]{\def\sf@numwidth{#1}}
```

`\DeclareSubrefFormat` We define the `\DeclareSubreffFormat` command just like the above `\DeclareCaptionListOfFormat`  
`\caption@setsubrefformat` command above. This format, however, controls how the `\subref*` command formats the sub-float label. Again, this command can only be used to define new formats in the preamble of your paper and the format may be changed at anytime using the `\captionsetup` command.

```
172 \def\DeclareSubrefFormat#1{%
173   \@namedef{caption@subreffmt@#1}##1##2##3##4}
174 \@onlypreamble\DeclareSubrefFormat
175 \def\caption@setsubrefformat#1{%
176   \@ifundefined{caption@subreffmt@#1}{%
177     \PackageError
178       {subfig}%
179       {Undefined subref format ‘#1’}%
180       {\caption@eh}%
181   }{%
182     \expandafter\let\expandafter\caption@subreffmt
183       \csname caption@subreffmt@#1\endcsname}}
```

Using the `\DeclareSubrefFormat` command, we define some common formats and the new keyword, ‘subrefformat’, which may be used in the key/value option list of the `\usepackage` command or with the `\captionsetup` command to change the format of the `\subref*` references.

```
184 \DeclareSubrefFormat{empty}{}
185 \DeclareSubrefFormat{simple}{#1#2}
186 \DeclareSubrefFormat{parens}{#1(#2)}
187 \DeclareSubrefFormat{subsimple}{#2}
188 \DeclareSubrefFormat{subparens}{(#2)}
189 \DeclareCaptionOption{subrefformat}{\caption@setsubrefformat{#1}}
```

## 7.4 Options Processing

`\KV@config` In order to work within the caption package, the subfig package saves most of the options  
`\sf@split` provided via `\usepackage` and (re-)applies them each time a sub-float is started. The two  
`\ProcessPackageOptions` exceptions are the ‘caption’ keyword, which is ignored (see section 7.3.1 above), and the ‘config’ keyword, which is executed immediately. To accomplish this, we use a modified version of the keyval package processing. ‘Config’ entries are detected and executed, while other keywords are passed back to add to the “subfloat” list. (**Note:** Currently the ‘config’ files are unable to use `\captionsetup` without its optional argument. If you need to set a global value in a configuration file, than do it directly.)

```
190 \newcounter{KVtest}
191 \def\KV@config{config}
192 \def\sf@split#1=#2=#3\relax{%
193   \setcounter{KVtest}{1}%
194   \KV@@sp@def\@tempa{#1}%
195   \ifx\@tempa\@empty
196   \else\ifx\@tempa\KV@caption
197     \setcounter{KVtest}{2}%
198   \else\ifx\@tempa\KV@config
199     \setcounter{KVtest}{2}%
200     \expandafter\let\expandafter\@tempc
201       \csname\KV@prefix\@tempa\endcsname
202     \ifx\@tempc\relax
```

```

203     \KV@errx
204     {\@tempa\space undefined}%
205     \else\ifx\@empty#3\@empty
206     \KV@default
207     \else
208     \KV@sp@def\@tempb{#2}%
209     \expandafter\@tempc\expandafter{\@tempb}\relax
210     \fi\fi
211     \fi\fi\fi}

212 \def\ProcessPackageOptions{%
213   \def\KV@prefix{KV@\@currname @}%
214   \let\@tempc\relax
215   \let\caption@tempa\@empty
216   \@for\CurrentOption:=\@classoptionslist\do{%
217     \ifundefined{KV@caption@\CurrentOption}{\do{%
218       \edef\caption@tempa{\caption@tempa,\CurrentOption,}%
219       \expandtwoargs\@removeelement\CurrentOption
220       \@unusedoptionlist\@unusedoptionlist}}%
221     \edef\caption@tempb{\@optionlist{\@currname.\@current}}%
222     \@for\CurrentOption:=\caption@tempb\do{%
223       \expandafter\sf@split\CurrentOption==\relax
224       \ifnum\c@KVtest<2\relax
225         \edef\caption@tempa{\caption@tempa,\CurrentOption,}%
226         \fi}%
227     \edef\caption@tempa{%
228       \noexpand\captionsetup[subfloat]{\caption@tempa}}%
229     \caption@tempa}

```

## 7.5 Generalized List-of-Floats

`\dottedxxxline` This is a generalized wrapper for the `\dottedtocline` command for sub-float entries. It checks for the level based on the output file extension (second argument) and not using only the `\tocdepth`, as the `\dottedtocline` command does. The arguments of the `\dottedxxxline` command are:

1. **Main Float Type Relative to the Sub-float.**
2. **File Extension.** The usual values are: `lof` or `lot`. The internal values `\ext@subfigure` and `\ext@subtable` hold these extensions.
3. **Level.** By default this is ‘2’ for sub-floats. If the level is greater than  $\langle Ext \rangle_{depth}$  (where  $\langle Ext \rangle$  is the second argument, above), then no line is produced.
4. **Indent.** Total indentation from the left margin.
5. **Numwidth.** Width of box for the label number if the `Title` has a `\numberline` command. This is also the amount of extra indentation added to second and later lines of a multiple line entry.
6. **Title.** Contents of entry (e.g., the  $\langle list\_entry \rangle$  or  $\langle sub\_caption \rangle$ ).
7. **Page.** The page number of the figure or table.

The final two arguments, `title` and `page`, are automatically appended to the value of `\l@subfigure` (and symmetrically for other sub-float types).

```

230 \def\dottedxxxline#1#2#3#4#5#6#7{%
231   \begingroup
232   \ifundefined{caption@setfloastype}%
233     \caption@settype
234     \caption@setfloastype
235     {#1}
236   \caption@settype{subfloat}%
237   \caption@settype{sub#1}%

```

```

238 \ifnum #3>\@nameuse{c@#2depth}\else
239 \dottedtocline{\z@}{#4}{#5}{#6}{#7}%
240 \fi
241 \endgroup}

```

## 7.6 Create New Sub-floats

`\newsfloat` This command is used to create new types of sub-floats. It is used during the subfig configuration to create the two standard float types: “subfigure” and “subtable” and may be used anywhere in the preamble to create other types of sub-floats (see section 4.2 and table 1).

```

242 \newif\ifmaincaptiontop
243 \def\newsfloat{%
244 \ifnextchar[ %] bracket matching
245 {\@newsfloat}
246 {\@newsfloat []}}

247 \def\@newsfloat[#1]#2{%
248 \ifundefined{c@sub#2}{%
249 \newcounter{sub#2}[#2]
250 \newcounter{sub#2@save}%
251 \@namedef{sub#2name}{}%
252 \@namedef{p@sub#2}{\@nameuse{the#2}}%
253 \@namedef{thesub#2}{\alph{sub#2}}%
254 \@namedef{ext@sub#2}{\@nameuse{ext@#2}}%

255 \@namedef{l@sub#2}{%
256 \dottedxxline{#2}%
257 {\@nameuse{ext@sub#2}}{2}{\sf@indent}{\sf@numwidth}}%
258 \ifundefined{c@\@nameuse{ext@#2}depth}{%
259 \expandafter\newcounter\expandafter{\@nameuse{ext@#2}depth}%
260 \expandafter\addtocounter\expandafter{\@nameuse{ext@#2}depth}\@ne}{%
261 \@namedef{KV@caption@\@nameuse{ext@#2}depth@default\expandafter}%
262 \expandafter{\csname KV@caption@\@nameuse{ext@#2}depth\endcsname{2}}%
263 \@namedef{KV@caption@\@nameuse{ext@#2}depth}##1{%
264 \setcounter{\@nameuse{ext@#2}depth}{##1}}%
265 \edef\sfc@counterlist{%
266 \ifundefined{sfc@counterlist}{}%
267 {\sfc@counterlist,}sub#2}%
268 \captionsetup[sub#2]{#1}%
269 }{%
270 \PackageWarning{subfig}{%
271 The sub#2\space type is already defined.}%
272 }}

273 \@onlypreamble\@newsfloat
274 \@onlypreamble\newsfloat

```

## 7.7 Layout Parameters

`\sf@farskip` We now create the sub-float layout parameters. We do it now so that the values will be available during the configuration and options processing, below. The ‘margin’ and `\sf@captopadj` ‘width’ are already defined in the caption package.

```

\sf@farskip
\sf@captopadj
\sf@capskip
\sf@nearskip
275 \newskip\sf@farskip
276 \sf@farskip 10\p@
277 \define@key{caption}{farskip}[10\p@]{\sf@farskip=#1}

278 \newdimen\sf@captopadj
279 \sf@captopadj \z@
280 \define@key{caption}{topadj}{\z@}{\sf@captopadj=#1}

```

```

281 \newskip\sf@capskip
282 \sf@capskip 4\p@
283 \define@key{caption}{caption}[4\p@]{\sf@capskip=#1}

284 \newskip\sf@nearskip
285 \sf@nearskip \z@
286 \define@key{caption}{nearskip}[5\p@]{\sf@nearskip=#1}

```

`\sf@old@caption` Save the current definition of the `\@caption` command so that we can wrap it with code that first checks if a caption for the current float type comes before (`'[position=top]'`) or after (`'[position=bottom]'`) the related sub-floats. Then the decision can be made of whether or not to flush the list of sub-float captions to the proper List-of-Floats file. See the `\caption@` definition in section 7.11.

```

287 \let\sf@old@caption\@caption
288 \def\@caption{\caption@}

```

## 7.8 Process the Package Options

1. Set the default (override) values in “subfloat”. (It would be nice not to set anything, however, most users will want something like this set so we do so. If desired, these may be wiped out in a configuration file with `\clearcaptionsetup` command.)

```

289 \captionsetup[subfloat]{%
290     font=footnotesize,
291     labelformat=parens,labelsep=space,
292     listofformat=subparens,subrefformat=subsimple}

```

2. Load the configuration file(s) if ‘config’ keyword is given. (Use `\captionsetup` to change options (remember, due to a known bug, you cannot set global-level values because you have to supply the optional argument in a subfig package configuration file.)

```

293 \define@key{subfig}{config}[subfig]{%
294     \InputIfFileExists{#1.cfg}{%
295         \typeout{*****^^J%
296             * Subfig configuration file #1.cfg used ^^J%
297             *****}%
298     }{%
299         \PackageWarning{subfig}{Configuration file #1.cfg not found}}%
300 }

```

3. Process the options list using the KV macros. (Note, the ‘config’ option is processed before any other option in the package list to load the files in the last step, above.) The remaining options are added to the end of “subfloat” after the configuration process.

```

301 \ProcessPackageOptions

```

4. If the ‘subfigure’ and the ‘subtable’ sub-floats have not been defined during the configuration process, than we define define them now (along with all of the items in table 1).

```

302 \@ifundefined{c@subfigure}{\newsfloat{figure}}{}
303 \@ifundefined{c@subtable}{\newsfloat{table}}{}

```

5. Finally, we designate those commands that we will not need after this package is finished. Also, we reset `\CaptionOption` to keep this package from influencing other packages using the variable.

```

304   \AtEndOfPackage{%
305     \global\let\ifsf@usecaption\relax
306     \global\let\sf@usecaptiontrue\relax
307     \global\let\sf@usecaptionfalse\relax
308     \global\let\ifsf@usecaptionfound\relax
309     \global\let\sf@usecaptionfoundtrue\relax
310     \global\let\sf@usecaptionfoundfalse\relax
311     \global\let\KV@caption\relax
312     \global\let\KV@subfig@caption\relax
313     \global\let\KV@subfig@caption@default\relax
314     \global\let\KV@config\relax
315     \global\let\KV@subfig@config\relax
316     \global\let\KV@subfig@config@default\relax
317     \global\let\ProcessPackageOptions\relax
318     \global\let\@unprocessedoptions\relax
319     \let\CurrentOption\@empty
320   }

```

6. (And, of course, we process calls to `\captionsetup` throughout the paper.)

## 7.9 Define the Sub-float Layout

The main command is `\subfloat`. This command takes the figure code and the optional caption and builds a vertical box that contains them along with some additional padding as defined by the layout parameters defined in section 7.7

`\sf@top` We define two skip variables which are set to the ‘farskip’ and the ‘nearskip’ values, depending on the ‘position’ of the corresponding float caption. These are used, when the time comes, to build the sub-float box as illustrated in figure 91.

```

321 \newskip\sf@top
322 \newskip\sf@bottom

```

`\subfloat` This is the “main” command. All it really does is to check that we are inside a float environment (or at the very least that someone has tricked us by defining `\@capttype`). If all seems salubrious, than we pass all of the arguments to the internal comamnd `\sf@subfloat`.

```

323 \def\subfloat{%
324   \ifx\@capttype\@undefined
325     \@latex@error{\noexpand\subfloat outside float}\@ehd
326     \expandafter\@gobble
327   \else
328     \expandafter\@firstofone
329   \fi
330   {\sf@subfloat}}

```

`\sf@subfloat` This routine does more setup and at the end begins to parse the optional argument. First the float options are applied and a flag `\ifmaincaptiontop` is set for later use; the ‘subfloat’ and sub-`\@capttype` options are set and the `\label` command is temporarily wrapped with `\subfloat@label`.

```

331 \def\sf@subfloat{%
332   \begingroup
333   \@ifundefined{caption@setfloattype}%
334     \caption@settype
335     \caption@setfloattype
336     \@capttype
337   \sf@ifpositiontop{%
338     \maincaptiontoptrue
339   }{%

```

```

340     \maincaptiontopfalse
341   }%
342   \caption@settype{subfloat}%
343   \caption@settype{sub\@capttype}%
344   \let\sf@oldlabel=\label
345   \let\label=\subfloat@label

```

Next, a decision (based on the `\ifmaincaptiontop` flag) is made of how to advance the float counter; then the sub-float counter is advanced and saved and a check is made if an optional argument is present (if not, one is supplied).

```

346   \ifmaincaptiontop\else
347     \advance\@nameuse{c@\@capttype}\@ne
348   \fi
349   \refstepcounter{sub\@capttype}%
350   \setcounter{sub\@capttype @save}{\value{sub\@capttype}}%
351   \@ifnextchar [% %] match left bracket
352     {\sf@@subfloat}%
353     {\sf@@subfloat[\@empty]}

```

`\sf@@subfloat` A check is made for a second optional argument, if one is not found, than one is supplied. We are now ready to call the real (internal) “`\subfloat`” command, `\sf@@@subfloat`.

```

354 \long\def\sf@@subfloat[#1]{%
355   \@ifnextchar [% %] match left bracket
356     {\sf@@@subfloat{sub\@capttype}[\@empty]{#1}}%
357     {\sf@@@subfloat{sub\@capttype}[\@empty]{#1}[\@empty]{#1}}

```

`\sf@@@subfloat` This is the main function in the whole package. It is the one that builds the sub-float box and stuffs it with the various parts from its arguments and the currently set options.

```

358 \long\def\sf@@@subfloat#1[#2][#3]#4{%

```

The next two lines are the first section of a hook for the `floatrow` package to obtain and save the height of the highest subfloat on the current row.

```

359   \@ifundefined{FBsc@max}{}%
360   {\FB@readaux{\let\FBsuboheight\relax}}%

```

The next section sets a counter, `\@tempcnta`, depending on the current interpreter mode. Zero indicates the start of a minipage; One is the normal; and, Two indicates that there was a non-zero skip preceding the sub-float. We save this information for a little later.

```

361   \@tempcnta=\@ne
362   \if@minipage
363     \@tempcnta=\z@
364   \else\ifdim \lastskip=\z@ \else
365     \@tempcnta=\tw@
366   \fi\fi

```

Then, set our `\sf@top` and `\sf@bottom` variables with right amounts, based on the `\ifmaincaptiontop` flag that we set earlier. Then we insure that we are in horizontal mode and process the sub-float body into a box so that we can measure it. `\@tempdim` is set to the width of the sub-float body.

NOTE: We need to either add negative margins or widths here or allow them to stick out!

```

367   \ifmaincaptiontop
368     \sf@top=\sf@nearskip
369     \sf@bottom=\sf@farskip
370   \else
371     \sf@top=\sf@farskip
372     \sf@bottom=\sf@nearskip

```

```

373 \fi
374 \leavevmode
375 \setbox\@tempboxa \hbox{#4}%
376 \@tempdima=\wd\@tempboxa

```

The next seven lines are the second section of the floatrow package hook which counts the maximal height of subfloat row.

```

377 \@ifundefined{FBsc@max}{%
378   {\global\advance\Xhsize-\wd\@tempboxa
379   \dimen@=\ht\@tempboxa
380   \advance\dimen@\dp\@tempboxa
381   \ifdim\dimen@>FBso@max
382     \global\FBso@max\dimen@
383   \fi}%

```

Now, we begin building our sub-float box. It will be a vertical box containing two vertical boxes. The baseline of the upper box is used as the baseline of the final sub-float. So this section decides what order to fill-in the box. Figure 91 shows the different ways that we can do this.

The first thing is to decide what skip to add to the top. Depending on the initial mode (stored in \@tempcnta) we may put nothing (and declare \@minipagefalse); the full \sf@top skip; or, the larger of the last skip and \sf@top.

(**Note:** If the ‘debug’ option is used in stripping this code to a package file, than a vertical rule instead of a skip is inserted into the box.)

```

384 \vtop\bgroup
385 \vbox\bgroup
386 \ifcase\@tempcnta
387   \@minipagefalse
388 \or
389 (+debug) \leaders\vrule\vskip\sf@top
390 (-debug) \vskip\sf@top
391 \or
392 \ifdim \lastskip=\z@ \else
393   \@tempskipb\sf@top\relax\@xaddvskip
394 \fi
395 \fi

```

Into the top box, after the initial skip (if any), we place either the sub-float body or the sub-caption. We decide which one based on the current ‘position’ setting. Finally, reset the float counter if we changed it above.

(**Note:** Here also, vertical rules are inserted into the box instead of a skip, if the ‘debug’ option is used in stripping this code to a package file.)

```

396 \sf@ifpositiontop{%
397   \ifx \@empty#3\relax \else
398     \sf@subcaption{#1}{#2}{#3}%
399 (+debug) \leaders\vrule width.8pt\vskip\sf@capskip
400 (-debug) \vskip\sf@capskip
401 (+debug) \leaders\vrule width1.2pt\vskip\sf@captopadj
402 (-debug) \vskip\sf@captopadj
403 \fi\egroup
404 \hrule width0pt height0pt depth0pt
405 \box\@tempboxa
406 }{%

```

The next seven lines contain the third section of the floatrow hook which applies a given height to the subfloat figure section.

```

407 \@ifundefined{FBsc@max}%
408   {\box\@tempboxa}%
409   {\ifx\FBsuboheight\relax

```

```

410         \box\@tempboxa
411     \else
412         \vbox to \FBsuboheight{\FBafil\box\@tempboxa\FBbfil}%
413     \fi}%
414     \egroup
415     \ifx \@empty#3\relax \else
416 (+debug)         \leaders\vrule width.8pt\vskip\sf@capskip
417 (-debug)         \vskip\sf@capskip
418                 \hrule width0pt height0pt depth0pt
419                 \sf@subcaption{#1}{#2}{#3}%
420     \fi
421 }%
422 (+debug)         \leaders\vrule\vskip\sf@bottom
423 (-debug)         \vskip\sf@bottom
424     \egroup

```

The next five lines contain the fourth section of the floatrow and the last in this macro. These add, if necessary, a separator for the subfloats.

```

425     \@ifundefined{FBsc@max}{}%
426     {\addtocounter{FRobj}{-1}%
427     \ifnum\c@FRobj=0\else
428         \subfloatrowsep
429     \fi}%
430     \ifmaincaptiontop\else
431         \global\advance\@nameuse{c@\@capytype}\m@ne
432     \fi
433     \endgroup\ignorespaces}

```

## 7.10 Use the **Caption** Package to Build the Sub-float Captions

`\sf@updatecaptionlist` This macro is used to setup the hyperref name, in case it is needed.

```

434 \def\sf@updatecaptionlist#1#2#3#4{%
435     \xdef\sf@captionlist{%
436         \sf@captionlist,%
437         {\protect\numberline{\@subcaplabel}\noexpand{\ignorespaces #2}}%
438         {#1.#3.#4}}

```

`\sf@subcaption` This command is called from within `\sf@@@subfloat` and does two things. First it adds the sub-caption to the list of sub-captions for printing later, after the main caption is printed, which is either before the next caption or at the end of the current float environment.

```

439 \long\def\sf@subcaption#1#2#3{%
440     \ifx \relax#2\relax \else
441         \bgroup
442         \let\label=\@gobble
443         \let\protect=\string
444         \def\@subcaplabel{%
445             \caption@lstfmt{\@nameuse{p@#1}}{\@nameuse{the#1}}}%
446         \sf@updatecaptionlist{#1}{#2}{\the\value{\@capytype}}{\the\value{#1}}%
447     \egroup
448     \fi

```

Next, it makes a box to hold and center the sub-caption and calls the `caption` package `\caption@make` command to format it. (NOTE: This last section of `\sf@subcaption` is closely combined with the `floatrow` package hooks.)

```

449     \bgroup
450     \ifx \relax#3\relax
451         \let\captionlabelsep=\relax
452     \fi

```

This next group of code finishes the `floatrow` package hooks into `subfig`. This gets and saves the maximum height/depth of the caption portion of the subfloats on this row and, optionally, sets the height/depth of the current subcaption.

The first section builds the box and if the marker `\FBsc@max` is not present, than it sets the box. Otherwise the `floatrow` code is activated.

```

453   \setbox0\vbox{%
454     \hb@xt@\the\@tempdima{%
455       \hss
456       \parbox[t]{\the\@tempdima}{%
457         \caption@make
458           {\@nameuse{sub\@capttype name}}}%
459         {\@nameuse{thesub\@capttype}}}%
460         {#3}}%
461       \hss}}%
462   \@ifundefined{FBsc@max}%
463     {\box0}%
464     {\dimen@ht0%
465      \advance\dimen@\dp0%
466      \ifdim\dimen@>\FBsc@max
467        \global\FBsc@max\dimen@
468        \fi
469      \FB@readaux{\let\FBsubcheight\relax}%
470      \ifx\FBsubcheight\relax
471        \def\next{\parbox[t]{\the\@tempdima}}%
472      \else
473        \def\next{\parbox[t][\FBsubcheight][t]{\the\@tempdima}}%
474      \fi
475      \vbox{%
476        \hb@xt@\the\@tempdima{%
477          \hss
478          \next{%
479            \caption@make
480              {\@nameuse{sub\@capttype name}}}%
481            {\@nameuse{thesub\@capttype}}}%
482            {#3}}%
483          \hss}}}%
484   \egroup}

```

## 7.11 Subfig Caption Processing for the List-of-Floats Files

`\listsubcaptions` The `\listsubcaptions` command writes the list of sub-captions to the List-of-Floats file. This is done so that they will follow the associated caption in the file. The `\listsubcaptions` command is (optionally) called by the `\caption` command and at the end of the float environment by the internal `\end@float` command. In rare instances the user may need to call it also, see section 2.2.4 for an example.

The starred form of the command, `\listsubcaptions*`, is not documented as it is not clear that it is of any real use. It may go away in the future, so it should not be used.

```

485 \def\listsubcaptions{%
486   \@ifstar
487     {\gdef\sfcaptionlist{}}%
488     {\@listsubcaptions{\@capttype}}

```

`\sfcaptionlist` `\sfcaptionlist` is the internal list of pending sub-captions. We initialize it here as an empty list.

```

489 \def\sfcaptionlist{}

```

`\@listsubcaptions` This is the code that actually writes the sub-captions to the appropriate List-of-Floats file. First, we check that `\@capttype` is defined and that the current type of sub-float expects to be written to a List-of-Floats file (by virtue of the file extension contained in `\ext@sub-<whatever>`).

Next we step through the internal list of pending sub-captions and write the contents line to the List-of-Floats file for each. Finally, the internal list, `\sf@captionlist`, is re-initialized.

```

490 \def\@listsubcaptions#1{%
491   \@ifundefined{capttype}{}{%
492     \@ifundefined{ext@sub#1}{}{%
493       \@for \sf@temp:=\sf@captionlist \do {%
494         \ifx \@empty\sf@temp\relax \else
495           \begingroup
496             \def\@currenthref{\expandafter\@secondoftwo\sf@temp}%
497             \sf@addcontentsline
498               {\@nameuse{ext@sub#1}}%
499               {sub#1}%
500               {\expandafter\@firstoftwo\sf@temp}%
501           \endgroup
502         \fi}}%
503   \gdef\sf@captionlist{}}

```

`\caption@` This last is a wrapper for the standard `\caption` command. It is called by the main float `\caption` command and makes sure that the `\@listsubcaptions` is called at the proper time to either add the pending sub-captions for the last caption (if the float caption appears *before* the corresponding sub-captions); or, to first write the float caption and then the pending sub-captions (if the float caption appears *after* the corresponding sub-captions).

It processes the options for the float and then checks the ‘position’ setting in order to determine how this float caption is supposed to be used.

```

504 \long\def\caption@#1[#2]#3{%
505   \@ifundefined{caption@setfloattype}%
506     \caption@settype
507     \caption@setfloattype
508     \@capttype
509   \sf@ifpositiontop{%
510     \@listsubcaptions{#1}%
511     \sf@old@caption{#1}[#2][#3]%
512   }{%
513     \sf@old@caption{#1}[#2][#3]%
514     \@listsubcaptions{#1}%
515   }}

```

`\sf@addcontentsline` Some packages may modify `\addcontentsline` which is used by `\@listsubcaptions` to write the sub-captions to the List-of-Float files, therefore we wait until the document begins and grab the then-current definition for use by the `\@listsubcaptions` command.

```

516 \AtBeginDocument{%
517   \let\sf@addcontentsline=\addcontentsline}

```

## 7.12 Sub-float Label Handling

The label handling has three aspects. The first is that the label for a sub-float is defined as the `\p@<sub-float type>` value prepended to the `\the<sub-float type>` value. Secondly, the `\subref` command is similar, except that it shows label as formatted on the List-of-Floats page. Finally, we need to check for the `hyperref` package and provide the extended reference format if it is present (see also, section 7.15.1).

`\subfloat@label` In the `\sf@subfloat` command, the standard label command, `\label` is stored in `\sf@oldlabel` while the sub-float is being processed and this command, `\subfloat@label` is substituted for it.

This first part checks for the optional argument, which has parentheses rather than square brackets, following the form of the similar command in the `hyperref` package. If there is no optional argument, than we supply one.

```
518 \def\subfloat@label{%
519   \@ifnextchar(%   %) match left parenthesis
520   {\sf@sub@label}
521   {\sf@sub@label(Sub\@capytype\space
522     \@ifundefined{thechapter}{\@nameuse{thechapter}\space}%
523     \@nameuse{p@sub\@capytype}%
524     \@nameuse{thesub\@capytype}.)}}}
```

`\sf@sub@label` The next portion of this process is to define the `\@currentlabelname` if the `hyperref` package is loaded and save it for later; then call `\sf@@sub@label` to finish the job. We know that the `hyperref` package is loaded using the `\ifhyperrefloaded` flag which is defined here and will be set later in section 7.15.1.

```
525 \newif\ifhyperrefloaded
526 \def\sfs@sub@label(#1)#2{%
527   \ifhyperrefloaded
528     \protected@edef\@currentlabelname{%
529       \expandafter\strip@period #1\relax.\relax\@@@}%
530   \fi
531   \sfs@@sub@label{#2}}
```

`\sfs@@sub@label` Finally, we get the the value-added portion. First, we call the standard `\label` command (via `\sf@oldlabel`). Then we write the additional information to support the `\subref[*]` command. This will take two forms, depending on the presence of the `hyperref` package. However, in either case, we store the formatted label and the raw sub-float label in the auxillary file.

```
532 \def\sfs@@sub@label#1{%
533   \@bsphack
534   \sf@oldlabel{#1}%
535   \ifhyperrefloaded
536     \begingroup
537     \edef\@currentlabstr{%
538       \expandafter\strip@prefix\meaning\@currentlabelname}%
539     \protected@write\@auxout}{-%
540       \string\newlabel{sub@#1}{-%
541         {\caption@lstfmt
542           {\@nameuse{p@sub\@capytype}}}%
543           {\@nameuse{thesub\@capytype}}}}-%
544       {\caption@subreffmt
545         {\@nameuse{p@sub\@capytype}}}%
546         {\@nameuse{thesub\@capytype}}}%
547         {\the\value{\@capytype}}}%
548         {\the\value{sub\@capytype}}}}-%
549       {\expandafter\strip@period\@currentlabelname\relax.\relax\@@@}%
550       {\@currentHref}}-%
551     {}}}%
552   \endgroup
553   \else
554     \protected@write\@auxout}{-%
555       \string\newlabel{sub@#1}{-%
556         {\caption@lstfmt
557           {\@nameuse{p@sub\@capytype}}}%
558         {\@nameuse{thesub\@capytype}}}}-%
559       {\@currentHref}}-%
560     {}}}%
```

```

558         {\@nameuse{thesub\@capttype}}}%
559     {\caption@subreffmt
560         {\@nameuse{p@sub\@capttype}}}%
561         {\@nameuse{thesub\@capttype}}}%
562         {\the\value{\@capttype}}}%
563         {\the\value{sub\@capttype}}}}}%
564 \fi
565 \@esphack}

```

`\subref` Now, we can define the `\subref[*]` commands. They are just like the `\ref` and `\pageref` commands. The only difference is that they use the alternate information placed in the auxillary file above.

```

\sf@subref
\sf@@subref
566 \def\subref{%
567     \@ifstar
568     \sf@@subref
569     \sf@subref}
570 \def\sf@subref#1{\ref{sub@#1}}
571 \def\sf@@subref#1{\pageref{sub@#1}}

```

### 7.13 Support for Continued Figures

Now we add the ability to have continued floating environments and have them work with the sub-floats without having to load the `captcont` package (but we stay compatible with it if it *is* loaded).

The `caption` package now contains a simple version of the `\ContinuedFloat` command, which works fine for regular floats. We redefine it here to also handle the sub-floats.

```

572 \newif\if@ccflag
573 \ccflagfalse

```

`\ContinuedFloat` We postpone this definition to the end of the preamble, so that we we can check to see if the `captcont` package was loaded. If it was, then we change its internal `\refsteponlycounter` command to work with the new and simpler approach to continuing the floats.

```

574 \AtBeginDocument{%
575     \let\sf@refstepcounter=\refstepcounter
576     \@ifpackageloaded{captcont}{-}{%
577         \def\refsteponlycounter#1{%
578             \if@ccflag
579                 \global\expandafter\advance\csname c@#1\endcsname\@ne
580                 \let\sf@temp\protect
581                 \def\protect{\noexpand\protect\noexpand}%
582                 \edef\@currentlabel{\csname p@#1\endcsname\csname the#1\endcsname}%
583                 \let\protect\sf@temp
584             \else
585                 \sf@refstepcounter{#1}%
586             \fi
587             \ccflagfalse}%
588     }%

```

Next, we re-define the `\ContinuedFloat` command to, in addition to backing up the float counter, check if a sub-float type is defined for this float type. If there is, than it restores the current sub-float counter and to sets the `\if@ccflag` true in order to enable the alternate code in the above `\refsteponlycounter`.

```

589 \def\ContinuedFloat{%
590     \ifx\@capttype\undefined
591         \@latex@error{\noexpand\ContinuedFloat outside float}\@ehd

```

```

592 \else
593   \addtocounter{\@capttype}{\m@ne}%
594   \caption@ContinuedFloat\@capttype
595   \@ifundefined{c@sub\@capttype}{}{%
596     \setcounter{sub\@capttype}{\value{sub\@capttype @save}}%
597     \@ccflagtrue}%
598   \fi}}

```

`\caption@ContinuedFloat` In addition, we provide the `\caption@ContinuedFloat` so that earlier versions of the caption package will not generate an error.

```
599 \providecommand*\caption@ContinuedFloat[1]{}

```

`\sf@caption` Finally, we define a wrapper for the `\caption` command now and wait until the end of the preamble to exchange it for the `\caption` command. Just in case some other package modifies it. It is possible that another package will also wait until the end of the preamble to change the `\caption` command. In that case, it may be necessary to load this package and the other in a specific order. However, this works for now.

```

600 \def\sfcaption{%
601   \let\refstepcounter=\refsteponlycounter
602   \sf@savecaption}
603 \AtBeginDocument{%
604   \let\sfc@savecaption=\caption
605   \let\caption=\sfcaption
606 }

```

## 7.14 Automate the Sub-float Listings

`\sf@end@float` We use the `end@float` and `end@dblfloat` hooks to process the List-of-Floats sub-captions at the end of a float environment so that the page numbers will be correct. The alternative would be for the user to add a `\listsubcaptions` command at the end of the float environment if there is not `\caption` command between the last sub-float and the end of the float environment.

```

607 \let\sfc@end@float=\end@float
608 \let\sfc@end@dblfloat=\end@dblfloat

```

`\end@float` These two wrappers are pretty much the same, they first zero out the sub-float counters (for all sub-float types, but not the saved counter values). Next they dump all of the pending sub-captions the current List-of-Float page. Finally, they call the `\end@float` or `\end@dblfloat` command.

There is one problem, the `fixltx2e` and (old) `fix2col` packages redefine `\end@dblfloat` and assume that the first token in `\end@float` is `\@endfloatbox`. Therefore we redefine `\@endfloatbox` below in section 7.15.3 if these packages are loaded.

```

609 \def\end@float{%
610   \@ifundefined{sf@counterlist}{}{%
611     \@for\sfc@temp:=\sf@counterlist\do{%
612       \setcounter{\sfc@temp}{\z@}}%
613   \@listsubcaptions{\@capttype}}%
614   \sf@end@float}%
615 \def\end@dblfloat{%
616   \@ifundefined{sf@counterlist}{}{%
617     \@for\sfc@temp:=\sf@counterlist\do{%
618       \setcounter{\sfc@temp}{\z@}}%
619   \@listsubcaptions{\@capttype}}%
620   \sf@end@dblfloat}

```

## 7.15 Provide Compatibility with Other Packages

We postpone the following to the end of the preamble in order to detect any other packages that are loaded after this one.

```
621 \AtBeginDocument{%
```

### 7.15.1 The Hyperref Package

We define a `\ifhyperrefloaded` flag which is used with the sub-caption labels (see section 7.12). If the `hyperref` package is loaded, we set this flag to true and, for each sub-float type, we create a `\theH<sub-float>` command that it needs.

```
622 \ifpackageloaded{hyperref}{%
623   \hyperrefloadedtrue
624   %
625   \def\s@setref#1sub#2\relax{%
626     \namedef{theHsub#2\expandafter}{\@nameuse{the#2}.\arabic{sub#2}}%
627     \namedef{toclevel@sub#2}{1}%
628   }
629   %
630   \@for\s@temp:=\s@counterlist\do{%
631     \expandafter\s@setref\s@temp\relax}%
632   %
633   \global\let\s@setref\relax
634   %
635   \let\s@Hrefstepcounter\H@refstepcounter
636   \def\H@refstepcounter#1{%
637     \s@Hrefstepcounter{#1}%
638     \ifundefined{c@sub#1}{-}{%
639       \ifccflag
640         \setcounter{sub#1}{\value{sub#1@save}}%
641       \fi
642       \ccflagfalse}}%
643   %
644 }{}
```

### 7.15.2 The Float Package

If the `float` package is loaded, we need to modify its wrapper for `\@endfloatbox` so that `\listsubcaptions` is called before finishing the float environment in order to get the page numbers right.

```
645 \ifpackageloaded{float}{%
646   \let\s@endfloatbox=\endfloatbox
647   \def\@endfloatbox{%
648     \listsubcaptions
649     \s@endfloatbox}%
650 }{}
```

### 7.15.3 The Fixltx2e Package

We also provide compatibility with the older `fix2col` package that the `fixltx2e` package supersedes. They assume that `\end@float` command begins with `\@endfloatbox` which may be removed with a `\@gobble`; however, we redefine the `\@endfloatbox` making this untrue. Therefore, we have to fix this assumption if one or both of these packages are loaded.

```
651 \ifpackageloaded{fixltx2e}{%
652   \def\end@dblfloat{%
653     \if@twocolumn
```

```

654     \ifundefined{sf@counterlist}{}{%
655         \for\sf@temp:=\sf@counterlist\do{%
656             \setcounter{\sf@temp}{\z@}}%
657         \@listsubcaptions{\@capttype}}%
658     \endfloatbox
659     \ifnum\@floatpenalty <\z@
660         \@largefloatcheck
661         \global\dp\@currbox1sp %
662         \expandafter\@gobble\sf@end@float
663     \fi
664 \else
665     \end@float
666 \fi}%
667 }{%
668 \ifpackageloaded{fix2col}{%
669     \def\end@dblfloat{%
670         \if@twocolumn
671             \@ifundefined{sf@counterlist}{}{%
672                 \for\sf@temp:=\sf@counterlist\do{%
673                     \setcounter{\sf@temp}{\z@}}%
674                 \@listsubcaptions{\@capttype}}%
675             \endfloatbox
676             \ifnum\@floatpenalty <\z@
677                 \@largefloatcheck
678                 \global\dp\@currbox1sp %
679                 \expandafter\@gobble\sf@end@float
680             \fi
681         \else
682             \end@float
683         \fi}}{}%
684 }
685 }
686 \endinput

```

## 8 Acknowledgments

This package was adapted from the `subfigure` package, which was originally written to automatically line up some figure boxes and place labels under them for my Ph.D. dissertation, years ago. I thought it useful and uploaded it to the Internet community and later to CTAN. Many people have asked questions or given comments which collectively have changed and improved the usefulness of that package. In 2002, **Michel Goossens** requested an updated version of the `subfigure` package to feature in the second edition of *The L<sup>A</sup>T<sub>E</sub>X Companion*. In collaboration with **Axel Sommerfeldt** and with many valuable suggestions from **Frank Mittelbach**, this package was developed. It uses the new version of the `caption` package (with which the `subfigure` had a large overlap in function), re-written by **Axel Sommerfeldt** for the same book. This version both simplifies the original package code and, unfortunately, forces it to be backward *in*-compatible with the `subfigure` package, therefore the change in the package name from `subfigure` to `subfig`. Recently, **Olga Lepko** further extended the this package by tightly integrating her extended `floatrow` package.

Beyond those mentioned above a few other people have made important contributions to the development of the prior `subfigure` package and to the present `subfig` package. I want to thank them publicly and they are, alphabetically: **Frederic Darboux**, **Andrew B. Collier**, **Harald Harders**, **David Kastrup**, **William ‘bil’ L. Kleb**, **Heiko Oberdiek**, **Axel Reichert**, and **Peter Wilson**.

## References

- [1] Axel Sommerfeldt, *The caption Package*, Version 3.0g, 2005/06/28. (Available from CTAN as file `/tex-archive/macros/latex/caption.zip`.)
- [2] Olga Lapko, *The floatrow Package*, Version 0.1f, 2005/07/02. (Available from CTAN as file `/tex-archive/macros/latex/floatrow.zip`.)
- [3] Frank Mittelbach and Michel Goossens, with Johannes Braams, David Carlisle and Chris Rowley, *The L<sup>A</sup>T<sub>E</sub>X Companion*, 2<sup>nd</sup> ed., Addison-Wesley, Reading, Massachusetts, 2004.
- [4] David Carlisle, *The keyval Package*, Version 1.13, 1999/03/16. (Available from CTAN as file `/tex-archive/macros/latex/required/graphics.zip`.)
- [5] Keith Reckdahl, *Using Imported Graphics in L<sup>A</sup>T<sub>E</sub>X 2<sub>ε</sub>*, 1997/12/15. (Available from CTAN as file `/tex-archive/info/epslatex.pdf`.)
- [6] Leslie Lamport, *LaTeX User's Guide and Reference Manual*, 2nd edition, Addison-Wesley, Reading, Massachusetts, 1994.
- [7] Donald Ervin Knuth, *The T<sub>E</sub>Xbook*, Addison-Wesley, Reading, Massachusetts, 1986.
