# Supplementary material for: Reentrant phenomenon in the exactly solvable mixed spin-1/2 and spin-1 Ising-Heisenberg model on diamond-like decorated planar lattices
Source: arXiv:0909.4191 source file (2009-09-23)
Supplement: Supplementary file 10 [file test6.tex]

%% test6.tex
%%
%% This is file `test6.tex', one of a set of several test/example files
%% in the `subfig' package.
%%
%% Copyright © 2003, 2004, 2005 Steven Douglas Cochran.
%% 
%% This work (the subfig package) may be distributed and/or modified 
%% under the conditions of the LaTeX Project Public License, either 
%% version 1.3 of this license or (at your option) any later version.
%% The latest version of this license is in
%%   http://www.latex-project.org/lppl.txt
%% and version 1.3 or later is part of all distributions of LaTeX
%% version 2003/12/01 or later.
%%
%% This work has the LPPL maintenance status "author-maintained".
%% 
%% This Current Maintainer of this work is Steven Douglas Cochran.
%%
%% This work consists of all files listed under "MANIFEST" in the
%% README file distributed with the subfig package.

\documentclass{article}

\usepackage{subfig}
\captionsetup[figure]{singlelinecheck=false,format=hang,
                      justification=raggedright,indention=38.5pt}
\captionsetup[subfloat]{singlelinecheck=true,format=default,
                        justification=justified,indention=0pt}

\def\sc{Short caption.}
\def\lc{Non fuit causa cur postularet. Qui hoc intellegi 
        potest? Naevio neque ex societatis ratione neque
        privatim quicquam debuit Quinctius.\par
        Quis huic rei testis est? Idem qui acerrimus 
        adversarius; in hanc rem te, te inquam, testem, 
        Naevi, citabo.\par
        Annum et eo diutius post mortem C. Quincti fuit 
        in Gallia tecum simul Quinctius.}
\makeatletter
  \renewcommand\abstract[1]{%
    \def\@abstract{%
      \centerline{{\large\bf Abstract}}
      \noindent
      #1}}
  \renewcommand\@maketitle{%
    \newpage
    \null\vfil
    \vskip 60\p@
    \begin{center}%
      {\LARGE \@title \par}%
      \vskip 3em%
      {\large
       \lineskip .75em%
       \begin{tabular}[t]{c}%
         \@author
       \end{tabular}\par}%
      \vskip 1.5em%
      {\large \@date \par}% 
    \end{center}%
    \vskip 2.5em%
    \@abstract
    \vfil\null}%
  \newcommand{\figshape}[3][\@empty]{%
    \typeout{#2}%
    \begin{figure}%
      \centering
      \captionsetup[subfigure]{#3}%
      \subfloat[][\sc]{\b}\g\subfloat[][\lc\label{#2b}]{\b}
      \ifx\@empty#1\relax
        \caption{Options [\texttt{#3}].}%
      \else
        \caption[Options [\texttt{#1}{]}]{Options [\texttt{#3}].}%
      \fi
      \label{#2}%
    \end{figure}}
  \newcommand{\figfont}[3]{%
    \captionsetup[subfigure]{#2=#3}%
    \subfloat[{Option [\texttt{#2=#3}]}]%
             [\sc]{\label{#1}\B{#2=#3}}}
  \newcommand{\figfontlist}[3]{%
    \captionsetup[subfigure]{#2={#3}}%
    \subfloat[{Option [\texttt{#2=\{#3\}}]}]%
             [\sc]{\label{#1}\B{#2=\{#3\}}}}
\makeatother

\def\b{\fboxsep=-\fboxrule
       \fbox{\hbox to 2.0in{\vbox to 2mm{\vfil\null}\hfil}}}
\def\B#1{\fboxsep=-\fboxrule
       \fbox{\hbox to 2.0in{\vbox to 6mm{\vfil\hbox to 2.0in{%
             \hfil[\texttt{#1}]\hfil}\vfil}\hfil}}}
\def\g{\hspace{.5in}}

\begin{document}

\title{Subfig Package Test Program Six}
\author{Steven Douglas Cochran\\
        Digital Mapping Laboratory\\
        School of Computer Science\\
        Carnegie-Mellon University\\
        5000 Forbes Avenue\\
        Pittsburgh, PA 15213-3890\\
        USA}
\date{21 December 2003}
\abstract{This test checks the various caption formatting options.}
\maketitle
\clearpage

\tableofcontents
\clearpage

\listoffigures
\clearpage

\makeatletter
  \global\@topnum\z@   % Prevents figures from going at top of page.
\makeatother
\section{Subcaption Shape Options}

There are seven options for setting the subcaption shape or ``format''.
The default setting is produced by
\begin{quote}
  $\backslash$captionsetup[subfigure]\{ style=default, margin=0pt, parskip=0pt, 
  hangindent=0pt, indention=0pt, singlelinecheck=true\}
\end{quote}
which is shown in figure~\ref{fig:shape-01}.
Figure~\ref{fig:shape-00} shows the same thing, but without setting
the ``singlelinecheck'' to centering.  You can see that the
``singlelinecheck'' option only affects the short caption.

Any or all of the other shape option may be used at one time, since
they define orthogonal aspects of the caption shape.  The other
options are:
\begin{itemize}
  \item \texttt{singlelinecheck}, (Boolean) which causes a caption
    that will fit on one line to be centered below the figure
    (actually, to use the singlelinecheck format) .
  \item \texttt{indention}, (amount) which indents the caption text.
  \item \texttt{hangindent}, (amount) which indents the caption text, except
    for the first line of each paragraph.
  \item \texttt{parskip}, (amount) which adds some extra space between 
    separate paragraphs in a caption.
  \item \texttt{format=hang}, which causes the label to hang out to
    the left of the caption text.  \texttt{normal} turns it off.
  \item \texttt{margin}, (amount) which sets extra space to either side of
    the caption.  The option \texttt{width} may also be used.  This sets
    the margins to provide the requested width of the caption.
\end{itemize}
Figures~\ref{fig:shape-00} thru \ref{fig:shape-63} show the different
combinations of these formats.

\def\exin{15pt}    % indention value
\def\exhi{-10pt}    % hangindent value
\def\exps{5pt}     % parskip value
\def\exma{10pt}    % margin value
\figshape{fig:shape-00}{singlelinecheck=false}
\figshape{fig:shape-01}{ }
\figshape{fig:shape-02}{indention=\exin,singlelinecheck=false}
\figshape{fig:shape-03}{indention=\exin}
\figshape{fig:shape-04}{hangindent=\exhi,singlelinecheck=false}
\figshape{fig:shape-05}{hangindent=\exhi}
\figshape[hangindent=\exhi,indention=\exin,
         \hfil\null\string\linebreak\ singlelinecheck=false]%
         {fig:shape-06}%
         {hangindent=\exhi,indention=\exin, singlelinecheck=false}%
\figshape{fig:shape-07}{hangindent=\exhi,indention=\exin}
\figshape{fig:shape-08}{parskip=\exps,singlelinecheck=false}
\figshape{fig:shape-09}{parskip=\exps}
\figshape[parskip=\exps,indention=\exin,
         \hfil\null\string\linebreak\ singlelinecheck=false]%
         {fig:shape-10}%
         {parskip=\exps,indention=\exin, singlelinecheck=false}%
\figshape{fig:shape-11}{parskip=\exps,indention=\exin}
\figshape[parskip=\exps,hangindent=\exhi,
         \hfil\null\string\linebreak\ singlelinecheck=false]%
         {fig:shape-12}%
         {parskip=\exps,hangindent=\exhi, singlelinecheck=false}%
\figshape{fig:shape-13}{parskip=\exps,hangindent=\exhi}
\figshape[parskip=\exps,hangindent=\exhi,indention=\exin,
         \hfil\null\string\linebreak\ singlelinecheck=false]%
         {fig:shape-14}%
         {parskip=\exps,hangindent=\exhi,indention=\exin, 
         singlelinecheck=false}
\figshape{fig:shape-15}{parskip=\exps,hangindent=\exhi,indention=\exin}
\clearpage
\figshape{fig:shape-16}{format=hang,singlelinecheck=false}
\figshape{fig:shape-17}{format=hang}
\figshape[format=hang,indention=\exin,
         \hfil\null\string\linebreak\ singlelinecheck=false]%
         {fig:shape-18}%
         {format=hang,indention=\exin, singlelinecheck=false}%
\figshape{fig:shape-19}{format=hang,indention=\exin}
\figshape[format=hang,hangindent=\exhi,
         \hfil\null\string\linebreak\ singlelinecheck=false]%
         {fig:shape-20}%
         {format=hang,hangindent=\exhi, singlelinecheck=false}%
\figshape{fig:shape-21}{format=hang,hangindent=\exhi}
\figshape[hang,hangindent=\exhi,indention=\exin,
         \hfil\null\string\linebreak\ singlelinecheck=false]%
         {fig:shape-22}%
         {format=hang,hangindent=\exhi,indention=\exin, singlelinecheck=false}
\figshape{fig:shape-23}{format=hang,hangindent=\exhi,indention=\exin}
\figshape{fig:shape-24}{format=hang,parskip=\exps,singlelinecheck=false}
\clearpage
\figshape{fig:shape-25}{format=hang,parskip=\exps}
\figshape[format=hang,parskip=\exps,indention=\exin,
         \hfil\null\string\linebreak\ singlelinecheck=false]%
         {fig:shape-26}%
         {format=hang,parskip=\exps,indention=\exin, singlelinecheck=false}%
\figshape{fig:shape-27}{format=hang,parskip=\exps,indention=\exin}
\figshape[format=hang,parskip=\exps,hangindent=\exhi,
         \hfil\null\string\linebreak\ singlelinecheck=false]%
         {fig:shape-28}%
         {format=hang,parskip=\exps,hangindent=\exhi, singlelinecheck=false}%
\figshape{fig:shape-29}{format=hang,parskip=\exps,hangindent=\exhi}
\figshape[format=hang,parskip=\exps,hangindent=\exhi,
         \hfil\null\string\linebreak\ indention=\exin,singlelinecheck=false]%
         {fig:shape-30}%
         {format=hang,parskip=\exps,hangindent=\exhi,
         indention=\exin,singlelinecheck=false}%
\figshape[format=hang,parskip=\exps,hangindent=\exhi,
         \hfil\null\string\linebreak\ indention=\exin]%
         {fig:shape-31}%
         {format=hang,parskip=\exps,hangindent=\exhi, indention=\exin}
\figshape{fig:shape-32}{margin=\exma,singlelinecheck=false}
\figshape{fig:shape-33}{margin=\exma}
\figshape[margin=\exma,indention=\exin,
         \hfil\null\string\linebreak\ singlelinecheck=false]%
         {fig:shape-34}%
         {margin=\exma,indention=\exin, singlelinecheck=false}
\figshape{fig:shape-35}{margin=\exma,indention=\exin}
\figshape[margin=\exma,hangindent=\exhi,
         \hfil\null\string\linebreak\ singlelinecheck=false]%
         {fig:shape-36}%
         {margin=\exma,hangindent=\exhi, singlelinecheck=false}
\figshape{fig:shape-37}{margin=\exma,hangindent=\exhi}
\figshape[margin=\exma,hangindent=\exhi,indention=\exin,
         \hfil\null\string\linebreak\ singlelinecheck=false]%
         {fig:shape-38}%
         {margin=\exma,hangindent=\exhi,indention=\exin, singlelinecheck=false}
\figshape{fig:shape-39}{margin=\exma,hangindent=\exhi,indention=\exin}
\clearpage
\figshape{fig:shape-40}{margin=\exma,parskip=\exps,singlelinecheck=false}
\figshape{fig:shape-41}{margin=\exma,parskip=\exps}
\figshape[margin=\exma,parskip=\exps,indention=\exin,
         \hfil\null\string\linebreak\ singlelinecheck=false]%
         {fig:shape-42}{margin=\exma,parskip=\exps,indention=\exin, singlelinecheck=false}
\figshape{fig:shape-43}{margin=\exma,parskip=\exps,indention=\exin}
\figshape[margin=\exma,parskip=\exps,hangindent=\exhi,
         \hfil\null\string\linebreak\ singlelinecheck=false]%
         {fig:shape-44}{margin=\exma,parskip=\exps,hangindent=\exhi, singlelinecheck=false}
\figshape{fig:shape-45}{margin=\exma,parskip=\exps,hangindent=\exhi}
\figshape[margin=\exma,parskip=\exps,hangindent=\exhi, 
         \hfil\null\string\linebreak\ indention=\exin,singlelinecheck=false]%
         {fig:shape-46}{margin=\exma,parskip=\exps,hangindent=\exhi, indention=\exin,singlelinecheck=false}
\figshape[margin=\exma,parskip=\exps,hangindent=\exhi,
         \hfil\null\string\linebreak\ indention=\exin]%
         {fig:shape-47}{margin=\exma,parskip=\exps,hangindent=\exhi, indention=\exin}
\figshape{fig:shape-48}{margin=\exma,format=hang,singlelinecheck=false}
\figshape{fig:shape-49}{margin=\exma,format=hang}
\figshape[margin=\exma,format=hang,indention=\exin,
         \hfil\null\string\linebreak\ singlelinecheck=false]%
         {fig:shape-50}%
         {margin=\exma,format=hang,indention=\exin, singlelinecheck=false}
\figshape{fig:shape-51}{margin=\exma,format=hang,indention=\exin}
\figshape[margin=\exma,format=hang,hangindent=\exhi,
         \hfil\null\string\linebreak\ singlelinecheck=false]%
         {fig:shape-52}%
         {margin=\exma,format=hang,hangindent=\exhi, singlelinecheck=false} 
\figshape{fig:shape-53}{margin=\exma,format=hang,hangindent=\exhi}
\figshape[margin=\exma,format=hang,hangindent=\exhi,
         \hfil\null\string\linebreak\ indention=\exin,singlelinecheck=false]%
         {fig:shape-54}%
         {margin=\exma,format=hang,hangindent=\exhi, indention=\exin,singlelinecheck=false}%
\figshape[margin=\exma,format=hang,hangindent=\exhi,
         \hfil\null\string\linebreak\ indention=\exin]%
         {fig:shape-55}%
         {margin=\exma,format=hang,hangindent=\exhi, indention=\exin}
\figshape[margin=\exma,format=hang,parskip=\exps,
         \hfil\null\string\linebreak\ singlelinecheck=false]%
         {fig:shape-56}%
         {margin=\exma,format=hang,parskip=\exps, singlelinecheck=false}
\figshape{fig:shape-57}{margin=\exma,format=hang,parskip=\exps}
\clearpage
\figshape[margin=\exma,format=hang,parskip=\exps,
         \hfil\null\string\linebreak\ indention=\exin,singlelinecheck=false]%
         {fig:shape-58}{margin=\exma,format=hang,parskip=\exps,
         indention=\exin,singlelinecheck=false}
\figshape[margin=\exma,format=hang,parskip=\exps,
         \hfil\null\string\linebreak\ indention=\exin]%
         {fig:shape-59}%
         {margin=\exma,format=hang,parskip=\exps, indention=\exin}
\figshape[margin=\exma,format=hang,parskip=\exps,
         \hfil\null\string\linebreak\ hangindent=\exhi,singlelinecheck=false]%
         {fig:shape-60}{margin=\exma,format=hang,parskip=\exps,
         hangindent=\exhi,singlelinecheck=false}
\figshape[margin=\exma,format=hang,parskip=\exps,
         \hfil\null\string\linebreak\ hangindent=\exhi]%
         {fig:shape-61}%
         {margin=\exma,format=hang,parskip=\exps, hangindent=\exhi}
\figshape[margin=\exma,format=hang,parskip=\exps,
         \hfil\null\string\linebreak\ hangindent=\exhi,indention=\exin,singlelinecheck=false]%
         {fig:shape-62}%
         {margin=\exma,format=hang,parskip=\exps, 
          hangindent=\exhi,indention=\exin,singlelinecheck=false}
\figshape[margin=\exma,format=hang,parskip=\exps,
         \hfil\null\string\linebreak\ hangindent=\exhi,indention=\exin]%
         {fig:shape-63}{margin=\exma,format=hang,parskip=\exps,
         hangindent=\exhi, indention=\exin}
\clearpage

\makeatletter
  \global\@topnum\z@   % Prevents figures from going at top of page.
\makeatother
\section{Subcaption Justification Options}

There are six options for setting the subcaption format, plus another
three if the ``ragged2e'' package is loaded.  The first is
\texttt{justified} which produces the format shows in
figure~\ref{fig:justification-00}.  Only one of these options is
allowed.  If multiple options appear, then only the last is used.  The
Figures~\ref{fig:justification-01} thru \ref{fig:justification-08}
show each of these formats.  The shape options selected along with
each format option is the default (see Figure~\ref{fig:shape-01}),
this shows the effect of the justification option on a single line
caption.

\figshape{fig:justification-00}{justification=justified,singlelinecheck=false}
\figshape{fig:justification-01}{justification=centerfirst,singlelinecheck=false}
\figshape{fig:justification-02}{justification=centerlast,singlelinecheck=false}
\figshape{fig:justification-03}{justification=centering,singlelinecheck=false}
\figshape{fig:justification-04}{justification=Centering,singlelinecheck=false}
\figshape{fig:justification-05}{justification=raggedleft,singlelinecheck=false}
\figshape{fig:justification-06}{justification=RaggedLeft,singlelinecheck=false}
\figshape{fig:justification-07}{justification=raggedright,singlelinecheck=false}
\figshape{fig:justification-08}{justification=RaggedRight,singlelinecheck=false}

\section{Subcaption Font Options}

First we show the size options and then various combinations
of the other font options.  The first subsection, shows the
effect of setting the ``font'' or ``size'' key; the second
subsection shows that of the ``labelfont'' key and the last 
subsection that of the ``textfont'' key.

\subsection{``font'' or ``size'' font Options}

Figures~\ref{fig:f_size-01}--\ref{fig:f_size-06} shows the 
effect of the ``font'' size options and the other font options
are shown in figures~\ref{fig:f_font-01}--\ref{fig:f_font-24}.

\begin{figure}%
  \centering
%
  \figfont{fig:f_size-01}{font}{Large}\g
  \figfont{fig:f_size-02}{font}{large}\\
%
  \figfont{fig:f_size-03}{font}{normalsize}\g
  \figfont{fig:f_size-04}{font}{small}\\
%
  \figfont{fig:f_size-05}{font}{footnotesize}\g
  \figfont{fig:f_size-06}{font}{scriptsize}\\
%
  \caption{Font Size Options.}%
  \label{fig:f_size}%
\end{figure}

\begin{figure}%
  \centering
%
  \figfontlist{fig:f_font-01}{font}{rm,up,md}\g
  \figfontlist{fig:f_font-02}{font}{rm,up,bf}\\
%
  \figfontlist{fig:f_font-03}{font}{rm,it,md}\g
  \figfontlist{fig:f_font-04}{font}{rm,it,bf}\\
%
  \figfontlist{fig:f_font-05}{font}{rm,sl,md}\g
  \figfontlist{fig:f_font-06}{font}{rm,sl,bf}\\
%
  \figfontlist{fig:f_font-07}{font}{rm,sc,md}\g
  \figfontlist{fig:f_font-08}{font}{rm,sc,bf}\\
%
  \figfontlist{fig:f_font-09}{font}{sf,up,md}\g
  \figfontlist{fig:f_font-10}{font}{sf,up,bf}\\
%
  \figfontlist{fig:f_font-11}{font}{sf,it,md}\g
  \figfontlist{fig:f_font-12}{font}{sf,it,bf}\\
%
  \figfontlist{fig:f_font-13}{font}{sf,sl,md}\g
  \figfontlist{fig:f_font-14}{font}{sf,sl,bf}\\
%
  \figfontlist{fig:f_font-15}{font}{sf,sc,md}\g
  \figfontlist{fig:f_font-16}{font}{sf,sc,bf}\\
%
  \figfontlist{fig:f_font-17}{font}{tt,up,md}\g
  \figfontlist{fig:f_font-18}{font}{tt,up,bf}\\
%
  \figfontlist{fig:f_font-19}{font}{tt,it,md}\g
  \figfontlist{fig:f_font-20}{font}{tt,it,bf}\\
%
  \figfontlist{fig:f_font-21}{font}{tt,sl,md}\g
  \figfontlist{fig:f_font-22}{font}{tt,sl,bf}\\
%
  \figfontlist{fig:f_font-23}{font}{tt,sc,md}\g
  \figfontlist{fig:f_font-24}{font}{tt,sc,bf}\\
%
  \caption{Other Font Options.}%
  \label{fig:f_font}%
\end{figure}

\subsection{``labelfont'' font Options.}

Figures~\ref{fig:l_size-01}--\ref{fig:l_size-06} shows the 
effect of the ``font'' size options and the other font options
are shown in figures~\ref{fig:l_font-01}--\ref{fig:l_font-24}.

\begin{figure}%
  \centering
%
  \figfont{fig:l_size-01}{labelfont}{Large}\g
  \figfont{fig:l_size-02}{labelfont}{large}\\
%
  \figfont{fig:l_size-03}{labelfont}{normalsize}\g
  \figfont{fig:l_size-04}{labelfont}{small}\\
%
  \figfont{fig:l_size-05}{labelfont}{footnotesize}\g
  \figfont{fig:l_size-06}{labelfont}{scriptsize}\\
%
  \caption{Labelfont Size Options.}%
  \label{fig:l_size}%
\end{figure}

\begin{figure}%
  \centering
%
  \figfontlist{fig:l_font-01}{labelfont}{rm,up,md}\g
  \figfontlist{fig:l_font-02}{labelfont}{rm,up,bf}\\
%
  \figfontlist{fig:l_font-03}{labelfont}{rm,it,md}\g
  \figfontlist{fig:l_font-04}{labelfont}{rm,it,bf}\\
%
  \figfontlist{fig:l_font-05}{labelfont}{rm,sl,md}\g
  \figfontlist{fig:l_font-06}{labelfont}{rm,sl,bf}\\
%
  \figfontlist{fig:l_font-07}{labelfont}{rm,sc,md}\g
  \figfontlist{fig:l_font-08}{labelfont}{rm,sc,bf}\\
%
  \figfontlist{fig:l_font-09}{labelfont}{sf,up,md}\g
  \figfontlist{fig:l_font-10}{labelfont}{sf,up,bf}\\
%
  \figfontlist{fig:l_font-11}{labelfont}{sf,it,md}\g
  \figfontlist{fig:l_font-12}{labelfont}{sf,it,bf}\\
%
  \figfontlist{fig:l_font-13}{labelfont}{sf,sl,md}\g
  \figfontlist{fig:l_font-14}{labelfont}{sf,sl,bf}\\
%
  \figfontlist{fig:l_font-15}{labelfont}{sf,sc,md}\g
  \figfontlist{fig:l_font-16}{labelfont}{sf,sc,bf}\\
%
  \figfontlist{fig:l_font-17}{labelfont}{tt,up,md}\g
  \figfontlist{fig:l_font-18}{labelfont}{tt,up,bf}\\
%
  \figfontlist{fig:l_font-19}{labelfont}{tt,it,md}\g
  \figfontlist{fig:l_font-20}{labelfont}{tt,it,bf}\\
%
  \figfontlist{fig:l_font-21}{labelfont}{tt,sl,md}\g
  \figfontlist{fig:l_font-22}{labelfont}{tt,sl,bf}\\
%
  \figfontlist{fig:l_font-23}{labelfont}{tt,sc,md}\g
  \figfontlist{fig:l_font-24}{labelfont}{tt,sc,bf}\\
%
  \caption{Other Labelfont Options.}%
  \label{fig:l_font}%
\end{figure}

\subsection{``textfont'' font Options.}

Figures~\ref{fig:t_size-01}--\ref{fig:t_size-06} shows the 
effect of the ``font'' size options and the other font options
are shown in figures~\ref{fig:t_font-01}--\ref{fig:t_font-24}.

\begin{figure}%
  \centering
%
  \figfont{fig:t_size-01}{textfont}{Large}\g
  \figfont{fig:tlsize-02}{textfont}{large}\\
%
  \figfont{fig:t_size-03}{textfont}{normalsize}\g
  \figfont{fig:t_size-04}{textfont}{small}\\
%
  \figfont{fig:t_size-05}{textfont}{footnotesize}\g
  \figfont{fig:t_size-06}{textfont}{scriptsize}\\
%
  \caption{Textfont Size Options.}%
  \label{fig:t_size}%
\end{figure}

\begin{figure}%
  \centering
%
  \figfontlist{fig:t_font-01}{textfont}{rm,up,md}\g
  \figfontlist{fig:t_font-02}{textfont}{rm,up,bf}\\
%
  \figfontlist{fig:t_font-03}{textfont}{rm,it,md}\g
  \figfontlist{fig:t_font-04}{textfont}{rm,it,bf}\\
%
  \figfontlist{fig:t_font-05}{textfont}{rm,sl,md}\g
  \figfontlist{fig:t_font-06}{textfont}{rm,sl,bf}\\
%
  \figfontlist{fig:t_font-07}{textfont}{rm,sc,md}\g
  \figfontlist{fig:t_font-08}{textfont}{rm,sc,bf}\\
%
  \figfontlist{fig:t_font-09}{textfont}{sf,up,md}\g
  \figfontlist{fig:t_font-10}{textfont}{sf,up,bf}\\
%
  \figfontlist{fig:t_font-11}{textfont}{sf,it,md}\g
  \figfontlist{fig:t_font-12}{textfont}{sf,it,bf}\\
%
  \figfontlist{fig:t_font-13}{textfont}{sf,sl,md}\g
  \figfontlist{fig:t_font-14}{textfont}{sf,sl,bf}\\
%
  \figfontlist{fig:t_font-15}{textfont}{sf,sc,md}\g
  \figfontlist{fig:t_font-16}{textfont}{sf,sc,bf}\\
%
  \figfontlist{fig:t_font-17}{textfont}{tt,up,md}\g
  \figfontlist{fig:t_font-18}{textfont}{tt,up,bf}\\
%
  \figfontlist{fig:t_font-19}{textfont}{tt,it,md}\g
  \figfontlist{fig:t_font-20}{textfont}{tt,it,bf}\\
%
  \figfontlist{fig:t_font-21}{textfont}{tt,sl,md}\g
  \figfontlist{fig:t_font-22}{textfont}{tt,sl,bf}\\
%
  \figfontlist{fig:t_font-23}{textfont}{tt,sc,md}\g
  \figfontlist{fig:t_font-24}{textfont}{tt,sc,bf}\\
%
  \caption{Other Textfont Options.}%
  \label{fig:t_font}%
\end{figure}


\end{document}
